# Supplementary material for: Knowledge Enhanced Machine Learning Pipeline against Diverse Adversarial Attacks
Source: arXiv:2106.06235 source file (2022-03-15)
Supplement: Supplementary file 1 [file supplementary.pdf]

---

# Knowledge Enhanced Machine Learning Pipeline against Diverse Adversarial Attacks

---

Nezihe Merve Gürel<sup>1\*</sup> Xiangyu Qi<sup>2\*</sup> Luka Rimanic<sup>1</sup> Ce Zhang<sup>1</sup> Bo Li<sup>3</sup>

## Abstract

Despite the great successes achieved by deep neural networks (DNNs), recent studies show that they are vulnerable against adversarial examples, which aim to mislead DNNs by adding small adversarial perturbations. Several defenses have been proposed against such attacks, while many of them have been adaptively attacked. In this work, we aim to enhance the ML robustness from a different perspective by leveraging *domain knowledge*: We propose a Knowledge Enhanced Machine Learning Pipeline (KEMLP) to integrate domain knowledge (i.e., logic relationships among different predictions) into a probabilistic graphical model via first-order logic rules. In particular, we develop KEMLP by integrating a diverse set of weak auxiliary models based on their logical relationships to the main DNN model that performs the target task. Theoretically, we provide convergence results and prove that, under mild conditions, the prediction of KEMLP is more robust than that of the main DNN model. Empirically, we take road sign recognition as an example and leverage the relationships between road signs and their shapes and contents as domain knowledge. We show that compared with adversarial training and other baselines, KEMLP achieves higher robustness against physical attacks,  $\mathcal{L}_p$  bounded attacks, unforeseen attacks, and natural corruptions under both whitebox and blackbox settings, while still maintaining high clean accuracy.

## 1. Introduction

Recent studies show that machine learning (ML) models are vulnerable to different types of adversarial examples, which are adversarially manipulated inputs aiming to mislead ML models to make arbitrarily incorrect predictions (Szegedy et al., 2013; Goodfellow et al., 2015; Bhattad et al., 2020; Eykholt et al., 2018). Different defense strategies have been proposed against such attacks, including adversarial training (Shafahi et al., 2019; Madry et al., 2017), input processing (Ross and Doshi-Velez, 2018), and approaches with certified robustness against  $\mathcal{L}_p$  bounded attacks (Cohen et al., 2019; Yang et al., 2020a). However, these defenses have either been adaptively attacked again (Carlini and Wagner, 2017a; Athalye et al., 2018) or can only certify the robustness within a small  $\ell_p$  perturbation radius. In addition, when models are trained to be robust against one type of attack, their robustness is typically not preserved against other attacks (Schott et al., 2018; Kang et al., 2019). Thus, despite the rapid recent progress on robust learning, it is still challenging to provide robust ML models against a diverse set of adversarial attacks in practice.

In this paper, we take a different perspective towards training robust ML models against diverse adversarial attacks by integrating *domain knowledge* during prediction, given the observation that human with knowledge is quite resilient against these attacks. We will first take stop sign recognition as a simple example to illustrate the potential role of knowledge in ML prediction. In this example, the **main task** is to predict whether a stop sign appears in the input image. Training a DNN model for this task is known to be vulnerable against a range of adversarial attacks (Eykholt et al., 2018; Xiao et al., 2018a). However, upon such a DNN model, if we could (1) build a detector for a different **auxiliary task**, e.g., detecting whether an octagon appears in the input by using other learning strategies such as traditional computer vision techniques, and (2) integrate the **domain knowledge** such that “A stop sign should be of an octagon shape”, it is possible that additional information could enable the ML system to detect or defend against attacks, which lead to conflicts between the DNN prediction and domain knowledge. For instance, if a speed limit sign with *rectangle* shape is misrecognized as a stop sign, the

---

\*Equal contribution <sup>1</sup>ETH Zurich, Zurich, Switzerland  
<sup>2</sup>Zhejiang University, China (work done during remote internship at UIUC) <sup>3</sup>University of Illinois at Urbana-Champaign, Illinois, USA. Correspondence to: Nezihe Merve Gürel <nezihе.guerel@inf.ethz.ch>, Xiangyu Qi <unispac@zju.edu.cn>, Ce Zhang <ce.zhang@inf.ethz.ch>, Bo Li <lbo@illinois.edu>.

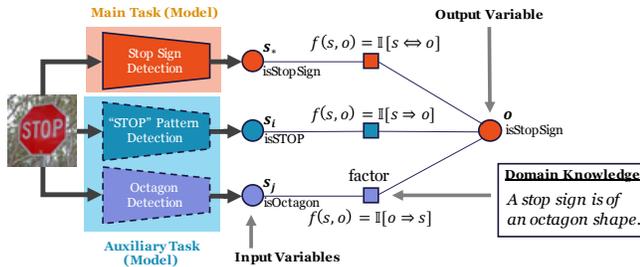

Figure 1. An overview of the KEMLP framework. KEMLP constructs a factor graph by modeling the output of ML models as random input variables, and the KEMLP prediction as a random output variable. It integrates domain knowledge via factors connecting different random variables.

ML system would identify this conflict and try to correct the prediction.

Inspired by this intuition, we aim to understand how to *enhance the robustness of ML models via domain knowledge integration*. Despite the natural intuition in the previous simple example, providing a technically rigorous treatment to this problem is far from trivial, yielding the following questions: How should we integrate domain knowledge in a principled way? When will integrating domain knowledge help with robustness and will there be a tradeoff between robustness and clean accuracy? Can integration of domain knowledge genuinely bring additional robustness benefits against practical attacks when compared with state-of-the-art defenses?

In this work, we propose KEMLP, a framework that facilitates the integration of *domain knowledge* in order to improve the robustness of ML models. Figure 1 illustrates the KEMLP framework. In KEMLP, the outputs of different ML models are modeled as random input variables, whereas the output of KEMLP is modeled as another variable. To integrate domain knowledge, KEMLP introduces corresponding factors connecting these random variables. For example, as illustrated in Figure 1, the knowledge rule “A stop sign is of an octagon shape” introduces a factor between the input variable (i.e., the output of the octagon detector) and the output variable (i.e., output of the stop sign detector) with a factor function that *the former implies the latter*. To make predictions, KEMLP runs statistical inference over the factor graph constructed by integrating all such domain knowledge expressed as first-order logic rules, and output the marginal probability of the output variable.

Based on KEMLP, our main goal is to understand two fundamental questions based on KEMLP: (1) *What type of knowledge is needed to improve the robustness of the joint inference results from KEMLP, and can we prove it?* (2) *Can we show that knowledge integration in the KEMLP framework can provide significant robustness gain over powerful state-of-the-art models?*

We conduct theoretical analysis to understand the first question, focusing on two specific types of knowledge rules:

(1) *permissive knowledge* of the form “ $B \implies A$ ”, and (2) *preventive knowledge* of the form “ $A \implies B$ ”, where  $A$  represents the main task,  $B$  an auxiliary task and  $\implies$  denotes logical implication. We focus on the *weighted robust accuracy*, which is a weighted average of accuracies on benign and adversarial examples, respectively, and we derive sufficient conditions under which KEMLP outperforms the main task model alone. Under mild conditions, we show that integrating multiple weak auxiliary models, both in their robustness and quality, together with the permissive and preventive rules, the weighted robust accuracy of KEMLP can be guaranteed to improve over the single main task model. To our best knowledge, this is the first analysis of proposed form, focusing on the intersection of knowledge integration, joint inference, and robustness.

We then conduct extensive empirical studies to understand the second question. We focus on the road sign classification task and consider the state-of-the-art adversarial training models based on both the  $\mathcal{L}_p$  bounded perturbation and occlusion perturbations (Wu et al., 2019) as our baselines as well as the main task model. We show that by training weak auxiliary models for recognizing the shapes and contents of road signs, together with the corresponding knowledge rules as illustrated in Figure 1, KEMLP achieves significant improvements on their robustness compared with baseline main task models against a *diverse* set of adversarial attacks while maintaining similar or even higher clean accuracy, given its improvement on the tradeoff between clean accuracy and robustness. In particular, we consider existing physical attacks (Eykholt et al., 2018),  $\mathcal{L}_p$  bounded attacks (Madry et al., 2017), unforeseen attacks (Kang et al., 2019), and common corruptions (Hendrycks and Dietterich, 2019), under both whitebox and blackbox settings. To our best knowledge, KEMLP is the first ML model robust to diverse attacks in practice with high clean accuracy. Our code is publicly available for reproducibility<sup>1</sup>.

**Technical Contributions.** In this paper, we take the *first* step towards integrating *domain knowledge* with ML to improve its robustness against different attacks. We make contributions on both theoretical and empirical fronts.

- We propose KEMLP, which integrates a main task ML model with a set of weak auxiliary task models, together with different knowledge rules connecting them.
- Theoretically, we provide the robustness guarantees for KEMLP and prove that under mild conditions, the prediction of KEMLP is more robust than that of a single main task model.
- Empirically, we develop KEMLP based on different main

<sup>1</sup><https://github.com/AI-secure/Knowledge-Enhanced-Machine-Learning-Pipeline>

task models, and evaluate them against a diverse set of attacks, including physical attacks,  $\mathcal{L}_p$  bounded attacks, unforeseen attacks, and common corruptions. We show that the robustness of KEMLP outperforms all baselines by a wide margin, with comparable and often higher clean accuracy.

## 2. Related Work

In the following, we review several bodies of literature that are relevant to the objective of our paper.

**Adversarial examples** are carefully crafted inputs aiming to mislead well-trained ML models (Goodfellow et al., 2015; Szegedy et al., 2013). A variety of approaches to generate such adversarial examples have also been proposed based on different perturbation measurement metrics, including  $\mathcal{L}_p$  bounded, unrestricted, and physical attacks (Wong et al., 2019; Bhattad et al., 2020; Xiao et al., 2018b;c; Eykholt et al., 2018).

**Defense methods** against such attacks have been proposed. Empirically, *adversarial training* (Madry et al., 2017) has shown to be effective, together with feature quantization (Xu et al., 2017) and reconstruction approaches (Samangouei et al., 2018). Certified robustness has also been studied by propagating the interval bound of a NN (Gowal et al., 2018), or randomized smoothing of a given model (Cohen et al., 2019). Several approaches have further improved it: by choosing different smoothing distributions for different  $L_p$  norms (Dvijotham et al., 2020; Zhang et al., 2020; Yang et al., 2020a), or training more robust smoothed classifiers via data augmentation (Cohen et al., 2019), unlabeled data (Carmon et al., 2019), adversarial training (Salman et al., 2019), and regularization (Li et al., 2019; Zhai et al., 2019). While most prior defenses focus on leveraging statistical properties of an ML model to improve its robustness, they can only be robust towards a specific type of attack, such as  $\ell_p$  bounded attacks. This paper aims to explore how to utilize knowledge inference information to improve the robustness of a logically connected ML pipeline against a diverse set of attacks.

**Joint inference** has been studied to take multiple predictions made by different models, together with the relations among them, to make a final prediction (Xu et al., 2020; Deng et al., 2014; Poon and Domingos, 2007; McCallum, 2009; Chen et al., 2014; Chakrabarti et al., 2014; Biba et al., 2011). These approaches usually use different inference models, such as factor graphs (Wainwright and Jordan, 2008), Markov logic networks (Richardson and Domingos, 2006) and Bayesian networks (Neuberg, 2003), as a way to characterize their relationships. The programmatic weak supervision approaches (Ratner et al., 2016; 2017) also perform joint inference by employing labeling functions and

using generative modeling techniques, which aims to create noisy training data. In this paper, we take a different perspective on this problem — we explore the potential of using joint inference with the objective of integrating domain knowledge and to eventually improving the ML robustness. As we will see, by integrating domain knowledge, it is possible to improve the learning robustness by a wide margin.

## 3. KEMLP: Knowledge Enhanced Machine Learning Pipeline

We first present the proposed framework KEMLP, which aims to improve the robustness of an ML model by integrating a diverse set of domain knowledge. In this section, we formally define the KEMLP framework.

We consider a classification problem under a supervised learning setting, defined on a feature space  $\mathcal{X}$  and a finite label space  $\mathcal{Y}$ . We refer to  $x \in \mathcal{X}$  as an input and  $y \in \mathcal{Y}$  as the target variable. An input  $x$  can be a benign example or an adversarial example. To model this, we use  $z \in \{0, 1\}$ , a latent variable that is not exposed to KEMLP. That is,  $x$  is an adversarial example with  $(x, y) \sim \mathcal{D}_a$  whenever  $z = 1$ , and  $(x, y) \sim \mathcal{D}_b$  otherwise, where  $\mathcal{D}_a$  and  $\mathcal{D}_b$  represent the adversarial and benign data distributions. We let  $\pi_{\mathcal{D}_a} = \mathbb{P}(z = 1)$  and  $\pi_{\mathcal{D}_b} = \mathbb{P}(z = 0)$ , implying  $\pi_{\mathcal{D}_a} + \pi_{\mathcal{D}_b} = 1$ . For convenience, we denote  $\mathbb{P}_{\mathcal{D}_a}(x, y) = \mathbb{P}(x, y|z = 1)$  and  $\mathbb{P}_{\mathcal{D}_b}(x, y) = \mathbb{P}(x, y|z = 0)$ . In the following, to ease the exposition, we slightly abuse the notation and use probability densities for discrete distributions.

Given an input  $x$  whose corresponding  $z$  is unknown (benign or adversarial), KEMLP aims to predict the target variable  $y$  by employing a set of *models*. These predictive models are constructed, say, using ML or some other traditional rule-based methods (e.g., edge detector). For simplicity, we describe the KEMLP framework as a binary classification task, in which case  $\mathcal{Y} = \{0, 1\}$ , noting that the multi-class scenario is a simple extension of it. We introduce the KEMLP framework as follows.

**Models** Models are a collection of predictive ML models, each of which takes as input  $x$  and outputs some predictions. In KEMLP, we distinguish three different type of models.

- *Main task model*: We call the (untrusted) ML model whose robustness users want to enhance as the *main task model*, denoting its predictions by  $s_* \in \mathcal{Y}$ .
- *Permissive models*: Let  $s_{\mathcal{I}} = \{s_i : i \in \mathcal{I}\}$  be a set of  $m$  permissive models, each of which corresponds to the prediction of one ML model. Conceptually, permissive models are usually designed for specific events which are *sufficient* for inferring  $y = 1$ :  $s_i \implies y$ .
- *Preventative models*: Similarly, we have  $n$  preventative

models:  $s_{\mathcal{J}} = \{s_j : j \in \mathcal{J}\}$ , each of which corresponds to the prediction of one ML model. Conceptually, preventative models capture the events that are *necessary* for the event  $y = 1$ :  $y = 1 \implies s_j$ .

**Knowledge Integration** Given a data example  $(x, y) \sim \mathcal{D}_b$  or  $(x, y) \sim \mathcal{D}_a$ ,  $y$  is unknown to KEMLP. We create a factor graph to embed the domain knowledge as follows. The outputs of each model over  $x$  become *input variables*:  $s_*, s_{\mathcal{I}} = \{s_i : i \in \mathcal{I}\}, s_{\mathcal{J}} = \{s_j : j \in \mathcal{J}\}$ . KEMLP also has an output variable  $o \in \mathcal{Y}$ , which corresponds to its prediction. Different models introduce different types of factors connecting these variables:

- **Main model:** KEMLP introduces a factor between the main model  $s_*$  and the output variable  $o$  with factor function  $f_*(o, s_*) = \mathbb{1}\{o = s_*\}$ ;
- **Permissive model:** KEMLP introduces a factor between each permissive model  $s_i$  and the output variable  $o$  with factor function  $f_i(o, s_i) = \mathbb{1}\{s_i \implies o\}$ .
- **Preventative model:** KEMLP introduces a factor between each preventative model  $s_j$  and the output variable  $o$  with factor function  $f_j(o, s_j) = \mathbb{1}\{o \implies s_j\}$ .

**Learning with KEMLP** To make a prediction, KEMLP outputs the *probability* of the output variable  $o$ . KEMLP assigns a weight for each model and constructs the following statistical model:

$$\mathbb{P}[o | s_*, s_{\mathcal{I}}, s_{\mathcal{J}}, w_*, w_{\mathcal{I}}, w_{\mathcal{J}}, b_o] \propto \exp\{b_o + w_* f_*(o, s_*)\} \times \exp\left\{\sum_{i \in \mathcal{I}} w_i f_i(o, s_i)\right\} \times \exp\left\{\sum_{j \in \mathcal{J}} w_j f_j(o, s_j)\right\}$$

where  $w_*, w_i, w_j$  are the corresponding weights for models  $s_*, s_i, s_j$ ,  $w_{\mathcal{I}} = \{w_i : i \in \mathcal{I}\}, w_{\mathcal{J}} = \{w_j : j \in \mathcal{J}\}$  and  $b_o$  is some bias parameter that depends on  $o$ . For the simplicity of exposition, we use an equivalent notation by putting all the weights and outputs of factor functions into vectors using an ordering of models. More precisely, we define

$$\mathbf{w} = [1; w_*; (w_i)_{i \in \mathcal{I}}; (w_j)_{j \in \mathcal{J}}],$$

$$\mathbf{f}_o(s_*, s_{\mathcal{I}}, s_{\mathcal{J}}) = [b_o; f_*(o, s_*); (f_i(o, s_i))_{i \in \mathcal{I}}; (f_j(o, s_j))_{j \in \mathcal{J}}],$$

for  $o \in \mathcal{Y}$ . All concatenated vectors from above are in  $\mathbb{R}^{m+n+2}$ . Given this, an equivalent form of KEMLP’s statistical model is

$$\mathbb{P}[o | s_*, s_{\mathcal{I}}, s_{\mathcal{J}}, \mathbf{w}] = \frac{1}{Z_{\mathbf{w}}} \exp(\langle \mathbf{w}, \mathbf{f}_o(s_*, s_{\mathcal{I}}, s_{\mathcal{J}}) \rangle) \quad (1)$$

where  $Z_{\mathbf{w}}$  is the normalization constant over  $o \in \mathcal{Y}$ . With some abuse of notation,  $\mathbf{w}$  is meant to govern all parameters including weights and biases whenever used with probabilities.

**Weight Learning** During the training phase of KEMLP, we choose parameters  $\mathbf{w}$  by performing standard maximum likelihood estimation over a training dataset. Given a particular input instance  $x^{(n)}$ , respective model predictions  $s_*^{(n)}, s_{\mathcal{I}}^{(n)}, s_{\mathcal{J}}^{(n)}$ , and the ground truth label  $y^{(n)}$ , we minimize the negative log-likelihood function in view of

$$\hat{\mathbf{w}} = \arg \min_{\mathbf{w}} \left\{ - \sum_n \log \left( \mathbb{P}[o^{(n)} = y^{(n)} | s_*^{(n)}, s_{\mathcal{I}}^{(n)}, s_{\mathcal{J}}^{(n)}, \mathbf{w}] \right) \right\}.$$

**Inference** During the inference phase of KEMLP, given an input example  $\hat{x}$ , we predict  $\hat{y}$  that has the largest probability given the respective model predictions  $\hat{s}_*, \hat{s}_{\mathcal{I}}, \hat{s}_{\mathcal{J}}$ , namely,  $\hat{y} = \arg \max_{\tilde{y} \in \mathcal{Y}} \mathbb{P}[o = \tilde{y} | \hat{s}_*, \hat{s}_{\mathcal{I}}, \hat{s}_{\mathcal{J}}, \hat{\mathbf{w}}]$ .

## 4. Theoretical Analysis

*How does knowledge integration impact the robustness of KEMLP?* In this section, we provide theoretical analysis about the impact of domain knowledge integration on the robustness of KEMLP. We hope to (1) depict the regime under which knowledge integration can help with robustness; (2) explain how a collection of “weak” (in terms of prediction accuracy) but “robust” auxiliary models, on tasks different from the main one, can be used to boost overall robustness. Here we state the main results, whereas we refer interested readers to Appendix A where we provide all relevant details.

**Weighted Robust Accuracy** Previous theoretical analysis on ML robustness (Javanmard et al., 2020; Xu et al., 2009; Raghunathan et al., 2020) have identified two natural dimensions of model quality: *clean accuracy* and *robust accuracy*, which are the accuracy of a given ML model on inputs  $x$  drawn from either the benign distribution  $\mathcal{D}_b$  or adversarial distribution  $\mathcal{D}_a$ . In this paper, to balance their tradeoff, we use their weighted average as our main metric of interest. That is, given a classifier  $h : \mathcal{X} \rightarrow \mathcal{Y}$  we define its *Weighted Robust Accuracy* as

$$\mathcal{A}_h = \pi_{\mathcal{D}_a} \mathbb{P}_{\mathcal{D}_a}[h(x) = y] + \pi_{\mathcal{D}_b} \mathbb{P}_{\mathcal{D}_b}[h(x) = y].$$

We use  $\mathcal{A}^{\text{KEMLP}}$  and  $\mathcal{A}^{\text{main}}$  to denote the weighted robust accuracies of KEMLP and main task model, respectively.

### 4.1. $\mathcal{A}^{\text{KEMLP}}$ : Weighted Robust Accuracy of KEMLP

The goal of our analysis is to identify the regime under which  $\mathcal{A}^{\text{KEMLP}} > \mathcal{A}^{\text{main}}$  is guaranteed. The main analysis to achieve this hinges on deriving the weighted robust accuracy  $\mathcal{A}^{\text{KEMLP}}$  for KEMLP. We first describe the modeling assumptions of our analysis, and then describe two key characteristics of models, culminating in a lower bound of  $\mathcal{A}^{\text{KEMLP}}$ .

**Modeling Assumptions** We assume that for a fixed  $z$ , that is, for a fixed  $\mathcal{D} \in \{\mathcal{D}_b, \mathcal{D}_a\}$ , the models make independent

errors given the target variable. Thus, for all  $\mathcal{D} \in \{\mathcal{D}_b, \mathcal{D}_a\}$ , the class conditional distribution can be decomposed as

$$\mathbb{P}_{\mathcal{D}}[s_*, s_{\mathcal{I}}, s_{\mathcal{J}}|y] = \mathbb{P}_{\mathcal{D}}[s_*|y] \prod_{i \in \mathcal{I}} \mathbb{P}_{\mathcal{D}}[s_i|y] \prod_{j \in \mathcal{J}} \mathbb{P}_{\mathcal{D}}[s_j|y].$$

We also assume for simplicity that the main task model makes symmetric errors given the class of target variable, that is,  $\mathbb{P}_{\mathcal{D}}[s_* \neq y|y]$  is fixed with respect to  $y$  for all  $\mathcal{D} \in \{\mathcal{D}_b, \mathcal{D}_a\}$ .

### Characterizing Models: Truth Rate ( $\alpha$ ) and False Rate

( $\epsilon$ ) Each auxiliary model  $k \in \mathcal{I} \cup \mathcal{J}$  is characterized by two values, their truth rate ( $\alpha$ ) and false rate ( $\epsilon$ ) over benign and adversarial distributions. These values measure the *consistency* of the model with the ground truth:

Permissive Models:

$$\alpha_{i,\mathcal{D}} := \mathbb{P}_{\mathcal{D}}[s_i = y|y = 1], \quad \epsilon_{i,\mathcal{D}} := \mathbb{P}_{\mathcal{D}}[s_i \neq y|y = 0]$$

Preventative Models:

$$\alpha_{j,\mathcal{D}} := \mathbb{P}_{\mathcal{D}}[s_j = y|y = 0], \quad \epsilon_{j,\mathcal{D}} := \mathbb{P}_{\mathcal{D}}[s_j \neq y|y = 1]$$

Note that, given the asymmetric nature of these auxiliary models, we do *not* necessarily have  $\epsilon_{k,\mathcal{D}} = 1 - \alpha_{k,\mathcal{D}}$ . In addition, for a high quality permissive model ( $k \in \mathcal{I}$ ), or a high quality preventative model ( $k \in \mathcal{J}$ ) for which the logic rules mostly hold, we expect  $\alpha_{k,\mathcal{D}}$  to be large and  $\epsilon_{k,\mathcal{D}}$  to be small.

We define the truth rate of main model over data examples drawn from  $\mathcal{D} \in \{\mathcal{D}_b, \mathcal{D}_a\}$  as  $\alpha_{*,\mathcal{D}} := \mathbb{P}_{\mathcal{D}}(s_* = y)$ , and its false rate as  $\epsilon_{*,\mathcal{D}} := \mathbb{P}_{\mathcal{D}}(s_* \neq y) = 1 - \alpha_{*,\mathcal{D}}$ .

These characteristics are of integral importance to weighted robust accuracy of KEMLP. To combine all the models together, we define upper and lower bounds to truth rates and false rates. For the main model, we have  $\wedge \alpha_* := \min_{\mathcal{D}} \alpha_{*,\mathcal{D}}$  and  $\vee \alpha_* := \max_{\mathcal{D}} \alpha_{*,\mathcal{D}}$ . For the auxiliary models, on the other hand, for each model index  $k \in \mathcal{I} \cup \mathcal{J}$ , we have

$$\begin{aligned} \wedge \alpha_k &:= \min_{\mathcal{D}} \alpha_{k,\mathcal{D}}, & \wedge \epsilon_k &:= \min_{\mathcal{D}} \epsilon_{k,\mathcal{D}} \\ \vee \alpha_k &:= \max_{\mathcal{D}} \alpha_{k,\mathcal{D}}, & \vee \epsilon_k &:= \max_{\mathcal{D}} \epsilon_{k,\mathcal{D}}. \end{aligned}$$

Intuitively, the difference between  $\wedge \alpha$  and  $\vee \alpha$  (resp.  $\wedge \epsilon$  and  $\vee \epsilon$ ) indicates the ‘‘robustness’’ of each individual model. If a model performs very similarly when it is given a benign and an adversarial example, we have that  $\wedge \alpha$  should be similar to  $\vee \alpha$  (resp.  $\wedge \epsilon$  to  $\vee \epsilon$ ).

The truth and false rates of models directly influence the factor weights which govern the influence of models in the main task. In Appendix A.2 we prove that the optimal weight of an auxiliary model is bounded by  $w_k \geq \log \wedge \alpha_k (1 - \vee \epsilon_k) / (1 - \wedge \alpha_k) \vee \epsilon_k$ , for all  $k \in \mathcal{I} \cup \mathcal{J}$ . That

is, the lowest truth rate and highest false rate of an auxiliary model (resp.  $\wedge \alpha_k$  and  $\vee \epsilon_k$ ) are indicative of its influence in the main task. By taking partial derivatives, this lower bound can be shown to be increasing in  $\wedge \alpha_k$  and decreasing in  $\vee \epsilon_k$ . That is, as the lowest truth rate of a model gets higher, KEMLP increases its influence in the weighted majority voting accordingly – in the above nonlinear fashion. The lowest truth rate is often determined by the *robust accuracy*. As a result, the more ‘‘robust’’ an auxiliary model is, the larger the influence on KEMLP, which naturally contributes to its robustness.

**Weighted Robust Accuracy of KEMLP** We now provide a lower bound on the weighted robust accuracy of KEMLP, which can be written as

$$\mathcal{A}^{\text{KEMLP}} = \mathbb{E}_{\mathcal{D} \sim \{\mathcal{D}_a, \mathcal{D}_b\}} \mathbb{E}_{y \sim \mathcal{Y}} [\mathbb{P}_{\mathcal{D}}[o = y|y, \mathbf{w}]]. \quad (2)$$

We first provide one key technical lemma followed by the general theorem.

We see that the key component in  $\mathcal{A}^{\text{KEMLP}}$  is  $\mathbb{P}_{\mathcal{D}}[o = y|y, \mathbf{w}]$ , the conditional probability that a KEMLP pipeline outputs the correct prediction. Using knowledge aggregation rules  $f_*, f_i$  and  $f_j$ , as well as (1), for each  $\mathcal{D} \in \{\mathcal{D}_b, \mathcal{D}_a\}$  we have

$$\begin{aligned} \mathbb{P}_{\mathcal{D}}[o = y|y, \mathbf{w}] &= \mathbb{P}_{\mathcal{D}}[\mathbb{P}[o = y|s_*, s_{\mathcal{I}}, s_{\mathcal{J}}, \mathbf{w}] > 1/2|y] \\ &= \mathbb{P}_{\mathcal{D}}[\langle \mathbf{w}, \mathbf{f}_y(s_*, s_{\mathcal{I}}, s_{\mathcal{J}}) - \mathbf{f}_{1-y}(s_*, s_{\mathcal{I}}, s_{\mathcal{J}}) \rangle > 0|y]. \end{aligned}$$

To bound the above value, we need to characterize the concentration behavior of the random variable

$$\Delta_{\mathbf{w}}(y, s_*, s_{\mathcal{I}}, s_{\mathcal{J}}) := \langle \mathbf{w}, \mathbf{f}_y(s_*, s_{\mathcal{I}}, s_{\mathcal{J}}) - \mathbf{f}_{1-y}(s_*, s_{\mathcal{I}}, s_{\mathcal{J}}) \rangle.$$

That is, we need to bound its left tail below zero. For this purpose, we reason about its expectation, leading to the following lemma.

**Lemma 1.** *Let  $\Delta_{\mathbf{w}}$  be a random variable defined above. Suppose that KEMLP uses optimal parameters  $\mathbf{w}$  such that  $\mathbb{P}[y|s_*, s_{\mathcal{I}}, s_{\mathcal{J}}] = \mathbb{P}[o|s_*, s_{\mathcal{I}}, s_{\mathcal{J}}, \mathbf{w}]$ . Let also  $r_y$  denote the log-ratio of class imbalance  $\log \frac{\mathbb{P}[y=1]}{\mathbb{P}[y=0]}$ . For a fixed  $y \in \mathcal{Y}$  and  $\mathcal{D} \in \{\mathcal{D}_b, \mathcal{D}_a\}$ , one has*

$$\begin{aligned} \mathbb{E}_{s_*, s_{\mathcal{I}}, s_{\mathcal{J}}} [\Delta_{\mathbf{w}}(y, s_*, s_{\mathcal{I}}, s_{\mathcal{J}})|y] \\ \geq \mu_{d_*, \mathcal{D}} + y \mu_{d_{\mathcal{I}}, \mathcal{D}} + (1 - y) \mu_{d_{\mathcal{J}}, \mathcal{D}} + (2y - 1) r_y := \mu_{y, \mathcal{D}}, \end{aligned}$$

where

$$\begin{aligned} \mu_{d_*, \mathcal{D}} &= \alpha_{*, \mathcal{D}} \log \frac{\wedge \alpha_*}{1 - \wedge \alpha_*} + (1 - \alpha_{*, \mathcal{D}}) \log \frac{1 - \vee \alpha_*}{\vee \alpha_*}, \\ \mu_{d_{\mathcal{I}}, \mathcal{D}} &= \sum_{i \in \mathcal{I}} \alpha_{i, \mathcal{D}} \log \frac{\wedge \alpha_i}{\vee \epsilon_i} + (1 - \alpha_{i, \mathcal{D}}) \log \frac{1 - \vee \alpha_i}{1 - \wedge \epsilon_i} \\ &\quad - \sum_{j \in \mathcal{J}} \epsilon_{j, \mathcal{D}} \log \frac{\vee \alpha_j}{\wedge \epsilon_j} - (1 - \epsilon_{j, \mathcal{D}}) \log \frac{1 - \wedge \alpha_j}{1 - \vee \epsilon_j}, \end{aligned}$$

and

$$\begin{aligned} \mu_{d_{\mathcal{J},\mathcal{D}}} &= \sum_{j \in \mathcal{J}} \alpha_{j,\mathcal{D}} \log \frac{\wedge \alpha_j}{\vee \epsilon_j} + (1 - \alpha_{j,\mathcal{D}}) \log \frac{1 - \vee \alpha_j}{1 - \wedge \epsilon_j} \\ &\quad - \sum_{i \in \mathcal{I}} \epsilon_{i,\mathcal{D}} \log \frac{\vee \alpha_i}{\wedge \epsilon_i} - (1 - \epsilon_{i,\mathcal{D}}) \log \frac{1 - \wedge \alpha_i}{1 - \vee \epsilon_i}. \end{aligned}$$

*Proof Sketch.* This lemma can be derived by first decomposing  $\Delta_{\mathbf{w}}$  into parts that are relevant for  $s_*$ ,  $s_{\mathcal{I}}$ ,  $s_{\mathcal{J}}$ , namely there exist  $d_{*,\mathcal{D}}$ ,  $d_{\mathcal{I},\mathcal{D}}$ ,  $d_{\mathcal{J},\mathcal{D}}$  such that

$$\Delta_{\mathbf{w}}(y, s_*, s_{\mathcal{I}}, s_{\mathcal{J}}) = d_{*,\mathcal{D}} + y d_{\mathcal{I},\mathcal{D}} + (1 - y) d_{\mathcal{J},\mathcal{D}} + (2y - 1) r_y.$$

Then we prove that  $\mu_{*,\mathcal{D}} \leq \mathbb{E}[d_{*,\mathcal{D}}]$  for the main model, and  $\mu_{d_{\mathcal{K},\mathcal{D}}} \leq \mathbb{E}[d_{\mathcal{K},\mathcal{D}}]$  for  $\mathcal{K} \in \{\mathcal{I}, \mathcal{J}\}$ , the permissive and preventative models. The full proof is presented in Appendix A.3.

**Discussion** The above lemma illustrates the relationship between the models and  $\mathcal{A}^{\text{KEMLP}}$ . Intuitively, the larger  $\mu_{y,\mathcal{D}}$  is, the further away the expectation of  $\Delta_{\mathbf{w}}(y, s_*, s_{\mathcal{I}}, s_{\mathcal{J}})$  is from 0, and thus, the larger the probability that  $\Delta_{\mathbf{w}}(y, s_*, s_{\mathcal{I}}, s_{\mathcal{J}}) > 0$ . We see that  $\mu_{y,\mathcal{D}}$  consists of three terms:  $\mu_{d_{*,\mathcal{D}}}$ ,  $\mu_{d_{\mathcal{I},\mathcal{D}}}$ ,  $\mu_{d_{\mathcal{J},\mathcal{D}}}$ , measuring the contributions from the main model for all  $y$ , permissive models and preventative models for  $y = 1$  and  $y = 0$ , respectively. More specifically,  $\mu_{y,\mathcal{D}}$  is increasing in terms of a weighted sum of  $\alpha_i$ , and decreasing in terms of a weighted sum of  $\epsilon_j$ . When  $s_i \implies y$  holds (permissive models), it implies a large  $\alpha_i$  for  $y = 1$ , whereas when  $y \implies s_j$  holds (preventative model) it implies a small  $\epsilon_j$  for  $y = 1$ . Thus, this lemma connects the property of auxiliary models to the weighted robust accuracy of KEMLP.

## 4.2. Convergence of $\mathcal{A}^{\text{KEMLP}}$

Now we are ready to present our convergence result.

**Theorem 1** (Convergence of  $\mathcal{A}^{\text{KEMLP}}$ ). *For  $y \in \mathcal{Y}$  and  $\mathcal{D} \in \{\mathcal{D}_b, \mathcal{D}_a\}$ , let  $\mu_{y,\mathcal{D}}$  be defined as in Lemma 1. Suppose that the modeling assumption holds, and suppose that  $\mu_{d_{\mathcal{K},\mathcal{D}}} > 0$ , for all  $\mathcal{K} \in \{\mathcal{I}, \mathcal{J}\}$  and  $\mathcal{D} \in \{\mathcal{D}_b, \mathcal{D}_a\}$ . Then*

$$\mathcal{A}^{\text{KEMLP}} \geq 1 - \mathbb{E}_{\mu_{y,\mathcal{D}}} [\exp(-2\mu_{y,\mathcal{D}}^2/v^2)], \quad (3)$$

where  $v^2$  is the variance upper bound to  $\mathbb{P}[o = y|y, \mathbf{w}]$  with

$$v^2 = 4 \left( \log \frac{\vee \alpha_*}{1 - \wedge \alpha_*} \right)^2 + \sum_{k \in \mathcal{I} \cup \mathcal{J}} \left( \log \frac{\vee \alpha_k (1 - \wedge \epsilon_k)}{\wedge \epsilon_k (1 - \vee \alpha_k)} \right)^2.$$

*Proof Sketch.* We begin by subtracting the term  $\mu_{y,\mathcal{D}}$  from  $\mathbb{P}_{\mathcal{D}}(o = y|y, \mathbf{w})$ , and then decomposing the result into individual summands, where each summand is induced by a single model. We then treat each summand as a bounded increment whose sum is a submartingale. Followed by an application of generalized bounded difference inequality (van de Geer, 2002), we arrive at the proof, whose full details can be found in Appendix A.4.

**Discussion** In the following, we attempt to understand the scaling of the weighted robust accuracy of KEMLP in terms of models' characteristics.

*Impact of truth rates and false rates:* We note that  $\mu_{d_{\mathcal{K},\mathcal{D}}}$  for  $\mathcal{K} \in \{\mathcal{I}, \mathcal{J}\}$ , which is an additive component of  $\mu_{y,\mathcal{D}}$ , poses importance to understand the factors contributing to the performance of KEMLP. Generally, larger  $\mu_{d_{\mathcal{K},\mathcal{D}}}$  (hence  $\mu_{y,\mathcal{D}}$ ) would increase the right tail probability of  $\Delta_{\mathbf{w}}(y, s_*, s_{\mathcal{I}}, s_{\mathcal{J}})$  leading to a larger weighted accuracy for KEMLP. Although exceptions exist in cases where the variance increases disproportionately, here in our discussion we first focus on parameters that increase  $\mu_{d_{\mathcal{K},\mathcal{D}}}$ . Towards that, we simplify our exposition and let each auxiliary model have the same truth and false rate over both benign and adversarial examples, and within each type, where the exact parameters are given by  $\alpha_k := \alpha_{k,\mathcal{D}} = \wedge \alpha_{k,\mathcal{D}} = \vee \alpha_{k,\mathcal{D}}$  and  $\epsilon_k := \epsilon_{k,\mathcal{D}} = \wedge \epsilon_{k,\mathcal{D}} = \vee \epsilon_{k,\mathcal{D}}$ , for  $k \in \mathcal{I} \cup \mathcal{J}$ . In this simplified setting where the expected performance improvement by the auxiliary models is given by  $\mu_{d_{\mathcal{K},\mathcal{D}}}$  for  $\mathcal{K} \in \{\mathcal{I}, \mathcal{J}\}$  and fixed with respect to  $\mathcal{D}$ , one can observe through partial derivatives that  $\mu_{d_{\mathcal{K},\mathcal{D}}}$  is increasing over  $\alpha_k$  and decreasing over  $\epsilon_k$ . This explains why the two types of knowledge rules would help: high-quality permissive models would have high truth rate and low false rate ( $\alpha_i$  and  $\epsilon_i$ ), as well as the preventative models ( $\alpha_j$  and  $\epsilon_j$ ), yet with different coverages for  $y \in \mathcal{Y}$ .

*Auxiliary models in KEMLP - the more the merrier?* Next, we investigate the effect of the number of auxiliary models. To simplify, let  $|\mathcal{I}| = |\mathcal{J}|$ , and let  $\hat{\mu}_{y,\mathcal{D}}$  be a random variable with  $\hat{\mu}_{y,\mathcal{D}} = \mu_{y,\mathcal{D}}/(n+1)$ , and  $\hat{v}^2 = v^2/(n+1)$ . The exponent thus becomes  $-\mu_{y,\mathcal{D}}^2/v^2 = -(n+1)\hat{\mu}_{y,\mathcal{D}}^2/\hat{v}^2$ . One can show that  $\hat{\mu}_{y,\mathcal{D}}^2/\hat{v}^2 \geq c$  for some positive constant  $c$ , implying that  $\mathcal{A}^{\text{KEMLP}} \geq 1 - \exp(-2(n+1)c)$ . That is, increasing the number of models generally improves the weighted robust accuracy of KEMLP. To demonstrate this, we now focus on understanding the scaling of weighted robust accuracy on a simplified setting. We assume that the auxiliary models are *homogeneous* for each type: permissive or preventative. For example,  $\alpha_k$  is fixed with respect to  $k \in \mathcal{I} \cup \mathcal{J}$ , hence we drop the subscripts, i.e.,  $\alpha_{k,\mathcal{D}} = \alpha$  and  $\epsilon_{k,\mathcal{D}} = \epsilon$ . We assume that the same number of auxiliary models are used, namely  $|\mathcal{I}| = |\mathcal{J}| = n$ , and that the classes are balanced with  $\mathbb{P}_{\mathcal{D}}(y = 1) = \mathbb{P}_{\mathcal{D}}(y = 0)$ , for all  $\mathcal{D} \in \{\mathcal{D}_b, \mathcal{D}_a\}$ . Finally, we let  $\alpha_{*,\mathcal{D}_b} = 1$  and  $\alpha_{*,\mathcal{D}_a} = 0$ , and  $\alpha - \epsilon > 0$ . Then, the following holds.

**Corollary 1** (Homogenous models). *The weighted robust accuracy of KEMLP in the homogeneous setting satisfies*

$$\mathcal{A}^{\text{KEMLP}} \geq 1 - \exp(-2n(\alpha - \epsilon)^2).$$

*In particular, one has  $\lim_{n \rightarrow \infty} \mathcal{A}^{\text{KEMLP}} = 1$ .*

For this particular case, the predicted class for the target

variable  $y$  is based upon an (unweighted) majority voting decision. The above result suggests that for a setting where the auxiliary models are homogeneous with different coverage, the performance of KEMLP to predict the output variable  $y$  robustly is determined by: (a) the difference between the probability of predicting the output variable correctly and that of making an erroneous prediction, that is,  $\alpha - \epsilon$ , and (b) the number of auxiliary models. Consequently,  $\mathcal{A}^{\text{KEMLP}}$  converges to 1 exponentially fast in the number of auxiliary models as long as  $\alpha - \epsilon > 0$ , which is naturally satisfied by the principle KEMLP employs while constructing the logical relations between the output variable and different knowledge.

### 4.3. Comparing $\mathcal{A}^{\text{KEMLP}}$ and $\mathcal{A}^{\text{main}}$

Theorem 1 guarantees that the addition of models allows the weighted robust accuracy of KEMLP to converge to 1 exponentially fast. We now introduce a sufficient condition under which  $\mathcal{A}^{\text{KEMLP}}$  is strictly better than  $\mathcal{A}^{\text{main}}$ .

**Theorem 2** (Sufficient condition for  $\mathcal{A}^{\text{KEMLP}} > \mathcal{A}^{\text{main}}$ ). *Let the number of permissive and preventative models be the same and denoted by  $n$  such that  $n := |\mathcal{I}| = |\mathcal{J}|$ . Note that the weighted accuracy of the main model in terms of its truth rate is simply  $\alpha_* := \sum_{\mathcal{D} \in \{\mathcal{D}_b, \mathcal{D}_a\}} \pi_{\mathcal{D}} \alpha_{*, \mathcal{D}}$ . Moreover, let  $\mathcal{K}, \mathcal{K}' \in \{\mathcal{I}, \mathcal{J}\}$  with  $\mathcal{K} \neq \mathcal{K}'$  and for any  $\mathcal{D} \in \{\mathcal{D}_b, \mathcal{D}_a\}$ , let*

$$\gamma_{\mathcal{D}} := \frac{1}{n+1} \min_{\mathcal{K}} \left\{ \alpha_{*, \mathcal{D}} - 1/2 + \sum_{k \in \mathcal{K}} \alpha_{k, \mathcal{D}} - \sum_{k' \in \mathcal{K}'} \epsilon_{k', \mathcal{D}} \right\}.$$

*If  $\gamma_{\mathcal{D}} > \sqrt{\frac{4}{n+1} \log \frac{1}{1-\alpha_*}}$  for all  $\mathcal{D} \in \{\mathcal{D}_b, \mathcal{D}_a\}$ , then  $\mathcal{A}^{\text{KEMLP}} > \mathcal{A}^{\text{main}}$ .*

*Proof Sketch.* We first approximate  $\Delta_{\mathbf{w}}(y, s_*, s_{\mathcal{I}}, s_{\mathcal{J}})$  with a Poisson Binomial random variable and apply the relevant Chernoff bound. Imposing a strict bound between the Chernoff result and the true and false rates of main model concludes the proof. We note that this bound is slightly simplified, and our full proof in the Appendix A.5 is tighter.

**Discussion** We start by noting that  $\gamma_{\mathcal{D}}$  is a combined truth rate of all models normalized over the number of models. That is, for a fixed distribution  $\mathcal{D}$ ,  $\alpha_{*, \mathcal{D}} - 1/2$  indicates the truth rate of main task model over a random classifier and  $\sum_{k \in \mathcal{K}} \alpha_{k, \mathcal{D}} - \sum_{k' \in \mathcal{K}'} \epsilon_{k', \mathcal{D}}$  refers to the improvement by the auxiliary models on top of the main task model. More specifically, in cases where the true class of output variable is positive with  $y = 1$ ,  $\sum_{i \in \mathcal{I}} \alpha_{i, \mathcal{D}} - \sum_{j \in \mathcal{J}} \epsilon_{j, \mathcal{D}}$  account for the total (and unnormalized) success of permissive models in identifying  $y = 1$  interfered by the failure of preventative model in identifying  $y = 1$  (resp. For  $y = 0$ ,  $\mathcal{K} = \mathcal{J}$ ). Hence,  $\gamma_{\mathcal{D}}$  is the "worst-case" combined truth rate of all

models, where the worst-case refers to minimization over all possible labels of target variable.

Theorem 2 therefore forms a relationship between the improvement of KEMLP over the main task model and the combined truth rate of models, and theoretically justifies our intuition – larger truth rates and lower false rates of individual auxiliary models result in larger combined truth rate  $\gamma_{\mathcal{D}}$ , hence making the sufficient condition more likely to hold. Additionally, employing a large number of auxiliary models is found to be beneficial for better KEMLP performance, as we conclude in Corollary 1 as well. Our finding here also confirms that in the extreme scenarios where the main task model has a perfect clean and robust truth rate ( $\alpha_* = 1$ ), it is *not* possible to improve upon the main task model. Conversely, when  $\alpha_* = 0$ , any improvement by KEMLP would result in absolute improvement over the main model.

## 5. Experimental Evaluation

In this section, we evaluate KEMLP based on the traffic sign recognition task against different adversarial attacks and corruptions, including the physical attacks (Eykholt et al., 2018),  $\mathcal{L}_{\infty}$  bounded attacks, unforeseen attacks (Kang et al., 2019), and common corruptions (Hendrycks and Dietterich, 2019). We show that under both whitebox and blackbox settings against a *diverse* set of attacks, 1) KEMLP achieves significantly higher robustness than baselines, 2) KEMLP maintains similar clean accuracy with a strong main task model whose clean accuracy is originally high (e.g., vanilla CNN), 3) KEMLP even achieves higher clean accuracy than a relatively weak main task model whose clean accuracy is originally low as a tradeoff for its robustness (e.g., adversarially trained models).

### 5.1. Experimental Setup

**Dataset** Following existing work (Eykholt et al., 2018; Wu et al., 2019) that evaluate ML robustness on traffic sign data, we adopt LISA (Mogelmoose et al., 2012) and GT-SRB (Stallkamp et al., 2012) for training and evaluation. All data are processed by standard crop-and-resize to  $32 \times 32$  as described in (Sermanet and LeCun, 2011). In this paper, we conduct the evaluation on two dataset settings: 1) *Setting-A*: a subset of GTSRB, which contains 12 types of German traffic signs. In total, there are 14880 samples in the training set, 972 samples in the validation set, and 3888 samples in the test set; 2) *Setting-B*: a modified version of Setting-A, where the German stop signs are replaced with the U.S. stop signs from LISA, following (Eykholt et al., 2018).

**Models** We adopt the GTSRB-CNN architecture (Eykholt et al., 2018) as the main task model. KEMLP is constructed based on the main task model together with a set of auxiliary task models (e.g., color, shape, and content detectors). To

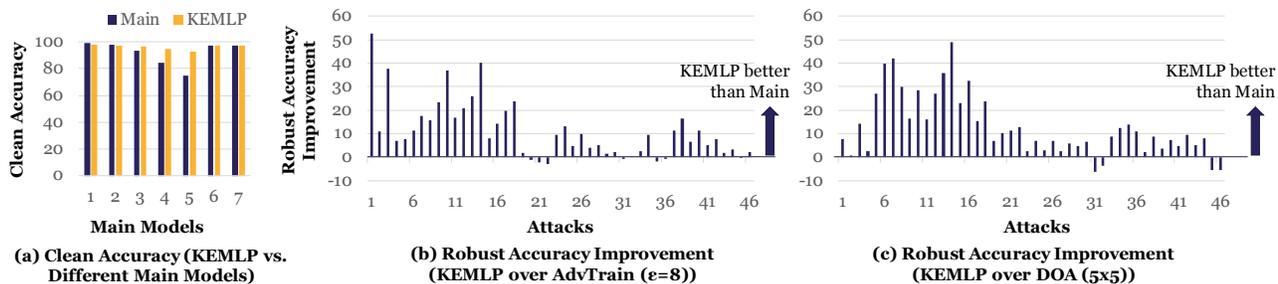

Figure 2. (a) Clean accuracy and (b) (c) robust accuracy improvement of KEMLP ( $\beta = 0.5$ ) over baselines against different attacks under both whitebox and blackbox settings. The represented attack list and results of other baselines are in Appendix B.2.

Table 1. Model performance (%) under physical attacks ( $\beta = 0.4$ ). Performance gain and loss of KEMLP over baselines are highlighted.

|                              | Main      |            |              | KEMLP          |             |               |
|------------------------------|-----------|------------|--------------|----------------|-------------|---------------|
|                              | Clean Acc | Robust Acc | W-Robust Acc | Clean Acc      | Robust Acc  | W-Robust Acc  |
| GTSRB-CNN                    | 100       | 5          | 52.5         | 100( $\pm 0$ ) | 87.5(+82.5) | 93.75(+41.25) |
| AdvTrain ( $\epsilon = 4$ )  | 100       | 12.5       | 56.25        | 100( $\pm 0$ ) | 90(+77.5)   | 95(+38.75)    |
| AdvTrain ( $\epsilon = 8$ )  | 97.5      | 37.5       | 67.5         | 100(+2.5)      | 90(+52.5)   | 95(+27.5)     |
| AdvTrain ( $\epsilon = 16$ ) | 87.5      | 50         | 68.75        | 100(+12.5)     | 90(+40)     | 95(+26.25)    |
| AdvTrain ( $\epsilon = 32$ ) | 62.5      | 32.5       | 47.5         | 100(+37.5)     | 90(+57.5)   | 95(+47.5)     |
| DOA (5x5)                    | 95        | 90         | 92.5         | 100(+5)        | 100(+10)    | 100(+7.5)     |
| DOA (7x7)                    | 57.5      | 32.5       | 45           | 100(+42.5)     | 100(+67.5)  | 100(+55)      |

train the weights of factors in KEMLP, we use  $\beta$  to denote the prior belief on balance between benign and adversarial distributions. More details on implementation are provided in Appendix B.3.

**Baselines** To demonstrate the superiority of KEMLP, we compare it with two state-of-the-art baselines: **adversarial training** (Madry et al., 2017) and **DOA** (Wu et al., 2019), which are strong defenses against  $\mathcal{L}_p$  bounded attacks and physically attacks respectively. Detailed setup for baselines is given in Appendix B.1.

**Evaluated Attacks and Corruptions** We consider four types of attacks for thorough evaluation: 1) *physical attacks* on stop signs (Eykholt et al., 2018); 2)  *$\mathcal{L}_\infty$  bounded attacks* (Madry et al., 2017) with  $\epsilon \in \{4, 8, 16, 32\}$ ; 3) *Unforeseen attacks*, which produce a diverse set of unforeseen test distributions (e.g. Elastic, JPEG, Fog) distinct from  $\mathcal{L}_p$  bounded perturbation (Kang et al., 2019); 4) *common corruptions* (Hendrycks and Dietterich, 2019). We present examples of these adversarial instances in Appendix B.4. For each attack, we consider both the *whitebox attack* against the main task model and *blackbox attack* by distilling either the main task model or the whole KEMLP pipeline. More details can be found in Appendix B.2.

## 5.2. Evaluation Results

Here we compare the clean accuracy, robust accuracy, and weighted robustness (W-Robust Accuracy) for baselines and KEMLP under different attacks and settings.

**Clean accuracy of KEMLP** First, we present the clean accuracy of KEMLP and baselines in Figure 2 (a) and Tables 1–4. As demonstrated, the clean accuracy of KEMLP is generally high (over 90%), by either maintaining the high clean accuracy of strong main task models (e.g., vanilla DNN) or improving upon the weak main task models with relatively low clean accuracy (e.g., adversarially trained models). It is clear that KEMLP can relax the tradeoff between benign and robust accuracy and maintain the high performance for both via knowledge integration.

**Robustness against diverse attacks** We then present the robustness of KEMLP based on different main task models against the physical attacks, which is very challenging to defend currently (Table 1),  $\mathcal{L}_p$  bounded attacks (Table 2), unseen attacks (Table 3), and common corruptions (Table 4) under whitebox attack setting. The corresponding results for blackbox setting can be found in Appendix B.5. From the tables, we observe that KEMLP achieves significant *robustness gain* over baselines. Note that although adversarial training improves the robustness against  $\mathcal{L}_\infty$  attacks and DOA helps to defend against physical attacks, they are not robust to other types of attacks or corruptions. In contrast, KEMLP presents general robustness against a range of attacks and corruptions without further adaptation.

**Performance stability of KEMLP** We conduct additional ablation studies on  $\beta$ , representing the prior belief on the benign and adversarial distribution balance. We set  $\beta = 0.5$  for KEMLP indicating a balanced random guess

## Knowledge Enhanced Machine Learning Pipeline against Diverse Adversarial Attacks

Table 2. Accuracy (%) under whitebox  $\mathcal{L}_\infty$  attacks ( $\beta = 0.8$ )

| Models                       |       | $\epsilon = 0$ | $\epsilon = 4$      | $\epsilon = 8$       | $\epsilon = 16$      | $\epsilon = 32$      |
|------------------------------|-------|----------------|---------------------|----------------------|----------------------|----------------------|
| GTSRB-CNN                    | Main  | <b>99.38</b>   | 67.31               | 43.13                | 13.50                | 3.63                 |
|                              | KEMLP | 98.28(-1.10)   | 85.39(+18.08)       | 71.76(+28.63)        | 48.89(+35.39)        | 26.13(+22.50)        |
| AdvTrain ( $\epsilon = 4$ )  | Main  | 97.94          | 87.94               | 68.85                | 38.66                | 8.77                 |
|                              | KEMLP | 97.89(-0.05)   | <b>92.80(+4.86)</b> | 79.58(+10.73)        | 57.48(+18.82)        | 28.58(+19.81)        |
| AdvTrain ( $\epsilon = 8$ )  | Main  | 93.72          | 84.21               | 71.76                | 43.16                | 13.01                |
|                              | KEMLP | 96.79(+3.07)   | 92.08(+7.87)        | 81.58(+9.82)         | 59.18(+16.02)        | 30.61(+17.60)        |
| AdvTrain ( $\epsilon = 16$ ) | Main  | 84.54          | 78.58               | 71.89                | 55.99                | 19.55                |
|                              | KEMLP | 94.68(+10.14)  | 91.64(+13.06)       | <b>85.55(+13.66)</b> | 67.98(+11.99)        | 32.61(+13.06)        |
| AdvTrain ( $\epsilon = 32$ ) | Main  | 74.74          | 70.24               | 65.61                | 56.22                | 29.04                |
|                              | KEMLP | 91.46(+16.72)  | 88.58(+18.34)       | 83.23(+17.62)        | <b>72.02(+15.80)</b> | <b>41.90(+12.86)</b> |
| DOA (5x5)                    | Main  | 97.43          | 57.46               | 28.76                | 5.81                 | 0.85                 |
|                              | KEMLP | 97.45(+0.02)   | 83.85(+26.39)       | 67.98(+39.22)        | 45.27(+39.46)        | 24.28(+23.43)        |
| DOA (7x7)                    | Main  | 97.27          | 38.50               | 9.75                 | 2.83                 | 0.67                 |
|                              | KEMLP | 97.22(-0.05)   | 80.89(+42.39)       | 63.40(+53.65)        | 49.20(+46.37)        | 31.04(+30.37)        |

Table 3. Accuracy (%) under whitebox unforeseen attacks ( $\beta = 0.8$ )

|                              | Clean | Fog-256       | Fog-512              | Snow-0.25            | Snow-0.75            | Jpeg-0.125           | Jpeg-0.25            | Gabor-20             | Gabor-40            | Elastic-1.5         | Elastic-2.0          |
|------------------------------|-------|---------------|----------------------|----------------------|----------------------|----------------------|----------------------|----------------------|---------------------|---------------------|----------------------|
| GTSRB-CNN                    | Main  | <b>99.38</b>  | 59.65                | 34.18                | 56.58                | 24.54                | 55.74                | 27.01                | 57.25               | 32.41               | 44.78                |
|                              | KEMLP | 98.28(-1.10)  | 76.95(+17.30)        | 62.83(+28.65)        | 78.94(+22.36)        | 53.22(+28.68)        | 79.63(+23.89)        | 63.40(+36.39)        | 80.17(+22.92)       | 65.20(+32.79)       | 69.34(+24.56)        |
| AdvTrain ( $\epsilon = 4$ )  | Main  | 97.94         | 55.53                | 29.50                | 66.31                | 32.61                | 56.58                | 28.11                | 73.30               | 46.76               | 57.25                |
|                              | KEMLP | 97.89(-0.05)  | 76.08(+20.55)        | 61.96(+32.46)        | 80.45(+14.14)        | 57.84(+25.23)        | 84.23(+27.65)        | 68.57(+40.46)        | 81.48(+8.18)        | 65.77(+19.01)       | 71.19(+13.94)        |
| AdvTrain ( $\epsilon = 8$ )  | Main  | 93.72         | 50.03                | 23.56                | 63.71                | 34.93                | 57.56                | 26.16                | 76.72               | 53.76               | 48.25                |
|                              | KEMLP | 96.79(+3.07)  | 76.59(+26.56)        | 63.97(+40.41)        | 81.40(+17.69)        | 57.07(+22.14)        | 85.11(+27.55)        | 68.70(+42.54)        | 85.29(+8.57)        | 68.90(+15.14)       | 68.78(+20.53)        |
| AdvTrain ( $\epsilon = 16$ ) | Main  | 84.54         | 47.92                | 19.75                | 66.46                | 37.60                | 66.56                | 34.23                | 78.01               | 64.33               | 55.48                |
|                              | KEMLP | 94.68(+10.14) | 77.13(+29.21)        | 64.38(+44.63)        | <b>81.64(+15.18)</b> | 58.20(+20.60)        | <b>86.99(+20.43)</b> | 70.40(+36.17)        | <b>87.42(+9.41)</b> | 72.61(+8.28)        | 67.31(+11.83)        |
| AdvTrain ( $\epsilon = 32$ ) | Main  | 74.74         | 48.71                | 22.84                | 61.78                | 38.91                | 63.58                | 43.49                | 70.37               | 65.20               | 54.58                |
|                              | KEMLP | 91.46(+16.72) | <b>79.22(+30.51)</b> | <b>66.33(+43.49)</b> | 81.20(+19.42)        | <b>64.53(+26.62)</b> | 86.70(+23.12)        | <b>73.38(+29.89)</b> | 87.04(+16.67)       | <b>74.92(+9.72)</b> | 66.38(+11.80)        |
| DOA (5x5)                    | Main  | 97.43         | 58.00                | 32.69                | 61.19                | 28.34                | 41.13                | 11.29                | 55.43               | 29.55               | 58.02                |
|                              | KEMLP | 97.45(+0.02)  | 76.85(+18.85)        | 63.07(+30.38)        | 78.78(+17.59)        | 56.76(+28.42)        | 78.60(+37.47)        | 61.78(+50.49)        | 80.25(+24.82)       | 63.89(+34.34)       | <b>72.69(+14.67)</b> |
| DOA (7x7)                    | Main  | 97.27         | 59.88                | 38.01                | 62.47                | 30.17                | 23.46                | 3.65                 | 54.58               | 27.29               | 56.33                |
|                              | KEMLP | 97.22(-0.05)  | 78.09(+18.21)        | 62.76(+24.75)        | 79.68(+17.21)        | 58.26(+28.09)        | 74.25(+50.79)        | 61.39(+37.74)        | 79.06(+24.48)       | 62.29(+35.00)       | 71.27(+14.94)        |

Table 4. Accuracy (%) under common corruptions ( $\beta = 0.2$ )

|                              | Clean | Fog           | Contrast            | Brightness           |
|------------------------------|-------|---------------|---------------------|----------------------|
| GTSRB-CNN                    | Main  | <b>99.38</b>  | 76.23               | 57.61                |
|                              | KEMLP | 98.28(-1.10)  | <b>78.14(+1.91)</b> | 72.43(+14.82)        |
| AdvTrain ( $\epsilon = 4$ )  | Main  | 97.94         | 63.81               | 42.31                |
|                              | KEMLP | 97.89(-0.05)  | 70.29(+6.48)        | 67.46(+25.16)        |
| AdvTrain ( $\epsilon = 8$ )  | Main  | 93.72         | 59.05               | 31.97                |
|                              | KEMLP | 96.79(+3.07)  | 67.41(+8.36)        | 66.69(+34.72)        |
| AdvTrain ( $\epsilon = 16$ ) | Main  | 84.54         | 56.58               | 34.31                |
|                              | KEMLP | 94.68(+10.14) | 66.80(+10.22)       | 68.39(+34.08)        |
| AdvTrain ( $\epsilon = 32$ ) | Main  | 74.74         | 50.87               | 30.45                |
|                              | KEMLP | 91.46(+16.72) | 64.94(+14.07)       | 68.31(+37.86)        |
| DOA (5x5)                    | Main  | 97.43         | 73.95               | 62.24                |
|                              | KEMLP | 97.45(+0.02)  | 76.08(+2.13)        | <b>74.38(+12.14)</b> |
| DOA (7x7)                    | Main  | 97.27         | 73.41               | 57.54                |
|                              | KEMLP | 97.22(-0.05)  | 76.00(+2.59)        | 72.40(+14.86)        |

for the distribution tradeoff. We show the clean accuracy and robustness of KEMLP and baselines under diverse 46 attacks in Figure 2. We can see that KEMLP consistently and significantly outperforms the baselines, which indicates the performance stability of KEMLP regarding different distribution ratio  $\beta$ . More results can be found in Appendix B.5, with additional discussions in Appendix B.6.

## 6. Discussions and Future Work

In this paper, we propose KEMLP, which integrates *domain knowledge* with a set of weak auxiliary models to enhance the ML robustness against a diverse set of adversarial attacks and corruptions. While our framework can be extended to other applications, for any knowledge system, one naturally needs domain experts to design the knowledge rules specific to that application. Here we aim to introduce this framework as a prototype, provide a rigorous analysis of it, and demon-

strate the benefit of such construction on an application. Nevertheless, there is probably no universal strategy on how to aggregate knowledge for any arbitrary application, and instead, application-specific constructions are needed. We do believe that, once the principled framework of knowledge fusion is ready, application-specific developments of knowledge rules will naturally follow, similar to what happened previously for knowledge-enriched joint inference.

## Acknowledgements

CZ and the DS3Lab gratefully acknowledge the support from the Swiss National Science Foundation (Project Number 200021\_184628), Innosuisse/SNF BRIDGE Discovery (Project Number 40B2-0\_187132), European Union Horizon 2020 Research and Innovation Programme (DAPHNE, 957407), Botnar Research Centre for Child Health, Swiss Data Science Center, Alibaba, Cisco, eBay, Google Focused Research Awards, Oracle Labs, Swisscom, Zurich Insurance, Chinese Scholarship Council, and the Department of Computer Science at ETH Zurich. BL and the SLLab would like to acknowledge the support from NSF grant No.1910100, NSF CNS 20-46726 CAR, and Amazon Research Award.

## References

Anish Athalye, Nicholas Carlini, and David Wagner. Obfuscated gradients give a false sense of security: Circumventing defenses to adversarial examples. In *Internat-*

- tional Conference on Machine Learning*, pages 274–283. PMLR, 2018.
- Kazuoki Azuma. Weighted sums of certain dependent random variables. *Tohoku Mathematical Journal, Second Series*, 19(3):357–367, 1967.
- Anand Bhattad, Min Jin Chong, Kaizhao Liang, Bo Li, and David A Forsyth. Unrestricted adversarial examples via semantic manipulation. 2020. URL [https://openreview.net/forum?id=Sye\\_OgHFwH](https://openreview.net/forum?id=Sye_OgHFwH).
- Marenglen Biba, Stefano Ferilli, and Floriana Esposito. Protein fold recognition using markov logic networks. In *Mathematical Approaches to Polymer Sequence Analysis and Related Problems*, pages 69–85. Springer, 2011.
- Stéphane Boucheron, Gábor Lugosi, and Pascal Massart. *Concentration inequalities: A nonasymptotic theory of independence*. Oxford university press, 2013.
- Qi-Zhi Cai Cai, Chang Liu, and Dawn Song. Curriculum adversarial training. pages 3740–3747, 7 2018. doi: 10.24963/ijcai.2018/520. URL <https://doi.org/10.24963/ijcai.2018/520>.
- Nicholas Carlini and David Wagner. Adversarial examples are not easily detected: Bypassing ten detection methods. In *Proceedings of the 10th ACM Workshop on Artificial Intelligence and Security*, pages 3–14, 2017a.
- Nicholas Carlini and David Wagner. Towards evaluating the robustness of neural networks. In *IEEE Symposium on Security and Privacy (SP)*, pages 39–57. IEEE, 2017b.
- Yair Carmon, Aditi Raghunathan, Ludwig Schmidt, John C Duchi, and Percy S Liang. Unlabeled data improves adversarial robustness. In *Advances in Neural Information Processing Systems*, pages 11190–11201, 2019.
- Deepayan Chakrabarti, Stanislaw Funiak, Jonathan Chang, and Sofus Macskassy. Joint inference of multiple label types in large networks. In *International Conference on Machine Learning*, pages 874–882. PMLR, 2014.
- Liwei Chen, Yansong Feng, Jinghui Mo, Songfang Huang, and Dongyan Zhao. Joint inference for knowledge base population. In *Proceedings of the 2014 Conference on Empirical Methods in Natural Language Processing (EMNLP)*, pages 1912–1923, 2014.
- Jeremy Cohen, Elan Rosenfeld, and Zico Kolter. Certified adversarial robustness via randomized smoothing. In *International Conference on Machine Learning*, pages 1310–1320. PMLR, 2019.
- Jia Deng, Nan Ding, Yangqing Jia, Andrea Frome, Kevin Murphy, Samy Bengio, Yuan Li, Hartmut Neven, and Hartwig Adam. Large-scale object classification using label relation graphs. In *European conference on computer vision*, pages 48–64. Springer, 2014.
- Krishnamurthy Dj Dvijotham, Jamie Hayes, Borja Balle, Zico Kolter, Chongli Qin, Andras Gyorgy, Kai Xiao, Sven Gowal, and Pushmeet Kohli. A framework for robustness certification of smoothed classifiers using f-divergences. In *International Conference on Learning Representations*, 2020. URL <https://openreview.net/forum?id=SJlKrksFPH>.
- Kevin Eykholt, Ivan Evtimov, Earleence Fernandes, Bo Li, Amir Rahmati, Chaowei Xiao, Atul Prakash, Tadayoshi Kohno, and Dawn Song. Robust physical-world attacks on deep learning visual classification. In *Proceedings of the IEEE Conference on Computer Vision and Pattern Recognition*, pages 1625–1634, 2018.
- Ian J Goodfellow, Yaroslav Bulatov, Julian Ibarz, Sacha Arnoud, and Vinay Shet. Multi-digit number recognition from street view imagery using deep convolutional neural networks. *arXiv preprint arXiv:1312.6082*, 2013.
- Ian J. Goodfellow, Jonathon Shlens, and Christian Szegedy. Explaining and harnessing adversarial examples. In *International Conference on Learning Representations*, 2015.
- Sven Gowal, Krishnamurthy Dvijotham, Robert Stanforth, Rudy Bunel, Chongli Qin, Jonathan Uesato, Relja Arandjelovic, Timothy Mann, and Pushmeet Kohli. On the effectiveness of interval bound propagation for training verifiably robust models. *arXiv preprint arXiv:1810.12715*, 2018.
- Dan Hendrycks and Thomas Dietterich. Benchmarking neural network robustness to common corruptions and perturbations. In *International Conference on Learning Representations*, 2019.
- Andrew Ilyas, Shibani Santurkar, Dimitris Tsipras, Logan Engstrom, Brandon Tran, and Aleksander Madry. Adversarial examples are not bugs, they are features. In *Advances in Neural Information Processing Systems*, pages 125–136, 2019.
- Adel Javanmard, Mahdi Soltanolkotabi, and Hamed Hassani. Precise tradeoffs in adversarial training for linear regression. In *Conference on Learning Theory*, pages 2034–2078. PMLR, 2020.
- Daniel Kang, Yi Sun, Dan Hendrycks, Tom Brown, and Jacob Steinhardt. Testing robustness against unforeseen adversaries. *arXiv preprint arXiv:1908.08016*, 2019.
- Sanjay Kariyappa and Moinuddin K Qureshi. Improving adversarial robustness of ensembles with diversity training. *arXiv preprint arXiv:1901.09981*, 2019.

- Nasser Kehtarnavaz, Norman C Griswold, and DS Kang. Stop-sign recognition based on color/shape processing. *Machine Vision and Applications*, 6(4):206–208, 1993.
- Bai Li, Changyou Chen, Wenlin Wang, and Lawrence Carin. Certified adversarial robustness with additive noise. In *Advances in Neural Information Processing Systems*, pages 9464–9474, 2019.
- Xuanqing Liu, Minhao Cheng, Huan Zhang, and Cho-Jui Hsieh. Towards robust neural networks via random self-ensemble. In *Proceedings of the European Conference on Computer Vision (ECCV)*, pages 369–385, 2018.
- Aleksander Madry, Aleksandar Makelov, Ludwig Schmidt, Dimitris Tsipras, and Adrian Vladu. Towards deep learning models resistant to adversarial attacks. *arXiv preprint arXiv:1706.06083*, 2017.
- Andrew McCallum. Joint inference for natural language processing. In *Proceedings of the Thirteenth Conference on Computational Natural Language Learning*, pages 1–1, 2009.
- Jun Miura, Tsuyoshi Kanda, and Yoshiaki Shirai. An active vision system for real-time traffic sign recognition. In *ITSC2000. 2000 IEEE Intelligent Transportation Systems. Proceedings (Cat. No. 00TH8493)*, pages 52–57. IEEE, 2000.
- Andreas Mogelmoose, Mohan Manubhai Trivedi, and Thomas B Moeslund. Vision-based traffic sign detection and analysis for intelligent driver assistance systems: Perspectives and survey. *IEEE Transactions on Intelligent Transportation Systems*, 13(4):1484–1497, 2012.
- Jeet Mohapatra, Ching-Yun Ko, Sijia Liu, Pin-Yu Chen, Luca Daniel, et al. Rethinking randomized smoothing for adversarial robustness. *arXiv preprint arXiv:2003.01249*, 2020.
- Leland Gerson Neuberg. Causality: Models, reasoning, and inference, 2003.
- Tianyu Pang, Kun Xu, Chao Du, Ning Chen, and Jun Zhu. Improving adversarial robustness via promoting ensemble diversity. *arXiv preprint arXiv:1901.08846*, 2019.
- Hoifung Poon and Pedro Domingos. Joint inference in information extraction. In *AAAI*, volume 7, pages 913–918, 2007.
- Aditi Raghunathan, Sang Michael Xie, Fanny Yang, John Duchi, and Percy Liang. Understanding and mitigating the tradeoff between robustness and accuracy. *arXiv preprint arXiv:2002.10716*, 2020.
- Alexander Ratner, Christopher De Sa, Sen Wu, Daniel Selsam, and Christopher Ré. Data programming: Creating large training sets, quickly. *Advances in neural information processing systems*, 29:3567, 2016.
- Alexander Ratner, Stephen H Bach, Henry Ehrenberg, Jason Fries, Sen Wu, and Christopher Ré. Snorkel: Rapid training data creation with weak supervision. In *Proceedings of the VLDB Endowment. International Conference on Very Large Data Bases*, volume 11, page 269. NIH Public Access, 2017.
- Matthew Richardson and Pedro Domingos. Markov logic networks. *Machine learning*, 62(1-2):107–136, 2006.
- Andrew Ross and Finale Doshi-Velez. Improving the adversarial robustness and interpretability of deep neural networks by regularizing their input gradients. In *Proceedings of the AAAI Conference on Artificial Intelligence*, volume 32, 2018.
- Carsten Rother, Vladimir Kolmogorov, and Andrew Blake. ”grabcut” interactive foreground extraction using iterated graph cuts. *ACM transactions on graphics (TOG)*, 23(3):309–314, 2004.
- Hadi Salman, Jerry Li, Ilya Razenshteyn, Pengchuan Zhang, Huan Zhang, Sebastien Bubeck, and Greg Yang. Provably robust deep learning via adversarially trained smoothed classifiers. In *Advances in Neural Information Processing Systems*, pages 11292–11303, 2019.
- Pouya Samangouei, Maya Kabkab, and Rama Chellappa. Defense-gan: Protecting classifiers against adversarial attacks using generative models. *arXiv preprint arXiv:1805.06605*, 2018.
- Lukas Schott, Jonas Rauber, Matthias Bethge, and Wieland Brendel. Towards the first adversarially robust neural network model on mnist. In *International Conference on Learning Representations*, 2018.
- Pierre Sermanet and Yann LeCun. Traffic sign recognition with multi-scale convolutional networks. In *The 2011 International Joint Conference on Neural Networks*, pages 2809–2813. IEEE, 2011.
- Ali Shafahi, Mahyar Najibi, Mohammad Amin Ghiasi, Zheng Xu, John Dickerson, Christoph Studer, Larry S Davis, Gavin Taylor, and Tom Goldstein. Adversarial training for free! In *Advances in Neural Information Processing Systems*, pages 3358–3369, 2019.
- Johannes Stalldkamp, Marc Schlipfing, Jan Salmen, and Christian Igel. Man vs. computer: Benchmarking machine learning algorithms for traffic sign recognition. *Neural networks*, 32:323–332, 2012.

- Thilo Strauss, Markus Hanselmann, Andrej Junginger, and Holger Ulmer. Ensemble methods as a defense to adversarial perturbations against deep neural networks. *arXiv preprint arXiv:1709.03423*, 2017.
- Christian Szegedy, Wojciech Zaremba, Ilya Sutskever, Joan Bruna, Dumitru Erhan, Ian Goodfellow, and Rob Fergus. Intriguing properties of neural networks. *arXiv preprint arXiv:1312.6199*, 2013.
- Dimitris Tsipras, Shibani Santurkar, Logan Engstrom, Alexander Turner, and Aleksander Madry. Robustness may be at odds with accuracy. In *International Conference on Learning Representations*, 2019. URL <https://openreview.net/forum?id=SyxAb30cY7>.
- Jonathan Uesato, Brendan O’donoghue, Pushmeet Kohli, and Aaron Oord. Adversarial risk and the dangers of evaluating against weak attacks. In *International Conference on Machine Learning*, pages 5025–5034. PMLR, 2018.
- Sara A van de Geer. On Hoeffding’s inequality for dependent random variables. In *Empirical process techniques for dependent data*, pages 161–169. Springer, 2002.
- Martin J Wainwright and Michael Irwin Jordan. *Graphical models, exponential families, and variational inference*. Now Publishers Inc, 2008.
- Eric Wong, Frank R Schmidt, and J Zico Kolter. Wasserstein adversarial examples via projected sinkhorn iterations. *arXiv preprint arXiv:1902.07906*, 2019.
- Tong Wu, Liang Tong, and Yevgeniy Vorobeychik. Defending against physically realizable attacks on image classification. *arXiv preprint arXiv:1909.09552*, 2019.
- Chaowei Xiao, Ruizhi Deng, Bo Li, Fisher Yu, Mingyan Liu, and Dawn Song. Characterizing adversarial examples based on spatial consistency information for semantic segmentation. In *Proceedings of the European Conference on Computer Vision (ECCV)*, pages 217–234, 2018a.
- Chaowei Xiao, Bo Li, Jun-Yan Zhu, Warren He, Mingyan Liu, and Dawn Song. Generating adversarial examples with adversarial networks. *IJCAI*, 2018b.
- Chaowei Xiao, Jun-Yan Zhu, Bo Li, Warren He, Mingyan Liu, and Dawn Song. Spatially transformed adversarial examples. In *International Conference on Learning Representations*, 2018c. URL <https://openreview.net/forum?id=HyydRMZC->.
- Huan Xu, Constantine Caramanis, and Shie Mannor. Robustness and regularization of support vector machines. *Journal of machine learning research*, 10(7), 2009.
- Weilin Xu, David Evans, and Yanjun Qi. Feature squeezing: Detecting adversarial examples in deep neural networks. *arXiv preprint arXiv:1704.01155*, 2017.
- Zhe Xu, Ivan Gavran, Yousef Ahmad, Rupak Majumdar, Daniel Neider, Ufuk Topcu, and Bo Wu. Joint inference of reward machines and policies for reinforcement learning. In *Proceedings of the International Conference on Automated Planning and Scheduling*, volume 30, pages 590–598, 2020.
- Greg Yang, Tony Duan, J Edward Hu, Hadi Salman, Ilya Razenshteyn, and Jerry Li. Randomized smoothing of all shapes and sizes. In *International Conference on Machine Learning*, pages 10693–10705. PMLR, 2020a.
- Huanrui Yang, Jingyang Zhang, Hongliang Dong, Nathan Inkawich, Andrew Gardner, Andrew Touchet, Wesley Wilkes, Heath Berry, and Hai Li. Dverge: Diversifying vulnerabilities for enhanced robust generation of ensembles. *arXiv preprint arXiv:2009.14720*, 2020b.
- Runtian Zhai, Chen Dan, Di He, Huan Zhang, Boqing Gong, Pradeep Ravikumar, Cho-Jui Hsieh, and Liwei Wang. Macer: Attack-free and scalable robust training via maximizing certified radius. In *International Conference on Learning Representations*, 2019.
- Dinghui Zhang, Mao Ye, Chengyue Gong, Zhanxing Zhu, and Qiang Liu. Black-box certification with randomized smoothing: A functional optimization based framework. *arXiv preprint arXiv:2002.09169*, 2020.

## A. Proofs

### A.1. Preliminaries

For completeness, here we recall our setup and introduce further remarks.

**Data model** We begin by recalling our notation. We consider a classification problem under supervised learning setting, defined on a feature space  $\mathcal{X}$  and a finite label space  $\mathcal{Y}$ . We refer to  $x \in \mathcal{X}$  as an input, and  $y \in \mathcal{Y}$  as the prediction. An input  $x$  can be a benign example or an adversarial example. To model this, we use  $z \in \{0, 1\}$ , a latent variable which is not exposed to KEMLP. That is,  $x$  is an adversarial example with  $(x, y) \sim \mathcal{D}_a$  whenever  $z = 1$ , and  $(x, y) \sim \mathcal{D}_b$  otherwise, where  $\mathcal{D}_a$  and  $\mathcal{D}_b$  represent the adversarial and benign data distribution. We let  $\pi_{\mathcal{D}_a} = \mathbb{P}(z = 1)$  and  $\pi_{\mathcal{D}_b} = \mathbb{P}(z = 0)$ , implying  $\pi_{\mathcal{D}_a} + \pi_{\mathcal{D}_b} = 1$ . For convenience, we denote  $\mathbb{P}_{\mathcal{D}_a}(x, y) = \mathbb{P}(x, y|z = 1)$  and  $\mathbb{P}_{\mathcal{D}_b}(x, y) = \mathbb{P}(x, y|z = 0)$ .

For simplicity, we describe the KEMLP framework as a binary classification task, in which case  $\mathcal{Y} = \{0, 1\}$ , noting that the multi-class scenario is a simple extension of it. We introduce the KEMLP framework as follows.

**Knowledge Integration** Given a data example  $(x, y) \sim \mathcal{D}_b$  or  $(x, y) \sim \mathcal{D}_a$ ,  $y$  is unknown to KEMLP. We create a factor graph to embed the domain knowledge as follows. The outputs of each model over  $x$  become *input variables*:  $s_*, s_{\mathcal{I}} = \{s_i : i \in \mathcal{I}\}, s_{\mathcal{J}} = \{s_j : j \in \mathcal{J}\}$ . KEMLP also has an output variable  $o \in \mathcal{Y}$ , which corresponds to its prediction. Different models introduce different types of factors connecting these variables:

- **Main model:** KEMLP introduces a factor between the main model  $s_*$  and the output variable  $o$  with factor function  $f_*(o, s_*) = \mathbb{1}\{o = s_*\}$ ;
- **Permissive model:** KEMLP introduces a factor between each permissive model  $s_i$  and the output variable  $o$  with factor function  $f_i(o, s_i) = \mathbb{1}\{s_i \implies o\}$ .
- **Preventative model:** KEMLP introduces a factor between each preventative model  $s_j$  and the output variable  $o$  with factor function  $f_j(o, s_j) = \mathbb{1}\{o \implies s_j\}$ .

**Learning with KEMLP** To make a prediction, KEMLP outputs the *probability* of the output variable  $o$ . KEMLP assigns a weight for each model and constructs the following log-linear statistical model:

$$\mathbb{P}[o|s_*, s_{\mathcal{I}}, s_{\mathcal{J}}, w_*, w_{\mathcal{I}}, w_{\mathcal{J}}] \propto \exp\{b_o + w_* f_*(o, s_*)\} \times \exp\left\{\sum_{i \in \mathcal{I}} w_i f_i(o, s_i)\right\} \times \exp\left\{\sum_{j \in \mathcal{J}} w_j f_j(o, s_j)\right\}$$

where  $w_*, w_i, w_j$  are the corresponding weights for models  $s_*, s_i, s_j$ ,  $w_{\mathcal{I}} = \{w_i : i \in \mathcal{I}\}, w_{\mathcal{J}} = \{w_j : j \in \mathcal{J}\}$  and  $b_o$  is some bias parameter that depends on  $o$ . For the simplicity of exposition, we use an equivalent notation by putting all the weights and outputs of factor functions into vectors using an ordering of models. More precisely, we define

$$\begin{aligned} \mathbf{w} &= [1; w_*; (w_i)_{i \in \mathcal{I}}; (w_j)_{j \in \mathcal{J}}], \\ \mathbf{f}_o(s_*, s_{\mathcal{I}}, s_{\mathcal{J}}) &= [b_o; f_*(o, s_*); (f_i(o, s_i))_{i \in \mathcal{I}}; (f_j(o, s_j))_{j \in \mathcal{J}}], \end{aligned}$$

for  $o \in \mathcal{Y}$ . All concatenated vectors from above are in  $\mathbb{R}^{m+n+2}$ . Given this, an equivalent form of KEMLP's statistical model is

$$\mathbb{P}[o|s_*, s_{\mathcal{I}}, s_{\mathcal{J}}, \mathbf{w}] = \frac{1}{Z_{\mathbf{w}}} \exp(\langle \mathbf{w}, \mathbf{f}_o(s_*, s_{\mathcal{I}}, s_{\mathcal{J}}) \rangle) \quad (4)$$

where  $Z_{\mathbf{w}}$  is the normalization constant over  $o \in \mathcal{Y}$  such that

$$Z_{\mathbf{w}} = \exp(\langle \mathbf{w}, \mathbf{f}_0(s_*, s_{\mathcal{I}}, s_{\mathcal{J}}) \rangle) + \exp(\langle \mathbf{w}, \mathbf{f}_1(s_*, s_{\mathcal{I}}, s_{\mathcal{J}}) \rangle).$$

With some abuse of notation,  $\mathbf{w}$  is meant to govern all parameters including weights and biases whenever used with probabilities.

**Weight Learning** During the training phase of KEMLP, we choose parameters  $\mathbf{w}$  by performing standard maximum likelihood estimation over a training dataset. Given a particular input instance  $x^{(n)}$ , respective model predictions  $s_*^{(n)}, s_{\mathcal{I}}^{(n)}, s_{\mathcal{J}}^{(n)}$ , and the ground truth label  $y^{(n)}$ , we minimize the negative log-likelihood function in view of

$$\hat{\mathbf{w}} = \arg \min_{\mathbf{w}} \left\{ - \sum_n \log \left( \mathbb{P}[o^{(n)} = y^{(n)} | s_*^{(n)}, s_{\mathcal{I}}^{(n)}, s_{\mathcal{J}}^{(n)}, \mathbf{w}] \right) \right\}.$$

**Inference** During the inference phase of KEMLP, given an input example  $\hat{x}$ , we predict  $\hat{y}$  that has the largest probability given the respective model predictions  $\hat{s}_*, \hat{s}_{\mathcal{I}}, \hat{s}_{\mathcal{J}}$ , namely,  $\hat{y} = \arg \max_{\tilde{y} \in \mathcal{Y}} \mathbb{P}[o = \tilde{y} | \hat{s}_*, \hat{s}_{\mathcal{I}}, \hat{s}_{\mathcal{J}}, \hat{\mathbf{w}}]$ .

**Weighted Robust Accuracy** Previous theoretical analysis on ML robustness (Javanmard et al., 2020; Xu et al., 2009; Raghunathan et al., 2020) have identified two natural dimensions of model quality: *clean accuracy* and *robust accuracy*, which are the accuracy of a given ML model on inputs  $x$  drawn from either the benign distribution  $\mathcal{D}_b$  or adversarial distribution  $\mathcal{D}_a$ . In this paper, to balance their tradeoff, we use their weighted average as our main metric of interest. That is, given a classifier  $h : \mathcal{X} \rightarrow \mathcal{Y}$  we define its *Weighted Robust Accuracy* as

$$\mathcal{A}_h = \pi_{\mathcal{D}_a} \mathbb{P}_{\mathcal{D}_a}[h(x) = y] + \pi_{\mathcal{D}_b} \mathbb{P}_{\mathcal{D}_b}[h(x) = y].$$

We use  $\mathcal{A}^{\text{KEMLP}}$  and  $\mathcal{A}^{\text{main}}$  to denote the weighted robust accuracies of KEMLP and main task model, respectively.

**Modeling Assumptions** We assume that for a fixed  $z$ , that is, for a fixed  $\mathcal{D} \in \{\mathcal{D}_b, \mathcal{D}_a\}$ , the models make independent errors given the target variable  $y$ . Thus, for all  $\mathcal{D} \in \{\mathcal{D}_b, \mathcal{D}_a\}$  the class conditional distribution can be decomposed as

$$\mathbb{P}_{\mathcal{D}}[s_*, s_{\mathcal{I}}, s_{\mathcal{J}} | y] = \mathbb{P}_{\mathcal{D}}[s_* | y] \prod_{i \in \mathcal{I}} \mathbb{P}_{\mathcal{D}}[s_i | y] \prod_{j \in \mathcal{J}} \mathbb{P}_{\mathcal{D}}[s_j | y].$$

We also assume for simplicity that the main task model makes symmetric errors given the class of target variable, that is,  $\mathbb{P}_{\mathcal{D}}[s_* \neq y | y]$  is fixed with respect to  $y$  for all  $\mathcal{D} \in \{\mathcal{D}_b, \mathcal{D}_a\}$ .

**Characterizing Models: Truth Rate ( $\alpha$ ) and False Rate ( $\epsilon$ )** Each auxiliary model  $k \in \mathcal{I} \cup \mathcal{J}$  is characterized by two values, their truth rate ( $\alpha$ ) and false rate ( $\epsilon$ ) over benign and adversarial distributions. These values measure the *consistency* of the model with the ground truth:

Permissive Models:

$$\alpha_{i,\mathcal{D}} := \mathbb{P}_{\mathcal{D}}[s_i = y | y = 1], \quad \epsilon_{i,\mathcal{D}} := \mathbb{P}_{\mathcal{D}}[s_i \neq y | y = 0]$$

Preventative Models:

$$\alpha_{j,\mathcal{D}} := \mathbb{P}_{\mathcal{D}}[s_j = y | y = 0], \quad \epsilon_{j,\mathcal{D}} := \mathbb{P}_{\mathcal{D}}[s_j \neq y | y = 1]$$

Note that, given the asymmetric nature of these auxiliary models, we do *not* necessarily have  $\epsilon_{k,\mathcal{D}} = 1 - \alpha_{k,\mathcal{D}}$ . In addition, for a high quality permissive model ( $k \in \mathcal{I}$ ), or a high quality preventative model ( $k \in \mathcal{J}$ ) for which the logic rules mostly hold, we expect  $\alpha_{k,\mathcal{D}}$  to be large and  $\epsilon_{k,\mathcal{D}}$  to be small.

We define the truth rate of main model over data examples drawn from  $\mathcal{D} \in \{\mathcal{D}_b, \mathcal{D}_a\}$  as  $\alpha_{*,\mathcal{D}} := \mathbb{P}_{\mathcal{D}}(s_* = y)$ , and its false rate as  $\epsilon_{*,\mathcal{D}} := \mathbb{P}_{\mathcal{D}}(s_* \neq y) = 1 - \alpha_{*,\mathcal{D}}$ .

These characteristics are of integral importance to weighted robust accuracy of KEMLP. To combine all the models together, we define upper and lower bounds to truth rates and false rates. For the main model, we have  $\wedge \alpha_* := \min_{\mathcal{D}} \alpha_{*,\mathcal{D}}$  and  $\vee \alpha_* := \max_{\mathcal{D}} \alpha_{*,\mathcal{D}}$ . whereas for auxiliary models, for each model index  $k \in \mathcal{I} \cup \mathcal{J}$ , we have

$$\begin{aligned} \wedge \alpha_k &:= \min_{\mathcal{D}} \alpha_{k,\mathcal{D}}, & \wedge \epsilon_k &:= \min_{\mathcal{D}} \epsilon_{k,\mathcal{D}} \\ \vee \alpha_k &:= \max_{\mathcal{D}} \alpha_{k,\mathcal{D}}, & \vee \epsilon_k &:= \max_{\mathcal{D}} \epsilon_{k,\mathcal{D}}. \end{aligned}$$

## A.2. Parameters

In this section we will derive the closed-form expressions for the parameters based on our generative model, namely, weights and biases.

To make a prediction, KEMLP outputs the *marginal probability* of the output variable  $o$ . KEMLP assigns a weight for each model and constructs the following statistical model:

$$\mathbb{P}[o|s_*, s_{\mathcal{I}}, s_{\mathcal{J}}, \mathbf{w}] \propto \exp\{b_o + w_* f_*(o, s_*)\} \times \exp\left\{\sum_{i \in \mathcal{I}} w_i f_i(o, s_i)\right\} \times \exp\left\{\sum_{j \in \mathcal{J}} w_j f_j(o, s_j)\right\},$$

where  $w_*, w_i, w_j$  are the corresponding weights for models  $s_*, s_i, s_j$ , and  $b_o$  is some bias parameter that depends on  $o$ . For the simplicity of exposition, we use an equivalent notation by putting all the weights and outputs of factor functions into vectors using an ordering of models. More precisely, we define

$$\begin{aligned} \mathbf{w} &= [1; w_*; (w_i)_{i \in \mathcal{I}}; (w_j)_{j \in \mathcal{J}}], \\ \mathbf{f}_o(s_*, s_{\mathcal{I}}, s_{\mathcal{J}}) &= [b_o; f_*(o, s_*); (f_i(o, s_i))_{i \in \mathcal{I}}; (f_j(o, s_j))_{j \in \mathcal{J}}], \end{aligned}$$

for  $o \in \mathcal{Y}$ . All concatenated vectors from above are in  $\mathbb{R}^{m+n+2}$ . Given this, an equivalent form of KEMLP's statistical model is

$$\mathbb{P}[o|s_*, s_{\mathcal{I}}, s_{\mathcal{J}}, \mathbf{w}] = \frac{1}{Z_{\mathbf{w}}} \exp(\langle \mathbf{w}, \mathbf{f}_o(s_*, s_{\mathcal{I}}, s_{\mathcal{J}}) \rangle), \quad (5)$$

where  $Z_{\mathbf{w}}$  is the normalization constant over  $o \in \mathcal{Y}$ . We can further show that

$$\begin{aligned} \mathbb{P}[o = \tilde{y}|s_*, s_{\mathcal{I}}, s_{\mathcal{J}}, \mathbf{w}] &= \frac{\mathbb{P}[o = \tilde{y}|s_*, s_{\mathcal{I}}, s_{\mathcal{J}}, \mathbf{w}]}{\mathbb{P}[o = \tilde{y}|s_*, s_{\mathcal{I}}, s_{\mathcal{J}}, \mathbf{w}] + \mathbb{P}[o = 1 - \tilde{y}|s_*, s_{\mathcal{I}}, s_{\mathcal{J}}, \mathbf{w}]} \\ &= \frac{\exp(\langle \mathbf{w}, \mathbf{f}_{\tilde{y}}(s_*, s_{\mathcal{I}}, s_{\mathcal{J}}) \rangle)}{\exp(\langle \mathbf{w}, \mathbf{f}_{\tilde{y}}(s_*, s_{\mathcal{I}}, s_{\mathcal{J}}) \rangle) + \exp(\langle \mathbf{w}, \mathbf{f}_{1-\tilde{y}}(s_*, s_{\mathcal{I}}, s_{\mathcal{J}}) \rangle)} \\ &= \frac{1}{1 + \exp(-\Delta_{\mathbf{w}}(\tilde{y}, s_*, s_{\mathcal{I}}, s_{\mathcal{J}}))} \end{aligned} \quad (6)$$

where  $\Delta_{\mathbf{w}}(\tilde{y}, s_*, s_{\mathcal{I}}, s_{\mathcal{J}})$  is previously defined as

$$\Delta_{\mathbf{w}}(\tilde{y}, s_*, s_{\mathcal{I}}, s_{\mathcal{J}}) := \langle \mathbf{w}, \mathbf{f}_{\tilde{y}}(s_*, s_{\mathcal{I}}, s_{\mathcal{J}}) - \mathbf{f}_{1-\tilde{y}}(s_*, s_{\mathcal{I}}, s_{\mathcal{J}}) \rangle.$$

Therefore, we have

$$\mathbb{P}[o = \tilde{y}|s_*, s_{\mathcal{I}}, s_{\mathcal{J}}, \mathbf{w}] = \sigma(\Delta_{\mathbf{w}}(\tilde{y}, s_*, s_{\mathcal{I}}, s_{\mathcal{J}})) \quad (7)$$

where  $\sigma : \mathbb{R} \mapsto [0, 1]$  is the Sigmoid function.

**Remark 1** (Closed form expression of  $\Delta_{\mathbf{w}}(\tilde{y}, s_*, s_{\mathcal{I}}, s_{\mathcal{J}})$ ). *Recalling our knowledge integration rules, it can be shown that*

$$\begin{aligned} \Delta_{\mathbf{w}}(\tilde{y}, s_*, s_{\mathcal{I}}, s_{\mathcal{J}}) &= \langle \mathbf{w}, \mathbf{f}_{\tilde{y}}(s_*, s_{\mathcal{I}}, s_{\mathcal{J}}) - \mathbf{f}_{1-\tilde{y}}(s_*, s_{\mathcal{I}}, s_{\mathcal{J}}) \rangle \\ &= b(\tilde{y}) + w_* (f_*(\tilde{y}, s_*) - f_*(1 - \tilde{y}, s_*)) + \sum_{i \in \mathcal{I}} w_i (f_i(\tilde{y}, s_i) - f_i(1 - \tilde{y}, s_i)) \\ &\quad + \sum_{j \in \mathcal{J}} w_j (f_j(\tilde{y}, s_j) - f_j(1 - \tilde{y}, s_j)) \end{aligned}$$

where  $b(\tilde{y}) = b_{\tilde{y}} - b_{1-\tilde{y}}$ . Let  $b := b_1 - b_0$ . Then  $b(\tilde{y}) = (2\tilde{y} - 1)b$ .

Using the logical rules, we moreover have

$$\begin{aligned} f_*(\tilde{y}, s_*) - f_*(1 - \tilde{y}, s_*) &= \mathbb{1}\{\tilde{y} = s_*\} - \mathbb{1}\{1 - \tilde{y} = s_*\} = (2\tilde{y} - 1)(2s_* - 1) \\ f_i(\tilde{y}, s_i) - f_i(1 - \tilde{y}, s_i) &= \mathbb{1}\{s_i \implies \tilde{y}\} - \mathbb{1}\{s_i \implies 1 - \tilde{y}\} = (2\tilde{y} - 1)s_i \\ f_j(\tilde{y}, s_j) - f_j(1 - \tilde{y}, s_j) &= \mathbb{1}\{\tilde{y} \implies s_j\} - \mathbb{1}\{1 - \tilde{y} \implies s_j\} = (2\tilde{y} - 1)(s_j - 1) = -(2\tilde{y} - 1)(1 - s_j). \end{aligned}$$

Therefore, the closed form expression for  $\Delta_{\mathbf{w}}(\tilde{y}, s_*, s_{\mathcal{I}}, s_{\mathcal{J}})$  is given by

$$\Delta_{\mathbf{w}}(\tilde{y}, s_*, s_{\mathcal{I}}, s_{\mathcal{J}}) = (2\tilde{y} - 1) \left( b + w_* (2s_* - 1) + \sum_{i \in \mathcal{I}} w_i s_i - \sum_{j \in \mathcal{J}} w_j (1 - s_j) \right)$$

**Remark 2** (Optimal parameters). *We now analyze the class conditional distribution  $\mathbb{P}[y|s_*, s_{\mathcal{I}}, s_{\mathcal{J}}]$ . Optimal set of parameters for our generative model must satisfy:*

$$\begin{aligned} \mathbb{P}[y = \tilde{y}|s_*, s_{\mathcal{I}}, s_{\mathcal{J}}] &= \frac{\mathbb{P}[y = \tilde{y}, s_*, s_{\mathcal{I}}, s_{\mathcal{J}}]}{\mathbb{P}[s_*, s_{\mathcal{I}}, s_{\mathcal{J}}]} = \frac{\mathbb{P}[y = \tilde{y}, s_*, s_{\mathcal{I}}, s_{\mathcal{J}}]}{\mathbb{P}[y = \tilde{y}, s_*, s_{\mathcal{I}}, s_{\mathcal{J}}] + \mathbb{P}[y = 1 - \tilde{y}, s_*, s_{\mathcal{I}}, s_{\mathcal{J}}]} \\ &= \frac{1}{1 + \frac{\mathbb{P}[y=1-\tilde{y}, s_*, s_{\mathcal{I}}, s_{\mathcal{J}}]}{\mathbb{P}[y=\tilde{y}, s_*, s_{\mathcal{I}}, s_{\mathcal{J}}]}} = \frac{1}{1 + \exp\left(\log \frac{\mathbb{P}[y=1-\tilde{y}, s_*, s_{\mathcal{I}}, s_{\mathcal{J}}]}{\mathbb{P}[y=\tilde{y}, s_*, s_{\mathcal{I}}, s_{\mathcal{J}}]}\right)} = \frac{1}{1 + \exp\left(-\log \frac{\mathbb{P}[y=\tilde{y}, s_*, s_{\mathcal{I}}, s_{\mathcal{J}}]}{\mathbb{P}[y=1-\tilde{y}, s_*, s_{\mathcal{I}}, s_{\mathcal{J}}]}\right)}. \end{aligned} \quad (8)$$

Note that, the optimal parameters satisfy

$$\mathbb{P}[o = \tilde{y}|s_*, s_{\mathcal{I}}, s_{\mathcal{J}}] = \mathbb{P}[y = \tilde{y}|s_*, s_{\mathcal{I}}, s_{\mathcal{J}}].$$

Hence, combining (6) and (8) as well as Remark 1 we further have

$$\log \frac{\mathbb{P}[y = \tilde{y}, s_*, s_{\mathcal{I}}, s_{\mathcal{J}}]}{\mathbb{P}[y = 1 - \tilde{y}, s_*, s_{\mathcal{I}}, s_{\mathcal{J}}]} = (2\tilde{y} - 1) \left( b + w_*(2s_* - 1) + \sum_{i \in \mathcal{I}} w_i s_i - \sum_{j \in \mathcal{J}} w_j (1 - s_j) \right). \quad (9)$$

Above remark indicates the condition that the optimal parameters must satisfy.

### A.3. Proof of Lemma 1

Recall that for each model index  $k \in \mathcal{I} \cup \mathcal{J}$  we define upper and lower bounds to truth rates and false rates as

$$\begin{aligned} \wedge \alpha_k &:= \min_{\mathcal{D}} \alpha_{k, \mathcal{D}}, & \wedge \epsilon_k &:= \min_{\mathcal{D}} \epsilon_{k, \mathcal{D}} \\ \vee \alpha_k &:= \max_{\mathcal{D}} \alpha_{k, \mathcal{D}}, & \vee \epsilon_k &:= \max_{\mathcal{D}} \epsilon_{k, \mathcal{D}}. \end{aligned}$$

Next, we revisit Lemma 1 towards its proof.

**Lemma** (Recall). *Let  $\Delta_{\mathbf{w}}$  be a random variable defined above. Suppose that KEMLP uses optimal parameters  $\mathbf{w}$  such that  $\mathbb{P}[y|s_*, s_{\mathcal{I}}, s_{\mathcal{J}}] = \mathbb{P}[o|s_*, s_{\mathcal{I}}, s_{\mathcal{J}}, \mathbf{w}]$ . Let also  $r_y$  denote the log-ratio of class imbalance  $\log \frac{\mathbb{P}[y=1]}{\mathbb{P}[y=0]}$ . For a fixed  $y \in \mathcal{Y}$  and  $\mathcal{D} \in \{\mathcal{D}_b, \mathcal{D}_a\}$ , one has*

$$\mathbb{E}_{s_*, s_{\mathcal{I}}, s_{\mathcal{J}}} [\Delta_{\mathbf{w}}(y, s_*, s_{\mathcal{I}}, s_{\mathcal{J}}) | y] \geq \mu_{d_*, \mathcal{D}} + y \mu_{d_{\mathcal{I}}, \mathcal{D}} + (1 - y) \mu_{d_{\mathcal{J}}, \mathcal{D}} + (2y - 1) r_y := \mu_{y, \mathcal{D}},$$

where

$$\begin{aligned} \mu_{d_*, \mathcal{D}} &= \alpha_{*, \mathcal{D}} \log \frac{\wedge \alpha_*}{1 - \wedge \alpha_*} + (1 - \alpha_{*, \mathcal{D}}) \log \frac{1 - \vee \alpha_*}{\vee \alpha_*}, \\ \mu_{d_{\mathcal{I}}, \mathcal{D}} &= \sum_{i \in \mathcal{I}} \alpha_{i, \mathcal{D}} \log \frac{\wedge \alpha_i}{\vee \epsilon_i} + (1 - \alpha_{i, \mathcal{D}}) \log \frac{1 - \vee \alpha_i}{1 - \wedge \epsilon_i} - \sum_{j \in \mathcal{J}} \epsilon_{j, \mathcal{D}} \log \frac{\vee \alpha_j}{\wedge \epsilon_j} - (1 - \epsilon_{j, \mathcal{D}}) \log \frac{1 - \wedge \alpha_j}{1 - \vee \epsilon_j}, \end{aligned}$$

and

$$\mu_{d_{\mathcal{J}}, \mathcal{D}} = \sum_{j \in \mathcal{J}} \alpha_{j, \mathcal{D}} \log \frac{\wedge \alpha_j}{\vee \epsilon_j} + (1 - \alpha_{j, \mathcal{D}}) \log \frac{1 - \vee \alpha_j}{1 - \wedge \epsilon_j} - \sum_{i \in \mathcal{I}} \epsilon_{i, \mathcal{D}} \log \frac{\vee \alpha_i}{\wedge \epsilon_i} - (1 - \epsilon_{i, \mathcal{D}}) \log \frac{1 - \wedge \alpha_i}{1 - \vee \epsilon_i}.$$

*Proof of Lemma 1.* We show earlier that the optimal parameters satisfy (9). Note that the probabilities on the left hand side of (9) are mixtures over both the benign and adversarial distributions. Namely,

$$\mathbb{P}[y = \tilde{y}, s_*, s_{\mathcal{I}}, s_{\mathcal{J}}] = \sum_{\mathcal{D} \in \{\mathcal{D}_b, \mathcal{D}_a\}} \pi_{\mathcal{D}} \mathbb{P}_{\mathcal{D}}[y = \tilde{y}, s_*, s_{\mathcal{I}}, s_{\mathcal{J}}].$$

Recall from our modeling assumptions that models are conditionally independent given  $y$  with  $\mathbb{P}_{\mathcal{D}}[s_*, s_{\mathcal{I}}, s_{\mathcal{J}} | y = \tilde{y}] = \mathbb{P}_{\mathcal{D}}[s_* | y = \tilde{y}] \prod_{i \in \mathcal{I}} \mathbb{P}_{\mathcal{D}}[s_i | y = \tilde{y}] \prod_{j \in \mathcal{J}} \mathbb{P}_{\mathcal{D}}[s_j | y = \tilde{y}]$ . Therefore, without loss of generality, this holds not for  $\mathbb{P}[y = \tilde{y}, s_*, s_{\mathcal{I}}, s_{\mathcal{J}}]$ . That is, each parameter is to encode this dependency structure and must be a function of some set of models. Below we propose a strategy to choose optimal weights to satisfy (9).

We start by decomposing  $\log \frac{\mathbb{P}[y=\tilde{y}, s_*, s_{\mathcal{I}}, s_{\mathcal{J}}]}{\mathbb{P}[y=1-\tilde{y}, s_*, s_{\mathcal{I}}, s_{\mathcal{J}}]}$ .

$$\log \frac{\mathbb{P}[y = \tilde{y}, s_*, s_{\mathcal{I}}, s_{\mathcal{J}}]}{\mathbb{P}[y = 1 - \tilde{y}, s_*, s_{\mathcal{I}}, s_{\mathcal{J}}]} = \log \frac{\mathbb{P}[y = \tilde{y}, s_*]}{\mathbb{P}[y = 1 - \tilde{y}, s_*]} + \sum_{i \in \mathcal{I}} \log \frac{\mathbb{P}[s_i | y = \tilde{y}, s_{I_i}]}{\mathbb{P}[s_i | y = 1 - \tilde{y}, s_{I_i}]} + \sum_{j \in \mathcal{J}} \log \frac{\mathbb{P}[s_j | y = \tilde{y}, s_{I_j}]}{\mathbb{P}[s_j | y = 1 - \tilde{y}, s_{I_j}, s_{J_j}]}$$

where  $I_i$  is the set of  $i'$  such that  $i' \in \mathcal{I}$  and  $i' < i$ . Similarly, we let  $J_j$  be the set of  $j'$  such that  $j' \in \mathcal{J}$  and  $j' < j$ . Note that there are multiple such constructions to satisfy (9) to have optimal set of weights.

We split our proof into three main steps as follows.

**Step 1: Derivation of bounds for optimal set of parameters** Given our strategy, we then derive the parameters in terms of conditional probabilities of individual models. Towards that, let  $b$  be decomposed into its additive components such that  $b = b_* + \sum_{i \in \mathcal{I}} b_i - \sum_{j \in \mathcal{J}} b_j$ . Let also  $r_y = \log \frac{\mathbb{P}[y=1]}{\mathbb{P}[y=0]}$ . We derive bounds for each sensor using (9) as follows.

• *Main task model:* The parameters for the main model simply satisfies

$$(2\tilde{y} - 1)(w_*(2s_* - 1) + b_*) = \log \frac{\mathbb{P}[y = \tilde{y}, s_*]}{\mathbb{P}[y = 1 - \tilde{y}, s_*]} = \log \frac{\sum_{\mathcal{D} \in \{\mathcal{D}_b, \mathcal{D}_a\}} \pi_{\mathcal{D}} \mathbb{P}_{\mathcal{D}}[y = \tilde{y}, s_*]}{\sum_{\mathcal{D} \in \{\mathcal{D}_b, \mathcal{D}_a\}} \pi_{\mathcal{D}} \mathbb{P}_{\mathcal{D}}[y = 1 - \tilde{y}, s_*]}.$$

With a simple algebraic manipulation where  $y = 1$  and  $s_* = 1$  (resp. for  $y = 0$ ,  $s_* = 1$ ), we have that

$$w_* + b_* = \log \frac{\mathbb{P}[y = 1, s_* = 1]}{\mathbb{P}[y = 0, s_* = 1]} \quad (10)$$

and for  $y = 0$  and  $s_* = 0$  (resp. for  $y = 1$ ,  $s_* = 0$ )

$$w_* - b_* = \log \frac{\mathbb{P}[y = 0, s_* = 0]}{\mathbb{P}[y = 1, s_* = 0]}. \quad (11)$$

Combining (10) and (11) we have

$$\begin{aligned} w_* &= \frac{1}{2} \log \frac{\mathbb{P}[y = 1, s_* = 1] \mathbb{P}[y = 0, s_* = 0]}{\mathbb{P}[y = 0, s_* = 1] \mathbb{P}[y = 1, s_* = 0]} \\ &\stackrel{(*)}{=} \frac{1}{2} \log \frac{(\sum_{\mathcal{D} \in \{\mathcal{D}_b, \mathcal{D}_a\}} \pi_{\mathcal{D}} \mathbb{P}_{\mathcal{D}}[y = 1] \alpha_{*, \mathcal{D}}) (\sum_{\mathcal{D} \in \{\mathcal{D}_b, \mathcal{D}_a\}} \pi_{\mathcal{D}} \mathbb{P}_{\mathcal{D}}[y = 0] \alpha_{*, \mathcal{D}})}{(\sum_{\mathcal{D} \in \{\mathcal{D}_b, \mathcal{D}_a\}} \pi_{\mathcal{D}} \mathbb{P}_{\mathcal{D}}[y = 1] (1 - \alpha_{*, \mathcal{D}})) (\sum_{\mathcal{D} \in \{\mathcal{D}_b, \mathcal{D}_a\}} \pi_{\mathcal{D}} \mathbb{P}_{\mathcal{D}}[y = 0] (1 - \alpha_{*, \mathcal{D}}))} \end{aligned} \quad (12)$$

where (\*) follows from that  $\mathbb{P}_{\mathcal{D}}[y = s_* | y] = \alpha_{*, \mathcal{D}}$  and  $\mathbb{P}_{\mathcal{D}}[y \neq s_* | y] = 1 - \alpha_{*, \mathcal{D}}$  for  $\mathcal{D} \in \{\mathcal{D}_b, \mathcal{D}_a\}$ .

Similarly, for  $b_*$  we have

$$\begin{aligned} b_* &= \frac{1}{2} \log \frac{\mathbb{P}[y = 1, s_* = 1] \mathbb{P}[y = 1, s_* = 0]}{\mathbb{P}[y = 0, s_* = 1] \mathbb{P}[y = 0, s_* = 0]} \\ &= \frac{1}{2} \log \frac{(\sum_{\mathcal{D} \in \{\mathcal{D}_b, \mathcal{D}_a\}} \pi_{\mathcal{D}} \mathbb{P}_{\mathcal{D}}[y = 1] \alpha_{*, \mathcal{D}}) (\sum_{\mathcal{D} \in \{\mathcal{D}_b, \mathcal{D}_a\}} \pi_{\mathcal{D}} \mathbb{P}_{\mathcal{D}}[y = 1] (1 - \alpha_{*, \mathcal{D}}))}{(\sum_{\mathcal{D} \in \{\mathcal{D}_b, \mathcal{D}_a\}} \pi_{\mathcal{D}} \mathbb{P}_{\mathcal{D}}[y = 0] (1 - \alpha_{*, \mathcal{D}})) (\sum_{\mathcal{D} \in \{\mathcal{D}_b, \mathcal{D}_a\}} \pi_{\mathcal{D}} \mathbb{P}_{\mathcal{D}}[y = 0] \alpha_{*, \mathcal{D}})}. \end{aligned} \quad (13)$$

Finally, noting that, for all  $\tilde{y} \in \mathcal{Y}$ , we have

$$\wedge \alpha_* \sum_{\mathcal{D} \in \{\mathcal{D}_b, \mathcal{D}_a\}} \pi_{\mathcal{D}} \mathbb{P}_{\mathcal{D}}[y = \tilde{y}] = \wedge \alpha_* \mathbb{P}[y = \tilde{y}] \leq \sum_{\mathcal{D} \in \{\mathcal{D}_b, \mathcal{D}_a\}} \pi_{\mathcal{D}} \mathbb{P}_{\mathcal{D}}[y = \tilde{y}] \alpha_{*, \mathcal{D}} \leq \vee \alpha_* \sum_{\mathcal{D} \in \{\mathcal{D}_b, \mathcal{D}_a\}} \pi_{\mathcal{D}} \mathbb{P}_{\mathcal{D}}[y = \tilde{y}] = \vee \alpha_* \mathbb{P}[y = \tilde{y}].$$

Using the above relation as well as (12) and (13), the weight and bias of the main task model,  $w_*$  and  $b_*$ , can therefore be bounded as

$$\log \frac{\wedge \alpha_*}{1 - \wedge \alpha_*} \leq w_* \leq \log \frac{\vee \alpha_*}{1 - \vee \alpha_*} \quad (14)$$

and

$$r_y + \log \frac{\wedge \alpha_* (1 - \vee \alpha_*)}{(1 - \wedge \alpha_*) \vee \alpha_*} \leq b_* \leq r_y + \log \frac{\vee \alpha_* (1 - \wedge \alpha_*)}{(1 - \vee \alpha_*) \wedge \alpha_*}. \quad (15)$$

To distinguish the effect of class imbalance in our analysis, we will define  $b_{**} := b_* - r_y$ .

- *Permissive models*: For permissive model, we have

$$\log \frac{\mathbb{P}[s_i|y = \tilde{y}, s_{I_i}]}{\mathbb{P}[s_i|y = 1 - \tilde{y}, s_{I_i}]} = (2\tilde{y} - 1)(w_i s_i + b_i).$$

Therefore

$$\log \frac{\mathbb{P}[s_i|y = \tilde{y}, s_{I_i}]}{\mathbb{P}[s_i|y = 1 - \tilde{y}, s_{I_i}]} = \log \frac{\frac{\mathbb{P}[s_i, y = \tilde{y}, s_{I_i}]}{\mathbb{P}[y = \tilde{y}, s_{I_i}]}}{\frac{\mathbb{P}[s_i, y = 1 - \tilde{y}, s_{I_i}]}{\mathbb{P}[y = 1 - \tilde{y}, s_{I_i}]}} \stackrel{(*)}{=} \log \frac{\frac{\sum_{\mathcal{D} \in \{\mathcal{D}_b, \mathcal{D}_a\}} \pi_{\mathcal{D}} \mathbb{P}_{\mathcal{D}}[y = \tilde{y}, s_{I_i}] \mathbb{P}_{\mathcal{D}}[s_i|y = \tilde{y}]}{\sum_{\mathcal{D} \in \{\mathcal{D}_b, \mathcal{D}_a\}} \pi_{\mathcal{D}} \mathbb{P}_{\mathcal{D}}[y = \tilde{y}, s_{I_i}]}}{\frac{\sum_{\mathcal{D} \in \{\mathcal{D}_b, \mathcal{D}_a\}} \pi_{\mathcal{D}} \mathbb{P}_{\mathcal{D}}[y = 1 - \tilde{y}, s_{I_i}] \mathbb{P}_{\mathcal{D}}[s_i|y = 1 - \tilde{y}]}{\sum_{\mathcal{D} \in \{\mathcal{D}_b, \mathcal{D}_a\}} \pi_{\mathcal{D}} \mathbb{P}_{\mathcal{D}}[y = 1 - \tilde{y}, s_{I_i}]}}$$

where (\*) follows from the conditional independence assumption.

Let  $\tilde{y} = 1$ . Therefore, for  $s_i = 1$  we have

$$\min_{\mathcal{D}} \alpha_{i, \mathcal{D}} = \wedge \alpha_i \leq \frac{\sum_{\mathcal{D} \in \{\mathcal{D}_b, \mathcal{D}_a\}} \pi_{\mathcal{D}} \mathbb{P}_{\mathcal{D}}[y = \tilde{y}, s_{I_i}] \mathbb{P}_{\mathcal{D}}[s_i|y = \tilde{y}]}{\sum_{\mathcal{D} \in \{\mathcal{D}_b, \mathcal{D}_a\}} \pi_{\mathcal{D}} \mathbb{P}_{\mathcal{D}}[y = \tilde{y}, s_{I_i}]} \leq \max_{\mathcal{D}} \alpha_{i, \mathcal{D}} = \vee \alpha_i$$

and

$$\min_{\mathcal{D}} \epsilon_{i, \mathcal{D}} = \wedge \epsilon_i \leq \frac{\sum_{\mathcal{D} \in \{\mathcal{D}_b, \mathcal{D}_a\}} \pi_{\mathcal{D}} \mathbb{P}_{\mathcal{D}}[y = 1 - \tilde{y}, s_{I_i}] \mathbb{P}_{\mathcal{D}}[s_i|y = 1 - \tilde{y}]}{\sum_{\mathcal{D} \in \{\mathcal{D}_b, \mathcal{D}_a\}} \pi_{\mathcal{D}} \mathbb{P}_{\mathcal{D}}[y = 1 - \tilde{y}, s_{I_i}]} \leq \max_{\mathcal{D}} \epsilon_{i, \mathcal{D}} = \vee \epsilon_i.$$

Above bounds finally lead to

$$\log \frac{\wedge \alpha_i}{\vee \epsilon_i} \leq \log \frac{\mathbb{P}[s_i|y = \tilde{y}, s_{I_i}]}{\mathbb{P}[s_i|y = 1 - \tilde{y}, s_{I_i}]} = w_i + b_i \leq \log \frac{\vee \alpha_i}{\wedge \epsilon_i}. \quad (16)$$

Next, we let  $s_i = 0$ . Repeating the same technique above, we have

$$\min_{\mathcal{D}} 1 - \alpha_{i, \mathcal{D}} = 1 - \vee \alpha_i \leq \frac{\sum_{\mathcal{D} \in \{\mathcal{D}_b, \mathcal{D}_a\}} \pi_{\mathcal{D}} \mathbb{P}_{\mathcal{D}}[y = \tilde{y}, s_{I_i}] \mathbb{P}_{\mathcal{D}}[s_i|y = \tilde{y}]}{\sum_{\mathcal{D} \in \{\mathcal{D}_b, \mathcal{D}_a\}} \pi_{\mathcal{D}} \mathbb{P}_{\mathcal{D}}[y = \tilde{y}, s_{I_i}]} \leq \max_{\mathcal{D}} 1 - \alpha_{i, \mathcal{D}} = 1 - \wedge \alpha_i$$

and

$$\min_{\mathcal{D}} 1 - \epsilon_{i, \mathcal{D}} = 1 - \vee \epsilon_i \leq \frac{\sum_{\mathcal{D} \in \{\mathcal{D}_b, \mathcal{D}_a\}} \pi_{\mathcal{D}} \mathbb{P}_{\mathcal{D}}[y = 1 - \tilde{y}, s_{I_i}] \mathbb{P}_{\mathcal{D}}[s_i|y = 1 - \tilde{y}]}{\sum_{\mathcal{D} \in \{\mathcal{D}_b, \mathcal{D}_a\}} \pi_{\mathcal{D}} \mathbb{P}_{\mathcal{D}}[y = 1 - \tilde{y}, s_{I_i}]} \leq \max_{\mathcal{D}} 1 - \epsilon_{i, \mathcal{D}} = 1 - \wedge \epsilon_i.$$

Above bounds finally lead to

$$\log \frac{1 - \vee \alpha_i}{1 - \wedge \epsilon_i} \leq \log \frac{\mathbb{P}[s_i|y = \tilde{y}, s_{I_i}]}{\mathbb{P}[s_i|y = 1 - \tilde{y}, s_{I_i}]} = b_i \leq \log \frac{1 - \wedge \alpha_i}{1 - \vee \epsilon_i}. \quad (17)$$

Note that the same conclusion can be drawn for  $\tilde{y} = 0$ .

- *Preventative models*: For preventative model, we have

$$\log \frac{\mathbb{P}[s_j|y = \tilde{y}, s_I, s_{J_j}]}{\mathbb{P}[s_j|y = 1 - \tilde{y}, s_I, s_{J_j}]} = -(2\tilde{y} - 1)(w_j(1 - s_j) + b_j).$$

Then

$$\log \frac{\mathbb{P}[s_j|y = \tilde{y}, s_I, s_{J_j}]}{\mathbb{P}[s_j|y = 1 - \tilde{y}, s_I, s_{J_j}]} = \log \frac{\frac{\mathbb{P}[s_j, y = \tilde{y}, s_I, s_{J_j}]}{\mathbb{P}[y = \tilde{y}, s_I, s_{J_j}]}}{\frac{\mathbb{P}[s_j, y = 1 - \tilde{y}, s_I, s_{J_j}]}{\mathbb{P}[y = 1 - \tilde{y}, s_I, s_{J_j}]}} \stackrel{(*)}{=} \log \frac{\frac{\sum_{\mathcal{D} \in \{\mathcal{D}_b, \mathcal{D}_a\}} \pi_{\mathcal{D}} \mathbb{P}_{\mathcal{D}}[y = \tilde{y}, s_I, s_{J_j}] \mathbb{P}_{\mathcal{D}}[s_j|y = \tilde{y}]}{\sum_{\mathcal{D} \in \{\mathcal{D}_b, \mathcal{D}_a\}} \pi_{\mathcal{D}} \mathbb{P}_{\mathcal{D}}[y = \tilde{y}, s_I, s_{J_j}]}}{\frac{\sum_{\mathcal{D} \in \{\mathcal{D}_b, \mathcal{D}_a\}} \pi_{\mathcal{D}} \mathbb{P}_{\mathcal{D}}[y = 1 - \tilde{y}, s_I, s_{J_j}] \mathbb{P}_{\mathcal{D}}[s_j|y = 1 - \tilde{y}]}{\sum_{\mathcal{D} \in \{\mathcal{D}_b, \mathcal{D}_a\}} \pi_{\mathcal{D}} \mathbb{P}_{\mathcal{D}}[y = 1 - \tilde{y}, s_I, s_{J_j}]}}$$

where (\*) follows from the conditional independence assumption.

Let  $\tilde{y} = 0$ . Therefore, for  $s_j = 0$  we have

$$\min_{\mathcal{D}} \alpha_{j,\mathcal{D}} = \wedge \alpha_j \leq \frac{\sum_{\mathcal{D} \in \{\mathcal{D}_b, \mathcal{D}_a\}} \pi_{\mathcal{D}} \mathbb{P}_{\mathcal{D}}[y = \tilde{y}, s_I, s_{J_j}] \mathbb{P}_{\mathcal{D}}[s_j | y = \tilde{y}]}{\sum_{\mathcal{D} \in \{\mathcal{D}_b, \mathcal{D}_a\}} \pi_{\mathcal{D}} \mathbb{P}_{\mathcal{D}}[y = \tilde{y}, s_I, s_{J_j}]} \leq \max_{\mathcal{D}} \alpha_{j,\mathcal{D}} = \vee \alpha_j$$

and

$$\min_{\mathcal{D}} \epsilon_{j,\mathcal{D}} = \wedge \epsilon_j \leq \frac{\sum_{\mathcal{D} \in \{\mathcal{D}_b, \mathcal{D}_a\}} \pi_{\mathcal{D}} \mathbb{P}_{\mathcal{D}}[y = 1 - \tilde{y}, s_I, s_{J_j}] \mathbb{P}_{\mathcal{D}}[s_j | y = 1 - \tilde{y}]}{\sum_{\mathcal{D} \in \{\mathcal{D}_b, \mathcal{D}_a\}} \pi_{\mathcal{D}} \mathbb{P}_{\mathcal{D}}[y = 1 - \tilde{y}, s_I, s_{J_j}]} \leq \max_{\mathcal{D}} \epsilon_{j,\mathcal{D}} = \vee \epsilon_j.$$

Above bounds finally lead to

$$\log \frac{\wedge \alpha_j}{\vee \epsilon_j} \leq \log \frac{\mathbb{P}[s_j | y = \tilde{y}, s_I, s_{J_j}]}{\mathbb{P}[s_j | y = 1 - \tilde{y}, s_I, s_{J_j}]} = w_j + b_j \leq \log \frac{\vee \alpha_j}{\wedge \epsilon_j}. \quad (18)$$

Next, we let  $s_j = 1$ . Repeating the same technique above, we have

$$\min_{\mathcal{D}} 1 - \alpha_{j,\mathcal{D}} = 1 - \vee \alpha_j \leq \frac{\sum_{\mathcal{D} \in \{\mathcal{D}_b, \mathcal{D}_a\}} \pi_{\mathcal{D}} \mathbb{P}_{\mathcal{D}}[y = \tilde{y}, s_I, s_{J_j}] \mathbb{P}_{\mathcal{D}}[s_j | y = \tilde{y}]}{\sum_{\mathcal{D} \in \{\mathcal{D}_b, \mathcal{D}_a\}} \pi_{\mathcal{D}} \mathbb{P}_{\mathcal{D}}[y = \tilde{y}, s_I, s_{J_j}]} \leq \max_{\mathcal{D}} 1 - \alpha_{j,\mathcal{D}} = 1 - \wedge \alpha_j$$

and

$$\min_{\mathcal{D}} 1 - \epsilon_{j,\mathcal{D}} = 1 - \vee \epsilon_j \leq \frac{\sum_{\mathcal{D} \in \{\mathcal{D}_b, \mathcal{D}_a\}} \pi_{\mathcal{D}} \mathbb{P}_{\mathcal{D}}[y = 1 - \tilde{y}, s_I, s_{J_j}] \mathbb{P}_{\mathcal{D}}[s_j | y = 1 - \tilde{y}]}{\sum_{\mathcal{D} \in \{\mathcal{D}_b, \mathcal{D}_a\}} \pi_{\mathcal{D}} \mathbb{P}_{\mathcal{D}}[y = 1 - \tilde{y}, s_I, s_{J_j}]} \leq \max_{\mathcal{D}} 1 - \epsilon_{j,\mathcal{D}} = 1 - \wedge \epsilon_j.$$

Similarly as in permissive models, above bounds lead to

$$\log \frac{1 - \vee \alpha_j}{1 - \wedge \epsilon_j} \leq \log \frac{\mathbb{P}[s_j | y = \tilde{y}, s_I, s_{J_j}]}{\mathbb{P}[s_j | y = 1 - \tilde{y}, s_I, s_{J_j}]} = b_j \leq \log \frac{1 - \wedge \alpha_j}{1 - \vee \epsilon_j}. \quad (19)$$

The same conclusion can be drawn for  $\tilde{y} = 1$ .

**Step 2: Decomposition of  $\Delta_{\mathbf{w}}(y, s_*, s_{\mathcal{I}}, s_{\mathcal{J}})$**  Next, we recall Remark 1 and present a lower bound for  $\Delta_{\mathbf{w}}(y, s_*, s_{\mathcal{I}}, s_{\mathcal{J}})$  that decomposes  $\Delta_{\mathbf{w}}(y, s_*, s_{\mathcal{I}}, s_{\mathcal{J}})$  into its additive components such that

$$\begin{aligned} \Delta_{\mathbf{w}}(y, s_*, s_{\mathcal{I}}, s_{\mathcal{J}}) &= (2\tilde{y} - 1) \left( b + w_*(2s_* - 1) + \sum_{i \in \mathcal{I}} w_i s_i - \sum_{j \in \mathcal{J}} w_j (1 - s_j) \right) \\ &= (2\tilde{y} - 1) \left( w_*(2s_* - 1) + \sum_{i \in \mathcal{I}} (w_i s_i + b_i) - \sum_{j \in \mathcal{J}} (w_j (1 - s_j) + b_j) \right). \end{aligned}$$

Next, we analyze

$$\mathbb{P}_{\mathcal{D}}[\langle \mathbf{w}, \mathbf{f}_y(s_*, s_{\mathcal{I}}, s_{\mathcal{J}}) - \mathbf{f}_{1-y}(s_*, s_{\mathcal{I}}, s_{\mathcal{J}}) \rangle | y] = \mathbb{P}_{\mathcal{D}}[\Delta_{\mathbf{w}}(y, s_*, s_{\mathcal{I}}, s_{\mathcal{J}}) | y].$$

Note that  $\mathbb{P}_{\mathcal{D}}[s_* | y] = \alpha_{*,\mathcal{D}}$  if  $s_* = y$ . Therefore,  $\mathbb{P}_{\mathcal{D}}[s_* = 1 | y = 1] = \alpha_{*,\mathcal{D}}$  and  $\mathbb{P}_{\mathcal{D}}[s_* = 0 | y = 1] = 1 - \alpha_{*,\mathcal{D}}$ . Similarly,  $\mathbb{P}_{\mathcal{D}}[s_* = 0 | y = 0] = \alpha_{*,\mathcal{D}}$  and  $\mathbb{P}_{\mathcal{D}}[s_* = 1 | y = 0] = 1 - \alpha_{*,\mathcal{D}}$ . Thus

$$\mathbb{P}_{\mathcal{D}}[(2\tilde{y} - 1)(w_*(2s_* - 1) + b_*) | y] \stackrel{(*)}{=} \mathbb{P}_{\mathcal{D}}[w_*(2s_{**} - 1) + b_{**} + (2\tilde{y} - 1)r_y | y]$$

where  $s_{**}$  satisfies  $\mathbb{P}_{\mathcal{D}}[s_{**} = 1] = \alpha_{*,\mathcal{D}}$  and  $\mathbb{P}_{\mathcal{D}}[s_{**} = 0] = 1 - \alpha_{*,\mathcal{D}}$ . Note that (\*) stems from the symmetry of  $s_*$  and  $b_{**}$  with respect to  $y$ . To reduce exposition, we will stick to  $s_*$  notation and continue to refer to  $s_{**}$  as  $s_*$ . Hence, we define  $d_{*,\mathcal{D}}$  as

$$d_{*,\mathcal{D}} := w_*(2s_* - 1) + b_{**} \quad (20)$$

where  $b_{**} := b_* - r_y$  as defined earlier. Therefore, the contribution of the main task model in the majority voting random variable  $\Delta_{\mathbf{w}}(y, s_*, s_{\mathcal{I}}, s_{\mathcal{J}})$  will be

$$d_{*,\mathcal{D}} + (2y - 1)r_y. \quad (21)$$

Next, we analyze the auxiliary model predictions. For  $y = 1$ ,

$$\mathbb{P}_{\mathcal{D}}[(2y - 1)\left(\sum_{i \in \mathcal{I}}(w_i s_i + b_i) - \sum_{j \in \mathcal{J}}(w_j(1 - s_j) + b_j)\right)|y] = \mathbb{P}_{\mathcal{D}}\left[\sum_{i \in \mathcal{I}}(w_i s_i + b_i) - \sum_{j \in \mathcal{J}}(w_j(1 - s_j) + b_j)|y = 1\right]$$

where, on the right hand side, we have  $\mathbb{P}_{\mathcal{D}}[s_i = 1|y = \tilde{y}] = \alpha_{i,\mathcal{D}}$  and  $\mathbb{P}_{\mathcal{D}}[1 - s_j = 1|y = \tilde{y}] = \epsilon_{j,\mathcal{D}}$  for  $\tilde{y} = 1$  over distribution  $\mathcal{D} \in \{\mathcal{D}_b, \mathcal{D}_a\}$ . Therefore, we define  $d_{\mathcal{I},\mathcal{D}}$  as

$$(\Delta_{\mathbf{w}}(y, s_*, s_{\mathcal{I}}, s_{\mathcal{J}}) - d_{*,\mathcal{D}} - r_y|y = 1) = \sum_{i \in \mathcal{I}}(w_i s_i + b_i) - \sum_{j \in \mathcal{J}}(w_j(1 - s_j) + b_j) := d_{\mathcal{I},\mathcal{D}}. \quad (22)$$

Using the same strategy for  $y = 0$ , we define  $d_{\mathcal{J},\mathcal{D}}$  as

$$(\Delta_{\mathbf{w}}(y, s_*, s_{\mathcal{I}}, s_{\mathcal{J}}) - d_{*,\mathcal{D}} + r_y|y = 0) = \sum_{j \in \mathcal{J}}(w_j(1 - s_j) + b_j) - \sum_{i \in \mathcal{I}}(w_i s_i + b_i) := d_{\mathcal{J},\mathcal{D}} \quad (23)$$

where, on the right hand side, we have  $\mathbb{P}_{\mathcal{D}}[1 - s_j = 1|y = \tilde{y}] = \alpha_{j,\mathcal{D}}$  and  $\mathbb{P}_{\mathcal{D}}[s_i = 1|y = \tilde{y}] = \epsilon_{i,\mathcal{D}}$  for  $\tilde{y} = 0$  over  $\mathcal{D} \in \{\mathcal{D}_b, \mathcal{D}_a\}$ .

Combining (21), (22) and (23), we have

$$(\Delta_{\mathbf{w}}(y, s_*, s_{\mathcal{I}}, s_{\mathcal{J}})|y) = d_{*,\mathcal{D}} + y d_{\mathcal{I},\mathcal{D}} + (1 - y) d_{\mathcal{J},\mathcal{D}} + (2y - 1) r_y. \quad (24)$$

**Final step:**  $\mathbb{E}_{s_*, s_{\mathcal{I}}, s_{\mathcal{J}}}[\Delta_{\mathbf{w}}(y, s_*, s_{\mathcal{I}}, s_{\mathcal{J}})|y]$  We express  $\Delta_{\mathbf{w}}(y, s_*, s_{\mathcal{I}}, s_{\mathcal{J}})|y$  in terms of  $y$  and a function of model predictions thus far. In this step, using the bounds on the optimal parameters in the first step as well as the decomposition introduced in the second step, we derive a lower bound for the  $\mathbb{E}_{s_*, s_{\mathcal{I}}, s_{\mathcal{J}}}[\Delta_{\mathbf{w}}(y, s_*, s_{\mathcal{I}}, s_{\mathcal{J}})|y]$ . Towards that, we lower bound the expected value of  $d_{*,\mathcal{D}}$ ,  $d_{\mathcal{I},\mathcal{D}}$  and  $d_{\mathcal{J},\mathcal{D}}$  individually.

- $\mathbb{E}_{s_*}[d_{*,\mathcal{D}}]$ : For the main task model, we have

$$\mathbb{E}_{s_*}[d_{*,\mathcal{D}}] = \mathbb{E}_{s_*}[w_*(2s_* - 1) + b_{**}] \quad (25)$$

over distribution  $\mathcal{D} \in \{\mathcal{D}_b, \mathcal{D}_a\}$  and  $w_*$ . One can infer from (14) and (15) for  $b_{**} = b_* - r_y$  that

$$\mathbb{E}_{s_*}[d_{*,\mathcal{D}}] = \mathbb{E}_{s_*}[w_*(2s_* - 1) + (2y - 1)b_{**}] \geq \alpha_{*,\mathcal{D}} \log \frac{\wedge \alpha_*}{1 - \wedge \alpha_*} + (1 - \alpha_{*,\mathcal{D}}) \log \frac{1 - \vee \alpha_*}{\vee \alpha_*} := \mu_{d_{*,\mathcal{D}}}. \quad (26)$$

- $\mathbb{E}_{s_{\mathcal{I}}, s_{\mathcal{J}}}[d_{\mathcal{I},\mathcal{D}}]$ : For the permissive models, we have

$$\mathbb{E}_{s_{\mathcal{I}}, s_{\mathcal{J}}}[d_{\mathcal{I},\mathcal{D}}] = \mathbb{E}_{s_{\mathcal{I}}, s_{\mathcal{J}}}\left[\sum_{i \in \mathcal{I}}(w_i s_i + b_i) - \sum_{j \in \mathcal{J}}(w_j(1 - s_j) + b_j)\right] = \mathbb{E}_{s_{\mathcal{I}}}\left[\sum_{i \in \mathcal{I}}(w_i s_i + b_i)\right] - \mathbb{E}_{s_{\mathcal{J}}}\left[\sum_{j \in \mathcal{J}}(w_j(1 - s_j) + b_j)\right].$$

Note that  $w_i s_i + b_i = w_i + b_i$  with probability  $\alpha_{i,\mathcal{D}}$  and  $w_i s_i + b_i = b_i$  otherwise. Therefore, using (16) and (17) we lower bound  $\mathbb{E}_{s_{\mathcal{I}}}\left[\sum_{i \in \mathcal{I}}(w_i s_i + b_i)\right]$  as

$$\mathbb{E}_{s_{\mathcal{I}}}\left[\sum_{i \in \mathcal{I}}(w_i s_i + b_i)\right] \geq \sum_{i \in \mathcal{I}} \alpha_{i,\mathcal{D}} \log \frac{\wedge \alpha_i}{\vee \epsilon_i} + (1 - \alpha_{i,\mathcal{D}}) \log \frac{1 - \vee \alpha_i}{1 - \wedge \epsilon_i}.$$

Similarly,  $-\mathbb{E}_{s_{\mathcal{J}}}\left[\sum_{j \in \mathcal{J}}(w_j(1 - s_j) + b_j)\right]$  can be lower bounded as

$$-\mathbb{E}_{s_{\mathcal{J}}}\left[\sum_{j \in \mathcal{J}}(w_j(1 - s_j) + b_j)\right] \geq -\sum_{j \in \mathcal{J}} \epsilon_{j,\mathcal{D}} \log \frac{\vee \alpha_j}{\wedge \epsilon_j} + (1 - \epsilon_{j,\mathcal{D}}) \log \frac{1 - \wedge \alpha_j}{1 - \vee \epsilon_j}.$$

Combining above result, we have

$$\mathbb{E}_{s_{\mathcal{I}}, s_{\mathcal{J}}}[d_{\mathcal{I},\mathcal{D}}] \geq \sum_{i \in \mathcal{I}} \alpha_{i,\mathcal{D}} \log \frac{\wedge \alpha_i}{\vee \epsilon_i} + (1 - \alpha_{i,\mathcal{D}}) \log \frac{1 - \vee \alpha_i}{1 - \wedge \epsilon_i} - \sum_{j \in \mathcal{J}} \epsilon_{j,\mathcal{D}} \log \frac{\vee \alpha_j}{\wedge \epsilon_j} - (1 - \epsilon_{j,\mathcal{D}}) \log \frac{1 - \wedge \alpha_j}{1 - \vee \epsilon_j} := \mu_{\mathcal{I},\mathcal{D}}. \quad (27)$$

- $\mathbb{E}_{s_{\mathcal{I}}, s_{\mathcal{J}}}[d_{\mathcal{J}, \mathcal{D}}]$ : Following to the same strategy to that of  $\mathbb{E}_{s_{\mathcal{I}}, s_{\mathcal{J}}}[d_{\mathcal{I}, \mathcal{D}}]$ , we have

$$\mathbb{E}_{s_{\mathcal{I}}, s_{\mathcal{J}}}[d_{\mathcal{J}, \mathcal{D}}] \geq \sum_{j \in \mathcal{J}} \alpha_{j, \mathcal{D}} \log \frac{\wedge \alpha_j}{\vee \epsilon_j} + (1 - \alpha_{j, \mathcal{D}}) \log \frac{1 - \vee \alpha_j}{1 - \wedge \epsilon_j} - \sum_{i \in \mathcal{I}} \epsilon_{i, \mathcal{D}} \log \frac{\vee \alpha_i}{\wedge \epsilon_i} - (1 - \epsilon_{i, \mathcal{D}}) \log \frac{1 - \wedge \alpha_i}{1 - \vee \epsilon_i} := \mu_{\mathcal{J}, \mathcal{D}}. \quad (28)$$

Finally, combining (24, 25, 27, 28) we conclude

$$\begin{aligned} \mathbb{E}_{s_*, s_{\mathcal{I}}, s_{\mathcal{J}}}[\Delta_{\mathbf{w}}(y, s_*, s_{\mathcal{I}}, s_{\mathcal{J}})|y] &= \mathbb{E}_{s_*, s_{\mathcal{I}}, s_{\mathcal{J}}}[d_{*, \mathcal{D}} + yd_{\mathcal{I}, \mathcal{D}} + (1 - y)d_{\mathcal{J}, \mathcal{D}} + (2y - 1)r_y] \\ &\geq \mu_{*, \mathcal{D}} + y\mu_{\mathcal{I}, \mathcal{D}} + (1 - y)\mu_{\mathcal{J}, \mathcal{D}} + (2y - 1)r_y := \mu_{y, \mathcal{D}}. \end{aligned} \quad (29)$$

The proof is thus completed.  $\square$

#### A.4. Proof of Theorem 1

We start by recalling our main theorem.

**Theorem (Recall).** For  $y \in \mathcal{Y}$  and  $\mathcal{D} \in \{\mathcal{D}_b, \mathcal{D}_a\}$ , let  $\mu_{y, \mathcal{D}}$  be defined as in Lemma 1. Suppose that the modeling assumption holds, and suppose that  $\mu_{d_{\mathcal{K}}, \mathcal{D}} > 0$ , for all  $\mathcal{K} \in \{\mathcal{I}, \mathcal{J}\}$  and  $\mathcal{D} \in \{\mathcal{D}_b, \mathcal{D}_a\}$ . Then

$$\mathcal{A}^{\text{KEMLP}} \geq 1 - \mathbb{E}_{\mu_{y, \mathcal{D}}}[\exp(-2\mu_{y, \mathcal{D}}^2/v^2)], \quad (30)$$

where  $v^2$  is the variance upper bound to  $\mathbb{P}[o = y|y]$  with

$$v^2 = 4 \left( \log \frac{\vee \alpha_*}{1 - \wedge \alpha_*} \right)^2 + \sum_{k \in \mathcal{I} \cup \mathcal{J}} \left( \log \frac{\vee \alpha_k (1 - \wedge \epsilon_k)}{\wedge \epsilon_k (1 - \vee \alpha_k)} \right)^2.$$

*Proof of Theorem 1.* Recall that we define weighted robust accuracy of KEMLP as

$$\mathcal{A}^{\text{KEMLP}} = \mathbb{E}_{\mathcal{D} \sim \{\mathcal{D}_a, \mathcal{D}_b\}} \mathbb{E}_{y \sim \mathcal{Y}} [\mathbb{P}_{\mathcal{D}}[o = y|y, \mathbf{w}]].$$

The weighted accuracy definition comes from the latent variable  $z$ . That is,  $\mathcal{A}^{\text{KEMLP}} = \mathbb{P}[o = y|\mathbf{w}] = \sum_{z \in \{0, 1\}} \mathbb{P}[o = y|z, \mathbf{w}]$  where  $\mathbb{P}[o = y|z = 0, \mathbf{w}] = \mathbb{P}_{\mathcal{D}_b}[o = y|\mathbf{w}]$  and  $\mathbb{P}[o = y|z = 1, \mathbf{w}] = \mathbb{P}_{\mathcal{D}_a}[o = y|\mathbf{w}]$ . Hence,  $\mathcal{A}^{\text{KEMLP}} = \mathbb{E}_{\mathcal{D} \sim \{\mathcal{D}_b, \mathcal{D}_a\}} [\mathbb{P}_{\mathcal{D}}[o = y|\mathbf{w}]] = \mathbb{E}_{\mathcal{D} \sim \{\mathcal{D}_b, \mathcal{D}_a\}} \mathbb{E}_{y \sim \mathcal{Y}} [\mathbb{P}_{\mathcal{D}}[o = y|y, \mathbf{w}]]$ .

Let  $\mathbf{w}$  be the set of optimal parameters. Using (7) and our inference rule,  $\mathbb{P}_{\mathcal{D}}[o = y|y, \mathbf{w}]$  can be further expressed as

$$\begin{aligned} \mathbb{P}_{\mathcal{D}}[o = y|y, \mathbf{w}] \\ = \mathbb{P}_{\mathcal{D}}[\sigma(\Delta_{\mathbf{w}}(y, s_*, s_{\mathcal{I}}, s_{\mathcal{J}})) > 1/2|y] = \mathbb{P}_{\mathcal{D}}[\Delta_{\mathbf{w}}(y, s_*, s_{\mathcal{I}}, s_{\mathcal{J}}) > 0|y] = 1 - \mathbb{P}_{\mathcal{D}}[\Delta_{\mathbf{w}}(y, s_*, s_{\mathcal{I}}, s_{\mathcal{J}}) < 0|y] \end{aligned}$$

For the rest of the proof, we will focus on bounding the term  $\mathbb{P}_{\mathcal{D}}[\Delta_{\mathbf{w}}(y, s_*, s_{\mathcal{I}}, s_{\mathcal{J}}) < 0|y]$ , and  $\mathcal{A}^{\text{KEMLP}}$  will follow from taking expectation of  $1 - \mathbb{P}_{\mathcal{D}}[\Delta_{\mathbf{w}}(y, s_*, s_{\mathcal{I}}, s_{\mathcal{J}}) < 0|y]$  over  $\mathcal{D} \in \{\mathcal{D}_b, \mathcal{D}_a\}$  and  $y \in \mathcal{Y}$ .

Next, we recall the generalized bounded difference inequality as well as generalized Hoeffding's inequality (van de Geer, 2002). Note that the same result can be shown via Azuma's inequality for submartingale sequences (Azuma, 1967).

**Theorem 3** ((Azuma, 1967), (van de Geer, 2002)). Assume that  $X_t$  be a random variable with respect to filtration  $\mathcal{F}_t$ , and  $\mathcal{L}_t$  and  $\mathcal{U}_t$  be  $\mathcal{F}_{t-1}$  measurable random variables such that

$$\mathcal{L}_t \leq X_t - X_{t-1} \leq \mathcal{U}_t$$

where  $\mathcal{L}_t < \mathcal{U}_t$  and  $\mathcal{U}_t - \mathcal{L}_t \leq c_t$  almost surely. Therefore, for some  $\epsilon > 0$ , one has

$$\mathbb{P}(X_n - \mathbb{E}[X_n] < -\epsilon) \leq \exp\left(-\frac{2\epsilon^2}{\sum_{t=[n]} c_t^2}\right) \quad \text{and symmetrically} \quad \mathbb{P}(X_n - \mathbb{E}[X_n] > \epsilon) \leq \exp\left(-\frac{2\epsilon^2}{\sum_{t=[n]} c_t^2}\right). \quad (31)$$

We now consider the random variable  $\Delta_{\mathbf{w}}(y, s_*, s_{\mathcal{I}}, s_{\mathcal{J}}) = d_{*, \mathcal{D}} + yd_{\mathcal{I}, \mathcal{D}} + (1 - y)d_{\mathcal{J}, \mathcal{D}} + (2y - 1)r_y$  that is meant to represent  $X_n$  in Theorem 3, where each increment is induced by a single model. We call  $\Delta_{\mathbf{w}}(y, s_*, s_{\mathcal{I}}, s_{\mathcal{J}})$  as  $X_{1+|\mathcal{I}|+|\mathcal{J}|}$ .

To prove compatibility of our setting with the Theorem 3, we present the following remark.

**Remark 3** (Measurability of  $X_{1+|\mathcal{I}|+|\mathcal{J}|}$  and the bounded differences). *Let  $y = 1$ . We can write our random variable  $X_{1+|\mathcal{I}|+|\mathcal{J}|} = \Delta_{\mathbf{w}}(y, s_*, s_{\mathcal{I}}, s_{\mathcal{J}})$  as*

$$(\Delta_{\mathbf{w}}(y, s_*, s_{\mathcal{I}}, s_{\mathcal{J}})|y = 1) = w_*(2s_* - 1) + b_* + \sum_{i \in \mathcal{I}} (w_i s_i + b_i) - \sum_{j \in \mathcal{J}} (w_j(1 - s_j) + b_j).$$

*That is, we represent  $(\Delta_{\mathbf{w}}(y, s_*, s_{\mathcal{I}}, s_{\mathcal{J}})|y = 1)$  as a random process with a total of  $1 + |\mathcal{I}| + |\mathcal{J}|$  increments. Let  $X_0 = 0$ , we treat the main sensor as the first increment such that*

$$X_1 = w_*(2s_* - 1) + b_*.$$

*For  $t = 1, \dots, |\mathcal{I}|$  we let*

$$X_{t+1} - X_t = w_i s_i + b_i \text{ s.t. } i = t + 1.$$

*Finally, for  $t = |\mathcal{I}| + 1, \dots, |\mathcal{I}| + |\mathcal{J}|$  we let*

$$X_{t+1} - X_t = -(w_j(1 - s_j) + b_j) \text{ s.t. } j = t + 1.$$

*and the similar analysis can be performed for  $y = 0$ .*

*Above decomposition shows that  $X_{1+|\mathcal{I}|+|\mathcal{J}|}$  is  $\mathcal{F}_n$  measurable. Specifically,  $X_{t+1} - X_t$  is  $\mathcal{F}_t$  measurable for all  $t = 1, \dots, 1 + |\mathcal{I}| + |\mathcal{J}|$ . Moreover,  $X_{t+1} - X_t$  and  $X_{t'+1} - X_{t'}$  are independent for  $t \neq t'$ .*

*Using the increments introduced above, one can further show that the maximum increments  $c_t$  for  $t = 1, \dots, 1 + |\mathcal{I}| + |\mathcal{J}|$  are given by*

$$|w_* + b_* - (-w_* + b_*)| = 2w_* \leq 2\sqrt{w_*} := c_1.$$

*For  $t = 1, \dots, |\mathcal{I}|$  we let*

$$|X_{t+1} - X_t| = |(w_i + b_i) - b_i| \leq \sqrt{w_i} := c_{t+1} \text{ s.t. } i = t + 1.$$

*Finally, for  $t = |\mathcal{I}| + 1, \dots, |\mathcal{I}| + |\mathcal{J}|$  we let*

$$|X_{t+1} - X_t| = |-(w_j + b_j) - (-b_j)| \leq \sqrt{w_j} := c_{t+1} \text{ s.t. } i = t + 1.$$

*Recalling the bounds in (14, 16, 17, 18, 19), we have*

$$c_1 = 2 \log \frac{\sqrt{\alpha_*}}{1 - \wedge \alpha_*} \text{ for } t=1 \text{ and } c_t = \log \frac{\sqrt{\alpha_t}(1 - \wedge \epsilon_t)}{\wedge \epsilon_t(1 - \sqrt{\alpha_t})} \text{ for } t \in \mathcal{I} \cup \mathcal{J}. \quad (32)$$

Next, for any  $y \in \mathcal{Y}$ , we derive the following

$$\begin{aligned} & \mathbb{P}_{\mathcal{D}}[\Delta_{\mathbf{w}}(y, s_*, s_{\mathcal{I}}, s_{\mathcal{J}}) < 0|y] \\ &= \mathbb{P}_{\mathcal{D}}[\Delta_{\mathbf{w}}(y, s_*, s_{\mathcal{I}}, s_{\mathcal{J}}) - \mathbb{E}_{s_*, s_{\mathcal{I}}, s_{\mathcal{J}}}[\Delta_{\mathbf{w}}(y, s_*, s_{\mathcal{I}}, s_{\mathcal{J}})] < -\mathbb{E}_{s_*, s_{\mathcal{I}}, s_{\mathcal{J}}}[\Delta_{\mathbf{w}}(y, s_*, s_{\mathcal{I}}, s_{\mathcal{J}})]|y] \\ &\stackrel{(*)}{\leq} \mathbb{P}_{\mathcal{D}}[\Delta_{\mathbf{w}}(y, s_*, s_{\mathcal{I}}, s_{\mathcal{J}}) - \mathbb{E}_{s_*, s_{\mathcal{I}}, s_{\mathcal{J}}}[\Delta_{\mathbf{w}}(y, s_*, s_{\mathcal{I}}, s_{\mathcal{J}})]|y] < -\mu_{y, \mathcal{D}}|y] \end{aligned}$$

where (\*) stems from that  $\mu_{y, \mathcal{D}}$  is a lower bound to  $\mathbb{E}_{s_*, s_{\mathcal{I}}, s_{\mathcal{J}}}[\Delta_{\mathbf{w}}(y, s_*, s_{\mathcal{I}}, s_{\mathcal{J}})|y]$  as shown in Lemma 1.

Let  $\epsilon = \mu_{y, \mathcal{D}}$ . If  $\mu_{y, \mathcal{D}} > 0$ , using Theorem 3 for  $\Psi_2 = \frac{\sum_{t \in \{1\} \cup \mathcal{I} \cup \mathcal{J}} c_t^2}{\mu_{y, \mathcal{D}}^2}$  where  $c_t$  is as defined in (32) results in

$$\mathbb{P}_{\mathcal{D}}[\Delta_{\mathbf{w}}(y, s_*, s_{\mathcal{I}}, s_{\mathcal{J}}) < 0|y] \leq \mathbb{P}_{\mathcal{D}}[\Delta_{\mathbf{w}}(y, s_*, s_{\mathcal{I}}, s_{\mathcal{J}}) - \mathbb{E}_{s_*, s_{\mathcal{I}}, s_{\mathcal{J}}}[\Delta_{\mathbf{w}}(y, s_*, s_{\mathcal{I}}, s_{\mathcal{J}})]|y] < -\mu_{y, \mathcal{D}}|y] \leq \exp(-2/\Psi_2).$$

By further taking the expectation of  $\mathbb{P}_{\mathcal{D}}[\Delta_{\mathbf{w}}(y, s_*, s_{\mathcal{I}}, s_{\mathcal{J}}) < 0|y]$  over  $\mathcal{D} \in \{\mathcal{D}_b, \mathcal{D}_a\}$  and  $y \in \mathcal{Y}$  such that

$$\begin{aligned} \mathcal{A}^{\text{KEMPLP}} &= \mathbb{E}_{\mathcal{D} \sim \{\mathcal{D}_a, \mathcal{D}_b\}} \mathbb{E}_{y \sim \mathcal{Y}} [\mathbb{P}_{\mathcal{D}}[o = y|y]] = \mathbb{E}_{\mathcal{D} \sim \{\mathcal{D}_a, \mathcal{D}_b\}} \mathbb{E}_{y \sim \mathcal{Y}} [\mathbb{P}_{\mathcal{D}}[\Delta_{\mathbf{w}}(y, s_*, s_{\mathcal{I}}, s_{\mathcal{J}}) > 0|y]] \\ &= 1 - \mathbb{E}_{\mathcal{D} \sim \{\mathcal{D}_a, \mathcal{D}_b\}} \mathbb{E}_{y \sim \mathcal{Y}} [\mathbb{P}_{\mathcal{D}}[\Delta_{\mathbf{w}}(y, s_*, s_{\mathcal{I}}, s_{\mathcal{J}}) < 0|y]] \geq 1 - \mathbb{E}_{\mu_{y, \mathcal{D}}} [\exp(-2\mu_{y, \mathcal{D}}^2/v^2)] \end{aligned}$$

concludes the proof.  $\square$

### A.5. Proof of Theorem 2

We begin with recalling Theorem 2.

**Theorem (Recall).** *Let the number of permissive and preventative models be the same and denoted by  $n$  such that  $n := |\mathcal{I}| = |\mathcal{J}|$ . Note that the weighted accuracy of the main model in terms of its truth rate is simply  $\alpha_* := \sum_{\mathcal{D} \in \{\mathcal{D}_b, \mathcal{D}_a\}} \pi_{\mathcal{D}} \alpha_{*, \mathcal{D}}$ . Moreover, let  $\mathcal{K}, \mathcal{K}' \in \{\mathcal{I}, \mathcal{J}\}$  with  $\mathcal{K} \neq \mathcal{K}'$  and for any  $\mathcal{D} \in \{\mathcal{D}_b, \mathcal{D}_a\}$ , let*

$$\gamma_{\mathcal{D}} := \frac{1}{n+1} \min_{\mathcal{K}} \left\{ \alpha_{*, \mathcal{D}} - 1/2 + \sum_{k \in \mathcal{K}} \alpha_{k, \mathcal{D}} - \sum_{k' \in \mathcal{K}'} \epsilon_{k', \mathcal{D}} \right\}.$$

If  $\gamma_{\mathcal{D}} > \sqrt{\frac{4}{n+1} \log \frac{1}{1-\alpha_*}}$  for all  $\mathcal{D} \in \{\mathcal{D}_b, \mathcal{D}_a\}$ , then  $\mathcal{A}^{KEMLP} > \mathcal{A}^{main}$ .

*Proof of Theorem 2.* We start by recalling the widely known Chernoff bound for the sum of independent and non-identical random variables.

**Lemma 2** (Chernoff Bound for Poisson Binomial Distributions). *Let  $X$  be a random variable with Poisson Binomial distribution. For  $\delta \in [0, 1]$ ,*

$$\mathbb{P}[X < (1 - \delta)\mu_X] \leq \exp(-\delta^2 \mu_X / 2).$$

Recall that KEMLP predicts  $y$  to be  $\hat{o}$  where

$$\hat{o} = \arg \max_{\tilde{y} \in \mathcal{Y}} \mathbb{P}[o = \tilde{y} | \tilde{s}_*, \tilde{s}_{\mathcal{I}}, \tilde{s}_{\mathcal{J}}, \mathbf{w}] = \arg \max_{\tilde{y} \in \mathcal{Y}} \sigma(\Delta_{\mathbf{w}}(\tilde{y}, s_*, s_{\mathcal{I}}, s_{\mathcal{J}}))$$

where

$$\Delta_{\mathbf{w}}(\tilde{y}, s_*, s_{\mathcal{I}}, s_{\mathcal{J}}) = (2\tilde{y} - 1) \left( b + w_*(2s_* - 1) + \sum_{i \in \mathcal{I}} w_i s_i - \sum_{j \in \mathcal{J}} w_j (1 - s_j) \right).$$

We showed earlier that there exist a set of parameters  $\mathbf{w}$ , and call it optimal parameters  $\mathbf{w}^*$ , where

$$\mathbb{P}[o = \tilde{y} | \tilde{s}_*, \tilde{s}_{\mathcal{I}}, \tilde{s}_{\mathcal{J}}, \mathbf{w}^*] = \mathbb{P}[y = \tilde{y} | \tilde{s}_*, \tilde{s}_{\mathcal{I}}, \tilde{s}_{\mathcal{J}}]$$

for all  $\tilde{y} \in \mathcal{Y}$ .

Note that, due to above equation,  $\mathbb{P}[o = \tilde{y} | \tilde{s}_*, \tilde{s}_{\mathcal{I}}, \tilde{s}_{\mathcal{J}}, \mathbf{w}^*]$  is Bayes classifier where the error of classifier is minimized over  $\mathbf{w}$ . Hence,

$$\mathbb{P}[\hat{o} \neq y | \mathbf{w}^*] \leq \mathbb{P}[\hat{o} \neq y | \mathbf{w}]$$

and

$$\mathbb{P}[\hat{o} = y | \mathbf{w}^*] \geq \mathbb{P}[\hat{o} = y | \mathbf{w}]$$

for any  $\mathbf{w} \in \mathbb{R}^{|\mathcal{I}|+|\mathcal{J}|+2}$ .

Leveraging above fact, we will bound  $\mathbb{P}[\hat{o} = y | \mathbf{w}]$  from below where we will use some parameters  $\mathbf{w}$  that are not optimal. That is, from now on, we will focus on  $\mathbb{P}[\hat{o} = y | \mathbf{w}]$  where  $\mathbf{w}$  is not optimal but leads to a close resemblance of  $\mathbb{P}[\hat{o} = y | \mathbf{w}^*]$ . In other words, we will perform a worst-case analysis where  $\hat{o}$  will be a result of unweighted majority voting. Hence, we let  $\mathbf{w}$  be given by  $\mathbf{w} = [0; 1/2; (1)_{i \in \mathcal{I}}; (1)_{j \in \mathcal{J}}]$ . For this case,  $\Delta_{\mathbf{w}}(\tilde{y}, s_*, s_{\mathcal{I}}, s_{\mathcal{J}})$  becomes a random variable with Poisson Binomial distribution and with some bias. That is,

$$\Delta_{\mathbf{w}}(\tilde{y}, s_*, s_{\mathcal{I}}, s_{\mathcal{J}}) = (2\tilde{y} - 1) \left( (s_* - 1/2) + \sum_{i \in \mathcal{I}} s_i - \sum_{j \in \mathcal{J}} (1 - s_j) \right)$$

where  $s_*$ ,  $s_{i \in \mathcal{I}}$  and  $s_{j \in \mathcal{J}}$  are random variables in  $\mathcal{Y}$ .

Using the weight introduced above, we can now re-write the weighted robust accuracy of KEMLP as

$$\begin{aligned} \mathcal{A}^{\text{KEMLP}} &= \mathbb{P}[\hat{o} = y | \mathbf{w}^*] \geq \mathbb{P}[\hat{o} = y | \mathbf{w}] = \pi_{\mathcal{D}_a} \mathbb{P}_{\mathcal{D}_a}[\hat{o} = y | \mathbf{w}] + \pi_{\mathcal{D}_b} \mathbb{P}_{\mathcal{D}_b}[\hat{o} = y | \mathbf{w}] \\ &= \pi_{\mathcal{D}_a} (\mathbb{P}_{\mathcal{D}_a}[\hat{o} = y | \mathbf{w}, y = 1] \mathbb{P}_{\mathcal{D}_a}[y = 1] + \mathbb{P}_{\mathcal{D}_a}[\hat{o} = y | \mathbf{w}, y = 0] \mathbb{P}_{\mathcal{D}_a}[y = 0]) \\ &\quad + \pi_{\mathcal{D}_b} (\mathbb{P}_{\mathcal{D}_b}[\hat{o} = y | \mathbf{w}, y = 1] \mathbb{P}_{\mathcal{D}_b}[y = 1] + \mathbb{P}_{\mathcal{D}_b}[\hat{o} = y | \mathbf{w}, y = 0] \mathbb{P}_{\mathcal{D}_b}[y = 0]). \end{aligned} \quad (33)$$

Next, we will derive a lower bound for  $\mathbb{P}_{\mathcal{D}}[\hat{o} = y | y = \tilde{y}, \mathbf{w}]$  for  $\mathcal{D} \in \{\mathcal{D}_b, \mathcal{D}_a\}$  and for all  $\tilde{y} \in \{0, 1\}$ .

**For  $y = 1$ :** We have

$$\begin{aligned} \mathbb{P}_{\mathcal{D}}[\hat{o} = y | \mathbf{w}, y = 1] &= \mathbb{P}_{\mathcal{D}}[s_* + \sum_{i \in \mathcal{I}} s_i + \sum_{j \in \mathcal{J}} s_j - (|\mathcal{J}| + 1/2) \geq 0 | y = 1] \\ 1 - \mathbb{P}_{\mathcal{D}}[s_* + \sum_{i \in \mathcal{I}} s_i + \sum_{j \in \mathcal{J}} s_j - (|\mathcal{J}| + 1/2) < 0 | y = 1] &= 1 - \mathbb{P}_{\mathcal{D}}[s_* + \sum_{i \in \mathcal{I}} s_i + \sum_{j \in \mathcal{J}} s_j < |\mathcal{J}| + 1/2 | y = 1] \end{aligned}$$

where  $\mathbb{P}_{\mathcal{D}}[s_* = 1 | y = 1] = \alpha_{*,\mathcal{D}}$  (resp.  $\mathbb{P}_{\mathcal{D}}[s_i = 1 | y = 1] = \alpha_{i,\mathcal{D}}$  and  $\mathbb{P}_{\mathcal{D}}[s_j = 1 | y = 1] = 1 - \epsilon_{j,\mathcal{D}}$ ).

We let

$$\Psi_{\mathcal{D},y=1} := s_* + \sum_{i \in \mathcal{I}} s_i + \sum_{j \in \mathcal{J}} s_j - (|\mathcal{J}| + 1/2)$$

and

$$\hat{\Psi}_{\mathcal{D},y=1} := s_* + \sum_{i \in \mathcal{I}} s_i + \sum_{j \in \mathcal{J}} s_j = \Psi_{\mathcal{D},y=1} + |\mathcal{J}| + 1/2.$$

Similarly, the expected values of  $\Psi_{\mathcal{D},y=1}$  and  $\hat{\Psi}_{\mathcal{D},y=1}$  over  $s_*$ ,  $s_i$  and  $s_j$  are given by  $\mu_{\Psi_{\mathcal{D},y=1}}$  and  $\mu_{\hat{\Psi}_{\mathcal{D},y=1}}$ , respectively. Precisely,

$$\mu_{\Psi_{\mathcal{D},y=1}} = \alpha_{*,\mathcal{D}} - 1/2 + \sum_{i \in \mathcal{I}} \alpha_{i,\mathcal{D}} - \sum_{j \in \mathcal{J}} \epsilon_{j,\mathcal{D}}$$

and

$$\mu_{\hat{\Psi}_{\mathcal{D},y=1}} = \alpha_{*,\mathcal{D}} + \sum_{i \in \mathcal{I}} \alpha_{i,\mathcal{D}} + \sum_{j \in \mathcal{J}} (1 - \epsilon_{j,\mathcal{D}}) = \mu_{\Psi_{\mathcal{D},y=1}} + |\mathcal{J}| + 1/2$$

We then write  $\mathbb{P}_{\mathcal{D}}[\hat{o} \neq y | \mathbf{w}, y = 1]$  as

$$\mathbb{P}_{\mathcal{D}}[\hat{o} \neq y | \mathbf{w}, y = 1] = \mathbb{P}[\Psi_{\mathcal{D},y=1} < 0] \leq \exp(-\delta_{\mathcal{D},y=1}^2 \mu_{\hat{\Psi}_{\mathcal{D},y=1}} / 2)$$

where

$$\delta_{\mathcal{D},y=1} = 1 - \frac{|\mathcal{J}| + 1/2}{\mu_{\hat{\Psi}_{\mathcal{D},y=1}}} = \frac{\mu_{\Psi_{\mathcal{D},y=1}}}{\mu_{\hat{\Psi}_{\mathcal{D},y=1}}}.$$

Let now  $\gamma_{\mathcal{D},y=1}$  be the difference between true and false rates of sensors normalized over preventative models when  $y = 1$  such that

$$\gamma_{\mathcal{D},y=1} := \frac{1}{|\mathcal{J}| + 1} (\alpha_{*,\mathcal{D}} - 1/2 + \sum_{i \in \mathcal{I}} \alpha_{i,\mathcal{D}} - \sum_{j \in \mathcal{J}} \epsilon_{j,\mathcal{D}}).$$

Noting that  $\mu_{\Psi_{\mathcal{D},y=1}} = (|\mathcal{I}|+1)\gamma_{\mathcal{D},y=1}$ , we have  $\delta_{\mathcal{D},y=1} = \frac{(|\mathcal{I}|+1)\gamma_{\mathcal{D},y=1}}{(|\mathcal{I}|+1)\gamma_{\mathcal{D},y=1} + |\mathcal{I}| + 1/2}$  and  $\mu_{\hat{\Psi}_{y=1}} = (|\mathcal{I}|+1)\gamma_{\mathcal{D},y=1} + |\mathcal{I}| + 1/2$ . Using Lemma 2 for a Poisson random variable  $\hat{\Psi}_{y=1}$ , we bound  $\mathbb{P}_{\mathcal{D}}[\hat{o} \neq y | \mathbf{w}, y = 1]$  as

$$\begin{aligned} \mathbb{P}_{\mathcal{D}}[\hat{o} \neq y | \mathbf{w}, Y = 1] &= \mathbb{P}[\Psi_{\mathcal{D},y=1} < 0] = \mathbb{P}[\hat{\Psi}_{\mathcal{D},y=1} < |\mathcal{I}| + 1/2] \leq \exp(-\delta_{\mathcal{D},y=1}^2 \mu_{\hat{\Psi}_{\mathcal{D},y=1}} / 2) \\ &= \exp\left(-\frac{(|\mathcal{I}|+1)^2 \gamma_{\mathcal{D},y=1}^2}{2((|\mathcal{I}|+1)\gamma_{\mathcal{D},y=1} + |\mathcal{I}| + 1/2)}\right) \leq \exp\left(-\frac{(|\mathcal{I}|+1)^2 \gamma_{\mathcal{D},y=1}^2}{2((|\mathcal{I}|+1)\gamma_{\mathcal{D},y=1} + |\mathcal{I}| + 1)}\right) \\ &= \exp\left(-(|\mathcal{I}|+1) \frac{\gamma_{\mathcal{D},y=1}^2}{2(\gamma_{\mathcal{D},y=1} + 1)}\right) \end{aligned} \quad (34)$$

**For  $y = 0$ :** We have

$$\begin{aligned} \mathbb{P}_{\mathcal{D}}[\hat{o} = y | \mathbf{w}, y = 0] &= \mathbb{P}_{\mathcal{D}}[s_* - 1/2 + \sum_{i \in \mathcal{I}} s_i - \sum_{j \in \mathcal{J}} 1 - s_j \leq 0 | y = 0] \\ 1 - \mathbb{P}_{\mathcal{D}}[s_* - 1/2 + \sum_{i \in \mathcal{I}} s_i - \sum_{j \in \mathcal{J}} 1 - s_j > 0 | y = 0] &= 1 - \mathbb{P}_{\mathcal{D}}[-s_* + 1/2 - \sum_{i \in \mathcal{I}} s_i + \sum_{j \in \mathcal{J}} 1 - s_j < 0 | y = 0] \\ &= 1 - \mathbb{P}_{\mathcal{D}}[-s_* + 1 - 1/2 + \sum_{i \in \mathcal{I}} 1 - s_i - |\mathcal{I}| + \sum_{j \in \mathcal{J}} 1 - s_j < 0 | y = 0] \\ &= 1 - \mathbb{P}_{\mathcal{D}}[-s_* + 1 + \sum_{i \in \mathcal{I}} 1 - s_i + \sum_{j \in \mathcal{J}} 1 - s_j < |\mathcal{I}| + 1/2 | y = 0] \end{aligned}$$

where  $\mathbb{P}_{\mathcal{D}}[s_* = 1 | y = 0] = 1 - \alpha_{*,\mathcal{D}}$  (resp.  $\mathbb{P}_{\mathcal{D}}[s_i = 1 | y = 0] = \epsilon_{i,\mathcal{D}}$  and  $\mathbb{P}_{\mathcal{D}}[s_j = 1 | y = 0] = 1 - \alpha_{j,\mathcal{D}}$ ).

We let

$$\Psi_{\mathcal{D},y=0} := 1 - s_* + \sum_{i \in \mathcal{I}} 1 - s_i + \sum_{j \in \mathcal{J}} 1 - s_j - (|\mathcal{I}| + 1/2)$$

and

$$\hat{\Psi}_{\mathcal{D},y=0} := 1 - s_* + \sum_{i \in \mathcal{I}} 1 - s_i + \sum_{j \in \mathcal{J}} 1 - s_j = \Psi_{\mathcal{D},y=0} + |\mathcal{I}| + 1/2.$$

Similarly, the expected values of  $\Psi_{\mathcal{D},y=0}$  and  $\hat{\Psi}_{\mathcal{D},y=0}$  over  $s_*$ ,  $s_i$  and  $s_j$  are given by  $\mu_{\Psi_{\mathcal{D},y=0}}$  and  $\mu_{\hat{\Psi}_{\mathcal{D},y=0}}$ , respectively. Precisely,

$$\mu_{\Psi_{\mathcal{D},y=0}} = \alpha_{*,\mathcal{D}} - 1/2 - \sum_{i \in \mathcal{I}} \epsilon_{i,\mathcal{D}} + \sum_{j \in \mathcal{J}} \alpha_{j,\mathcal{D}}$$

and

$$\mu_{\hat{\Psi}_{\mathcal{D},y=0}} = \alpha_{*,\mathcal{D}} + \sum_{i \in \mathcal{I}} 1 - \epsilon_{i,\mathcal{D}} + \sum_{j \in \mathcal{J}} \alpha_{j,\mathcal{D}} = \mu_{\Psi_{\mathcal{D},y=0}} + |\mathcal{I}| + 1/2$$

We then write  $\mathbb{P}_{\mathcal{D}}[\hat{o} \neq y | \mathbf{w}, y = 0]$  as

$$\mathbb{P}_{\mathcal{D}}[\hat{o} \neq y | \mathbf{w}, y = 0] = \mathbb{P}[\Psi_{\mathcal{D},y=0} < 0] \leq \exp(-\delta_{\mathcal{D},y=0}^2 \mu_{\hat{\Psi}_{\mathcal{D},y=0}} / 2)$$

where

$$\delta_{\mathcal{D},y=0} = 1 - \frac{|\mathcal{I}| + 1/2}{\mu_{\hat{\Psi}_{\mathcal{D},y=0}}} = \frac{\mu_{\Psi_{\mathcal{D},y=0}}}{\mu_{\hat{\Psi}_{\mathcal{D},y=0}}}.$$

Let now  $\gamma_{\mathcal{D},y=0}$  be the difference between true and false rates of sensors normalized over permissive models when  $y = 0$  such that

$$\gamma_{\mathcal{D},y=0} := \frac{1}{|\mathcal{I}| + 1} (\alpha_{*,\mathcal{D}} - 1/2 + \sum_{j \in \mathcal{J}} \alpha_{j,\mathcal{D}} - \sum_{i \in \mathcal{I}} \epsilon_{i,\mathcal{D}}).$$

Noting that  $\mu_{\Psi_{\mathcal{D},y=0}} = (|\mathcal{I}| + 1)\gamma_{\mathcal{D},y=0}$ , we have  $\delta_{\mathcal{D},y=0} = \frac{(|\mathcal{I}|+1)\gamma_{\mathcal{D}}}{(|\mathcal{I}|+1)\gamma_{\mathcal{D}}+|\mathcal{I}|+1/2}$  and  $\mu_{\hat{\Psi}_{y=0}} = (|\mathcal{I}| + 1)\gamma_{\mathcal{D},y=0} + |\mathcal{I}| + 1/2$ . Using Lemma 2 for a Poisson random variable  $\hat{\Psi}_{y=0}$ , we bound  $\mathbb{P}_{\mathcal{D}}[\hat{\sigma} \neq y | \mathbf{w}, y = 0]$  as

$$\begin{aligned} \mathbb{P}_{\mathcal{D}}[\hat{\sigma} \neq y | \mathbf{w}, y = 0] &= \mathbb{P}[\Psi_{\mathcal{D},y=0} < 0] = \mathbb{P}[\hat{\Psi}_{\mathcal{D},y=0} < |\mathcal{I}| + 1/2] \leq \exp(-\delta_{\mathcal{D},y=0}^2 \mu_{\hat{\Psi}_{\mathcal{D},y=0}} / 2) \\ &= \exp\left(-\frac{(|\mathcal{I}| + 1)^2 \gamma_{\mathcal{D},y=0}^2}{2((|\mathcal{I}| + 1)\gamma_{\mathcal{D},y=0} + |\mathcal{I}| + 1/2)}\right) \leq \exp\left(-\frac{(|\mathcal{I}| + 1)^2 \gamma_{\mathcal{D},y=0}^2}{2((|\mathcal{I}| + 1)\gamma_{\mathcal{D},y=0} + |\mathcal{I}| + 1)}\right) \\ &= \exp\left(-(|\mathcal{I}| + 1) \frac{\gamma_{\mathcal{D},y=0}^2}{2(\gamma_{\mathcal{D},y=0} + 1)}\right) \end{aligned} \quad (35)$$

**Last step:** For convenience, let  $n := |\mathcal{I}| = |\mathcal{J}|$  and

$$\gamma_{\mathcal{D}} := \min(\gamma_{\mathcal{D},y=1}, \gamma_{\mathcal{D},y=0}).$$

Using (34) and (35), we bound the pipeline accuracy in (33) such that

$$\begin{aligned} \mathcal{A}^{\text{KEMLP}} &\geq 1 - \sum_{\mathcal{D} \in \{\mathcal{D}_b, \mathcal{D}_a\}} \pi_{\mathcal{D}} \exp\left(- (n+1) \frac{\gamma_{\mathcal{D}}^2}{2(\gamma_{\mathcal{D}} + 1)}\right) \\ &\geq 1 - \sum_{\mathcal{D} \in \{\mathcal{D}_b, \mathcal{D}_a\}} \pi_{\mathcal{D}} \exp\left(- (n+1) \frac{\gamma_{\mathcal{D}}^2}{4}\right). \end{aligned} \quad (36)$$

Hence, if

$$1 - \exp\left(- (n+1) \frac{\gamma_{\mathcal{D}}^2}{4}\right) > \mathcal{A}^{\text{main}} \quad (37)$$

for all  $\mathcal{D} \in \{\mathcal{D}_b, \mathcal{D}_a\}$ , then we have  $\mathcal{A}^{\text{KEMLP}} > \mathcal{A}^{\text{main}}$ . Manipulating (37) for all  $\mathcal{D} \in \{\mathcal{D}_b, \mathcal{D}_a\}$  concludes the proof.  $\square$

## A.6. Proof of Corollary 1

We recall the respective setting as follows. We assume that the auxiliary models are *homogeneous* for each type: permissive or preventative. For example,  $\alpha_k$  is fixed with respect to  $k \in \mathcal{I} \cup \mathcal{J}$ , hence we drop the subscripts, i.e.,  $\alpha_{k,\mathcal{D}} = \alpha$  and  $\epsilon_{k,\mathcal{D}} = \epsilon$ . We assume that the same number of auxiliary models are used, namely  $|\mathcal{I}| = |\mathcal{J}| = n$ , and that the classes are balanced with  $\mathbb{P}_{\mathcal{D}}(y = 1) = \mathbb{P}_{\mathcal{D}}(y = 0)$ , for all  $\mathcal{D} \in \{\mathcal{D}_b, \mathcal{D}_a\}$ . Finally, we let  $\alpha_{*,\mathcal{D}_b} = 1$  and  $\alpha_{*,\mathcal{D}_a} = 0$ , and  $\alpha - \epsilon > 0$ . Then, the following holds.

**Corollary (Recall).** *The weighted robust accuracy of KEMLP in the homogeneous setting satisfies*

$$\mathcal{A}^{\text{KEMLP}} \geq 1 - \exp(-2n(\alpha - \epsilon)^2).$$

*In particular, one has  $\lim_{n \rightarrow \infty} \mathcal{A}^{\text{KEMLP}} = 1$ .*

*Proof of Corollary 1.* First, for  $\alpha_{*,\mathcal{D}_b} = 1$  and  $\alpha_{*,\mathcal{D}_a} = 0$ , using (10) and (11), we note that

$$w_* = b_* = 0.$$

Secondly, in the homogeneous case, the conditional independence reflects to the mixture model and models become conditionally independent in the mixture model as well. That is, the condition on the other models in (16, 17, 18, 19) drops and we have closed form expression for all optimal parameters. Namely, for  $\alpha_{i,\mathcal{D}} = \alpha_{j,\mathcal{D}} = \alpha$  and  $\epsilon_{i,\mathcal{D}} = \epsilon_{j,\mathcal{D}} = \epsilon$  with  $\alpha > \epsilon$ , once can deduce from (16, 17, 18, 19) that the optimal weight of auxiliary sensors are given by  $w_i = w_j = \log \frac{\alpha}{\epsilon}$

and  $b = \sum_{i \in \mathcal{I}} b_i - \sum_{j \in \mathcal{J}} b_j = \sum_{i \in \mathcal{I}} \log \frac{1-\alpha}{1-\epsilon} - \sum_{j \in \mathcal{J}} \log \frac{1-\alpha}{1-\epsilon} = 0$ . Also,  $w_i = w_j > 0$  for  $\alpha > \epsilon$ . For this setting, we can write out  $\mathcal{A}^{\text{KEMLP}}$  as follows.

$$\begin{aligned} \mathcal{A}^{\text{KEMLP}} &= \mathbb{E}_{\mathcal{D} \in \{\mathcal{D}_b, \mathcal{D}_a\}} \mathbb{E}_{y \sim \mathcal{Y}} [\mathbb{P}[d_{*,\mathcal{D}} + yd_{\mathcal{I},\mathcal{D}} + (1-y)d_{\mathcal{J},\mathcal{D}} > 0 | y]] \stackrel{(*)}{=} \mathbb{E}_{y \sim \mathcal{Y}} [\mathbb{P}[yd_{\mathcal{I},\mathcal{D}} + (1-y)d_{\mathcal{J},\mathcal{D}} > 0 | y]] \\ &\stackrel{(**)}{=} \frac{1}{2} (\mathbb{P}[d_{\mathcal{I},\mathcal{D}} > 0 | y = 1] + \mathbb{P}[d_{\mathcal{J},\mathcal{D}} > 0 | y = 0]) \stackrel{(***)}{=} \mathbb{P}[d_{\mathcal{I},\mathcal{D}} > 0 | y = 1] \end{aligned}$$

where  $(*)$  follows from the homogeneity of models over both benign and adversarial distributions as well as that  $d_{*,\mathcal{D}} = w_*(2s_* - 1) = 0$ ,  $(**)$  follows from the class balance, and finally  $(***)$  stems from the symmetry.

Let  $B(n, p)$  denote the Binomial distribution with count parameter  $n$  and success probability  $p$ . Let also that  $d_\alpha$  and  $d_\epsilon$  be random variables with Binomial distributions such that  $d_\alpha \sim B(n, \alpha)$  and  $d_\epsilon \sim B(n, \epsilon)$ . We then rewrite the Weighted Robust Accuracy of KEMLP as follows.

$$\mathcal{A}^{\text{KEMLP}} = \mathbb{P}[d_{\mathcal{I},\mathcal{D}} > 0 | y = 1] = 1 - \mathbb{P}[d_{\mathcal{I},\mathcal{D}} < 0 | y = 1] = 1 - \mathbb{P}[w(d_\alpha - d_\epsilon) < 0 | y = 1] = 1 - \mathbb{P}[d_\alpha - d_\epsilon < 0]$$

where the last equality follows from that  $w = \log \frac{\alpha}{\epsilon} > 0$ .

We then review the Bounded Differences Inequality which will enable us to bound the tail probability  $\mathbb{P}[d_\alpha - d_\epsilon < 0 | y = 1]$ .

**Theorem 4** (Bounded Differences Inequality (Boucheron et al., 2013)). *Assume that a function  $\phi : \mathcal{X}^n \rightarrow \mathbb{R}$  of independent random variables  $X_1, \dots, X_n \in \mathcal{X}$  satisfies the bounded differences property with constants  $c_1, \dots, c_n$ . Denote  $v^2 = \sum_{i=1}^n c_i^2$  and  $Z = \phi(X_1, \dots, X_n)$ .  $Z$  satisfies:*

$$\mathbb{P}(Z - \mathbb{E}(Z) > t) \leq \exp\left(-\frac{2t^2}{v^2}\right) \quad \text{and} \quad \mathbb{P}(Z - \mathbb{E}(Z) < -t) \leq \exp\left(-\frac{2t^2}{v^2}\right).$$

We refer to, for example, (Boucheron et al., 2013) for a proof of Theorem 4.

Using Theorem 4 for  $Z = d_\alpha - d_\epsilon$ ,  $\mathcal{A}^{\text{KEMLP}}$  can be bounded as:

$$\mathcal{A}^{\text{KEMLP}} = 1 - \mathbb{P}[d_\alpha - d_\epsilon < 0] = 1 - \mathbb{P}[d_\alpha - d_\epsilon - \mathbb{E}[d_\alpha - d_\epsilon] < -\mathbb{E}[d_\alpha - d_\epsilon]] = 1 - \mathbb{P}[d_\alpha - d_\epsilon - n(\alpha - \epsilon) < -n(\alpha - \epsilon)].$$

Moreover, for  $t = n(\alpha - \epsilon)$  and  $v^2 = n$  we finally have

$$\mathcal{A}^{\text{KEMLP}} = 1 - \mathbb{P}[d_\alpha - d_\epsilon - n(\alpha - \epsilon) < -n(\alpha - \epsilon)] \geq 1 - \exp\left(-2(n^2(\alpha - \epsilon)^2)/n\right) \geq 1 - \exp\left(-2n(\alpha - \epsilon)^2\right)$$

concludes the proof for the lower bound.

As the final step, we will prove that  $\mathcal{A}^{\text{KEMLP}} > \mathcal{A}^{\text{main}}$ . Note that  $\mathcal{A}^{\text{main}} = \mathbb{E}_{\mathcal{D} \in \{\mathcal{D}_b, \mathcal{D}_a\}} \mathbb{E}_{y \sim \mathcal{Y}} [\mathbb{P}[d_{*,\mathcal{D}} > 0 | y]] = \pi_{\mathcal{D}_b} \alpha_{*,\mathcal{D}_b} + \pi_{\mathcal{D}_a} \alpha_{*,\mathcal{D}_a} = 1/2 \cdot 1 + 1/2 \cdot 0 = 1/2$ . Therefore, it only remains to analyze whether  $\mathcal{A}^{\text{KEMLP}} > 1/2$  or not. Towards that, we state the following result.

**Lemma 3** (On the comparison of two binomial random variables). *Let  $p, q \in [0, 1]$  denote the success probabilities for two Binomial random variables. If  $p > q$ , then  $\mathbb{P}[X > Y] > \frac{1}{2}$ .*

*Proof.* Let  $X$  and  $Y$  be random variables such that  $X \sim B(n, p)$  and  $Y \sim B(n, q)$ .  $Z := X - Y$  can be shown to have the following probability mass function

$$\mathbb{P}(Z = z) = \begin{cases} \sum_{k \in \{0\} \cup [n]} f(k+z, n, p) f(k, n, q) & \text{if } z \geq 0 \\ \sum_{k \in \{0\} \cup [n]} f(k, n, p) f(k+z, n, q) & \text{elsewhere} \end{cases}$$

where  $f(k, n, p) = \binom{n}{k} p^k (1-p)^{n-k}$  for  $k \leq n$ . Moreover, we have

$$\mathbb{P}(Z > 0) = \mathbb{P}(X - Y > 0) = \sum_{\substack{z \in [n] \\ k \in \{0\} \cup [n]}} f(k+z, n, p) f(k, n, q), \quad \mathbb{P}(Z \leq 0) = \sum_{\substack{z \in [n] \\ k \in \{0\} \cup [n]}} f(k, n, p) f(k+z, n, q).$$

Note that if  $p > q$ , then  $f(k+z, n, p) f(k, n, q) > f(k, n, p) f(k+z, n, q)$  for fixed  $n, k \geq 0$ . Hence, the summation over  $z \in [n], k \in \{0\} \cup [n]$  leads to  $\mathbb{P}(Z > 0) > \mathbb{P}(Z \leq 0)$ . It is further implied by  $\mathbb{P}(Z > 0) + \mathbb{P}(Z \leq 0) = 1$  that  $\mathbb{P}(Z > 0) > \frac{1}{2}$ .  $\square$

Using Lemma 3 for  $X = d_\alpha$  and  $Y = d_\epsilon$  as well as that  $\alpha > \epsilon$ , we have

$$\mathcal{A}^{\text{KEMLP}} = \mathbb{P}[d_\alpha - d_\epsilon > 0] = \mathbb{P}[d_\alpha > d_\epsilon] > 1/2 = \mathcal{A}^{\text{main}}.$$

Hence the proof results.  $\square$

## B. Experimental Details

### B.1. Detailed Setup of Baselines

To demonstrate the superior KEMLP, we compare it with two state-of-the-art baselines: **adversarial training** (Madry et al., 2017) and **DOA** (Wu et al., 2019), which are strong defenses against  $\mathcal{L}_p$  bounded attacks and physically realizable attacks respectively.

For adversarial training, we adopt  $\mathcal{L}_\infty$  bound  $\epsilon \in \{4, 8, 16, 32\}$  during training phase. Since adversarial training failed to make progress for  $\epsilon \in \{16, 32\}$ , we use the curriculum training version (Cai et al., 2018), where the model is firstly trained on smaller  $\epsilon$  with  $\epsilon$  gradually increasing to the largest bound. For all versions of adversarial training in our implementation, we adopt 40 iterations of PGD attack with a step size of  $1/255$ . In all cases, pixels are in  $0 \sim 255$  range and the retraining takes 3000 training iterations with a batch size of 200 for each random iteration.

For DOA, we consider adversarial patches with the size of  $5 \times 5$  and  $7 \times 7$  respectively for rectangle occlusion during retraining. For both cases, we use an exhaustive search to pick the attack location and perform 30 iterations PGD inside the adversarial patch to generate noise. The retraining takes 5000 training iterations and the batch size is 200.

Thus, in total, we have 7 baseline CNN models (1 standard CNN model, 4 adversarially trained CNN models, 2 DOA trained CNN models), and we use id numbers  $1 \sim 7$  to denote ‘‘GTSRB-CNN’’, ‘‘AdvTrain ( $\epsilon = 4$ )’’, ‘‘AdvTrain ( $\epsilon = 8$ )’’, ‘‘AdvTrain ( $\epsilon = 16$ )’’, ‘‘AdvTrain ( $\epsilon = 32$ )’’, ‘‘DOA (5x5)’’, ‘‘DOA (7x7)’’, respectively in Figure 2(a).

### B.2. Details of Attacks and Corruptions

Since our constructed KEMLP pipeline is a compound model consisting of multiple sub-models, some of which are not differentiable, we can not directly generate adversarial examples via the standard end-to-end white-box attack. Alternatively, we further propose three different attack settings to evaluate the robustness of our KEMLP pipeline: **1) White-box sensor attack**, where adversarial examples are generated by directly applying gradient methods to the main task model of the KEMLP pipeline in a white-box fashion; **2) Black-box sensor attack**. In this setting, we train substitute model of the main task model using the same model architecture and the same standard training data, and generate adversarial examples with this substitute model; **3) Black-box pipeline attack**, in which we generate adversarial examples with a substitute model, which is obtained via distilling the whole KEMLP pipeline. For this setting, a substitute model with the same GTSRB-CNN architecture is trained on a synthetic training set, where all the images are from the original training set, while the labels are generated by the pipeline model. Then all the models are evaluated on the same set of adversarial test samples crafted on the trained substitute.

Specifically, **1) For  $\mathcal{L}_\infty$  attack**, we consider the strength of  $\epsilon \in \{4, 8, 16, 32\}$  in our evaluation. 1000 iterations of standard PGD (Madry et al., 2017) with a step size of  $1/255$  is used to craft the adversarial examples, and all the three attack settings introduced above are respectively applied; **2) For unforeseen attacks**, we consider the Fog, Snow, JPEG, Gabor and Elastic attacks suggested in Kang et al. (2019), which are all gradient-based worst-case adversarial attacks, generating diverse test distributions distinct from the common  $\mathcal{L}_p$  bounded attacks. For Fog attack, we consider  $\epsilon \in \{256, 512\}$ . For Snow attack, we evaluate for  $\epsilon \in \{0.25, 0.75\}$  respectively. For JPEG attack, we adopt the parameters  $\epsilon \in \{0.125, 0.25\}$ . For Gabor attack,  $\epsilon \in \{20, 40\}$  are tested. Finally,  $\epsilon \in \{1.5, 2.0\}$  are considered for Elastic attack. Since all of these attacks are gradient based, we also apply the three different settings above to generate adversarial examples respectively; **3) For physical attacks on stop signs**, we directly use the same stickers (i.e., the same color and mask) generated in Eykholt et al. (2018) to attack the same 40 stop sign samples, and we also adopt the same end-to-end classification model used in Eykholt et al. (2018) to construct KEMLP model. Since our ultimate goal is defense, we follow the same practice in Wu et al. (2019), where we only consider the digital representation of the attack instead of the real physical implementation, ignoring issues like the attack’s robustness to different viewpoints and environments. Thus, we implement the physical stop sign attack by directly placing the stickers on the stop sign samples in digital space; **4) For common corruptions**, we evaluate our models with the 15 categories of corruptions suggested in Hendrycks and Dietterich (2019). Empirically, in our traffic sign identification task, only 3 types of corruptions out of the 15 categories effectively reduce the accuracy (with a margin over

Table 5. Correspondence between id numbers and attacks/corruptions

| 1                                                                  | 2                                                                | 3                                                                 | 4                                                                 | 5                                                                  |
|--------------------------------------------------------------------|------------------------------------------------------------------|-------------------------------------------------------------------|-------------------------------------------------------------------|--------------------------------------------------------------------|
| Physical Attack                                                    | Fog Corruption                                                   | Contrast Corruption                                               | Brightness Corruption                                             | $\mathcal{L}_\infty$ Attack ( $\epsilon = 4$ , whitebox sensor)    |
| 6                                                                  | 7                                                                | 8                                                                 | 9                                                                 | 10                                                                 |
| $\mathcal{L}_\infty$ Attack ( $\epsilon = 8$ , whitebox sensor)    | $\mathcal{L}_\infty$ Attack ( $\epsilon = 16$ , whitebox sensor) | $\mathcal{L}_\infty$ Attack ( $\epsilon = 32$ , whitebox sensor)  | Fog Attack ( $\epsilon = 256$ , whitebox sensor)                  | Fog Attack ( $\epsilon = 512$ , whitebox sensor)                   |
| 11                                                                 | 12                                                               | 13                                                                | 14                                                                | 15                                                                 |
| Snow Attack ( $\epsilon = 0.25$ , whitebox sensor)                 | Snow Attack ( $\epsilon = 0.75$ , whitebox sensor)               | Jpeg Attack ( $\epsilon = 0.125$ , whitebox sensor)               | Jpeg Attack ( $\epsilon = 0.25$ , whitebox sensor)                | Gabor Attack ( $\epsilon = 20$ , whitebox sensor)                  |
| 16                                                                 | 17                                                               | 18                                                                | 19                                                                | 20                                                                 |
| Gabor Attack ( $\epsilon = 40$ , whitebox sensor)                  | Elastic Attack ( $\epsilon = 1.5$ , whitebox sensor)             | Elastic Attack ( $\epsilon = 2.0$ , whitebox sensor)              | $\mathcal{L}_\infty$ Attack ( $\epsilon = 4$ , blackbox sensor)   | $\mathcal{L}_\infty$ Attack ( $\epsilon = 8$ , blackbox sensor)    |
| 21                                                                 | 22                                                               | 23                                                                | 24                                                                | 25                                                                 |
| $\mathcal{L}_\infty$ Attack ( $\epsilon = 16$ , blackbox sensor)   | $\mathcal{L}_\infty$ Attack ( $\epsilon = 32$ , blackbox sensor) | Fog Attack ( $\epsilon = 256$ , blackbox sensor)                  | Fog Attack ( $\epsilon = 512$ , blackbox sensor)                  | Snow Attack ( $\epsilon = 0.25$ , blackbox sensor)                 |
| 26                                                                 | 27                                                               | 28                                                                | 29                                                                | 30                                                                 |
| Snow Attack ( $\epsilon = 0.75$ , blackbox sensor)                 | Jpeg Attack ( $\epsilon = 0.125$ , blackbox sensor)              | Jpeg Attack ( $\epsilon = 0.25$ , blackbox sensor)                | Gabor Attack ( $\epsilon = 20$ , blackbox sensor)                 | Gabor Attack ( $\epsilon = 40$ , blackbox sensor)                  |
| 31                                                                 | 32                                                               | 33                                                                | 34                                                                | 35                                                                 |
| Elastic Attack ( $\epsilon = 1.5$ , blackbox sensor)               | Elastic Attack ( $\epsilon = 2.0$ , blackbox sensor)             | $\mathcal{L}_\infty$ Attack ( $\epsilon = 4$ , blackbox pipeline) | $\mathcal{L}_\infty$ Attack ( $\epsilon = 8$ , blackbox pipeline) | $\mathcal{L}_\infty$ Attack ( $\epsilon = 16$ , blackbox pipeline) |
| 36                                                                 | 37                                                               | 38                                                                | 39                                                                | 40                                                                 |
| $\mathcal{L}_\infty$ Attack ( $\epsilon = 32$ , blackbox pipeline) | Fog Attack ( $\epsilon = 256$ , blackbox pipeline)               | Fog Attack ( $\epsilon = 512$ , blackbox pipeline)                | Snow Attack ( $\epsilon = 0.25$ , blackbox pipeline)              | Snow Attack ( $\epsilon = 0.75$ , blackbox pipeline)               |
| 41                                                                 | 42                                                               | 43                                                                | 44                                                                | 45                                                                 |
| Jpeg Attack ( $\epsilon = 0.125$ , blackbox pipeline)              | Jpeg Attack ( $\epsilon = 0.25$ , blackbox pipeline)             | Gabor Attack ( $\epsilon = 20$ , blackbox pipeline)               | Gabor Attack ( $\epsilon = 40$ , blackbox pipeline)               | Elastic Attack ( $\epsilon = 1.5$ , blackbox pipeline)             |
| 46                                                                 |                                                                  |                                                                   |                                                                   |                                                                    |
| Elastic Attack ( $\epsilon = 2.0$ , blackbox pipeline)             |                                                                  |                                                                   |                                                                   |                                                                    |

10%) of our standard GTSRB-CNN model. Thus, we only present the evaluation results of our models against the three most successful corruption — Fog, Contrast, Brightness. (Note that, here we use Fog corruption which is similar to the Fog attack in unforeseen attacks. However, they are different in that the Fog corruption here is not adversarially generated like that in Fog attack.)

Thus, based on different attack/corruption methods and attack settings, in total, we have 46 different attacks/corruptions. In Figure 2(b)(c), we use id numbers 1 ~ 46 to denote all the attacks we evaluate on, and we present the correspondence between id numbers and attacks in Table 5. Moreover, besides the two representative baselines presented in the main body, we present the complete robustness improvement results under the 46 types of attacks/corruptions for all baselines in Figure 3.

### B.3. Implementation Details of KEMLP Pipeline for Traffic Sign Identification

To implement a nontrivial KEMLP pipeline for traffic sign identification, we need to design informative knowledge rules, connecting useful sensory information to each type of traffic sign. The full GTSRB dataset contains 43 types of signs, thus it requires a large amount of fine-grained sensory information and corresponding knowledge rules to distinguish between different signs, which requires a heavy engineering workload. Since the main purpose of this work is to illustrate the knowledge enhancement methodology rather than engineering practice, alternatively, we only consider a 12-class subset (as shown in Figure 4) in our experiment, where the selected signs have diverse appearance and high frequencies.

For detailed KEMLP pipeline implementation, we consider two orthogonal domains — logic domain and sensing domain, respectively.

**In the logic domain**, based on the specific tasks we need to deal with, we design a set of knowledge rules, which determine the basic logical structure of the predefined reasoning model. Specifically, for our task of traffic sign identification on the 12-class dataset, in total, we have designed 12 pieces of permissive knowledge rules and 12 pieces of preventative knowledge rules for the selected 12 types of signs. Each type of sign shares exactly one permissive knowledge rule and one preventative knowledge rule, respectively.

In our design, we take *border patterns* and *sign contents* of the traffic signs as the sensory information to construct knowledge rules. As shown in Figure 5, based on the border pattern, we can always construct a preventative knowledge rule for each sign based on its border in the form as *if it is a stop sign, it should be of the shape of octagon*. In our 12-class set, since there are six types of signs (“Stop”, “Priority Road”, “Construction Area”, “Yield”, “Do Not Enter”, “End of Previous Limitation”) sharing the unique border pattern, we also design an permissive rule for each of the six classes based on their borders, e.g. *if the sign is of the shape of octagon, it must be a stop sign*. Then, for the rest of the six types (“No Vehicles”, “Speed Limit 50”, “Speed Limit 20”, “Speed Limit 120”, “Keep Right”, “Turn Left Ahead”), whose borders can not uniquely determine their identity, we use their unique sign content to design permissive rules for them. Specifically, we define the content pattern *Blank Circle*, *Digits-20*, *Digits-50*, *Digits-120*, *Arrow-Right-Down*, *Arrow-Left-Ahead* to distinguish between these signs. We present the permissive relations in Figure 6.

**In the sensing domain**, the principal task is to design a set of reliable auxiliary models to identify those sensory information required by the knowledge rules defined in the logic domain. For traffic sign identification, we adopt a non-neural pre-

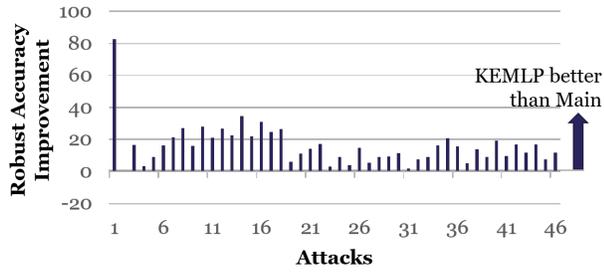

(a) Baseline: KEMLP over GTSRB-CNN

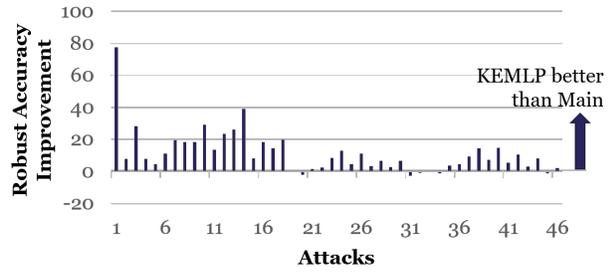

(b) Baseline: KEMLP over AdvTrain ( $\epsilon = 4$ )

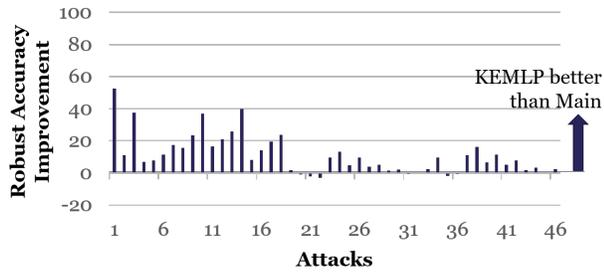

(c) Baseline: KEMLP over AdvTrain ( $\epsilon = 8$ )

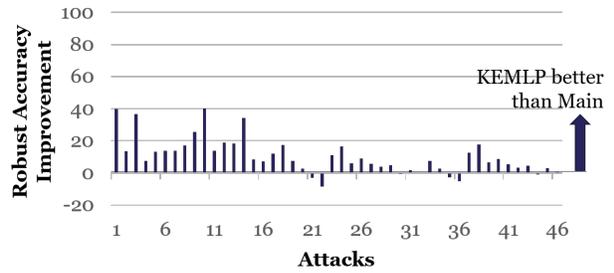

(d) Baseline: KEMLP over AdvTrain ( $\epsilon = 16$ )

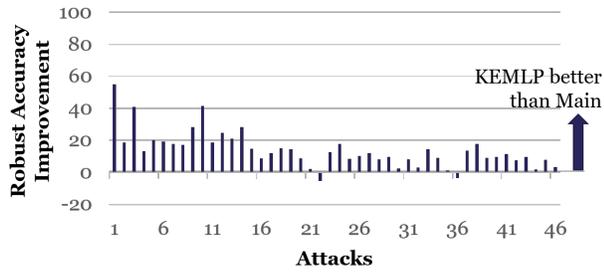

(e) Baseline: KEMLP over AdvTrain ( $\epsilon = 32$ )

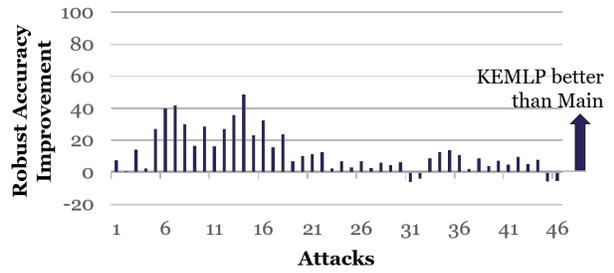

(f) Baseline: KEMLP over DOA (5x5)

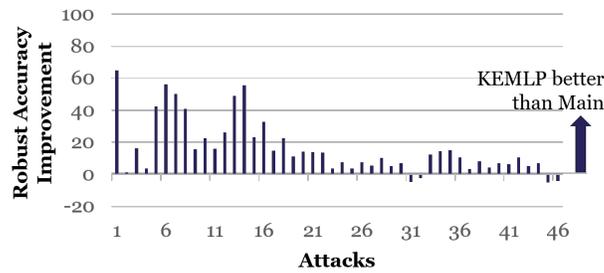

(g) Baseline: KEMLP over DOA (7x7)

Figure 3. Improvement of robustness accuracy after being enhanced by KEMLP. ( $\alpha = 0.5$ )

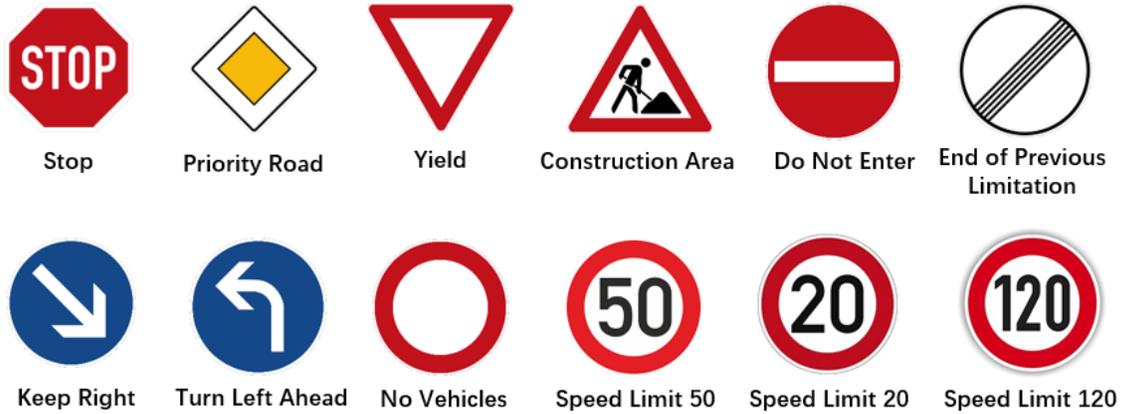

Figure 4. The selected 12 types of signs from the full GTSRB.

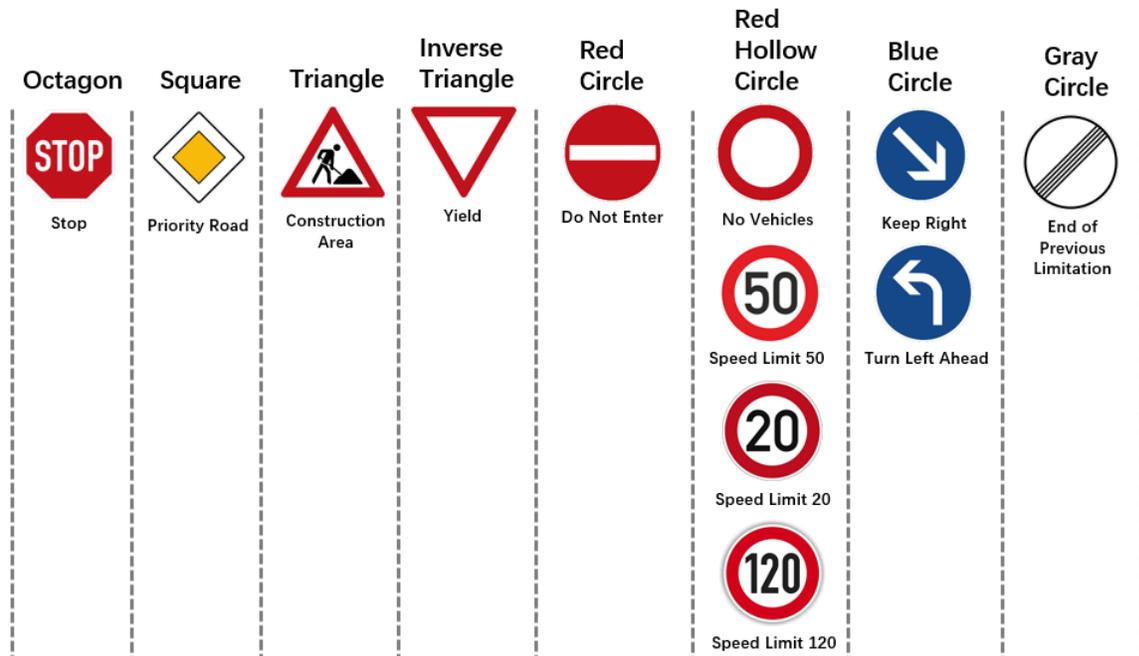

Figure 5. Border patterns of the selected signs.

processing plus neural identification workflow to identify the border and content of each type. Specifically, to identify the border type (e.g. shape and color), we first use GrabCut (Rother et al., 2004) to get the mask of the sign and then discard all pixels of sign content and background, only retaining the border pixels, and finally a binary CNN classifier is used to make the statistical prediction (e.g. predict whether the shape is octagon only based on the border pixels). For sign content, similarly, we first use GrabCut to filter out all irrelevant pixels except for the sign content, and then the edge operator will extract the contour of the content, finally CNN models are applied to recognize specific features like digits, arrows and characters. In Figure 7, we provide an overview of the workflow of our implemented auxiliary models.

In total, in our KEMLP pipeline, we implement 19 submodels — 1) One end-to-end GTSRB-CNN classifier (Eykholt et al., 2018) as the main task model; 2) 8 binary preventative models for all 8 types of borders; 3) 6 binary permissive models for the 6 border types, each of which is shared only by a unique class of sign; 4) 3 binary permissive models based on edge map of sign content (*Blank Circle*, *Arrow-Right-Down*, *Arrow-Left-Ahead*); 5) A single permissive model for digit recognition, which is used to identify *Digits-20*, *Digits-50*, *Digits-120*. All of the 17 binary classification neural models adopt the same

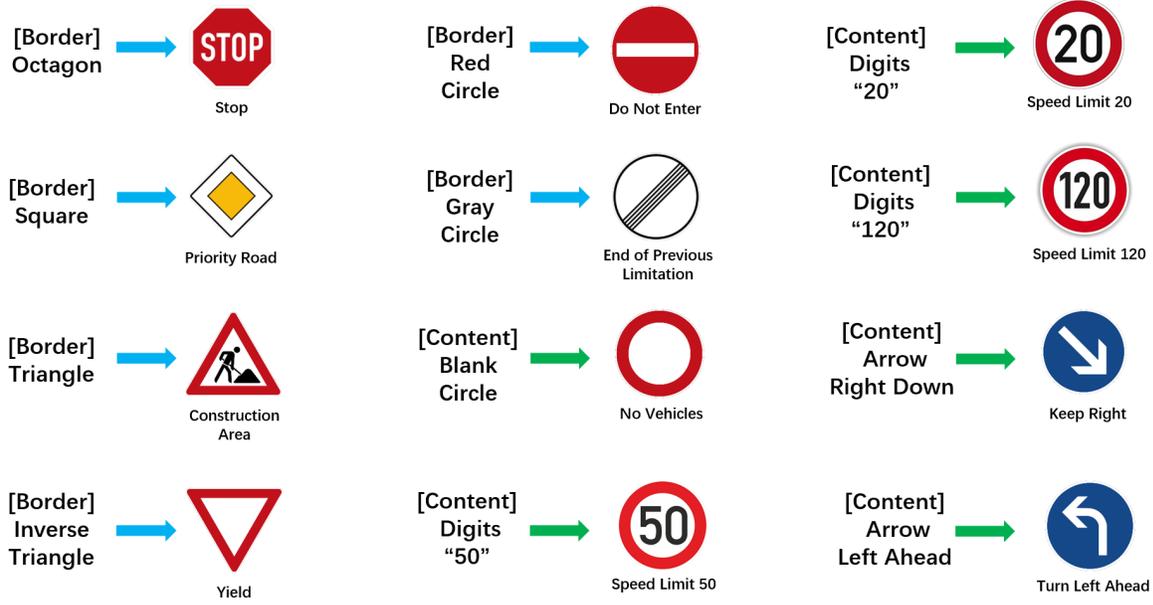

Figure 6. permissive relations for each sign.

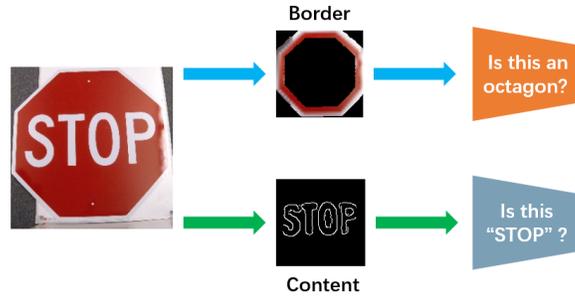

Figure 7. Overview: workflow of the auxiliary models.

backbone architecture in GTSRB-CNN and the rest digit recognition model adopts the architecture proposed in Goodfellow et al. (2013).

**Training Details.** To make our KEMLP pipeline function normally as the way we expect, next, we consider the training issues of the overall model.

Given the definition of permissive and preventative models, ideally, the permissive models should have low false rate and nontrivial truth rate, while the preventative models should have high truth rate and nontrivial false rate. These conditions are very critical for auxiliary models to bring accuracy improvement into the KEMLP pipeline. We guarantee the conditions to hold by assigning biased weights to classification loss on positive samples and negative samples during the training stage. Specifically, we train all of our binary auxiliary models with the following loss function:

$$L(\mathcal{D}, f) = a\mathbb{E}_{x \sim \mathcal{D}^+} [CE(f(x), 1)] + b\mathbb{E}_{x \sim \mathcal{D}^-} [CE(f(x), 0)],$$

where  $\mathcal{D} = \{D^+, D^-\}$  is the dataset,  $D^+$  is the subset containing positive samples,  $D^-$  is the subset containing negative samples,  $f$  is the classifier and  $CE$  is the crossentropy loss. For permissive model, we set  $a \ll b$ , so that low false rate will be encouraged at the cost of truth rate; while for preventative sensors, we set  $a \gg b$ , then we can expect a high truth rate at the cost of some false rate.

Besides the performance of each individual model, we also need to get proper weights for the reasoning graphical model in

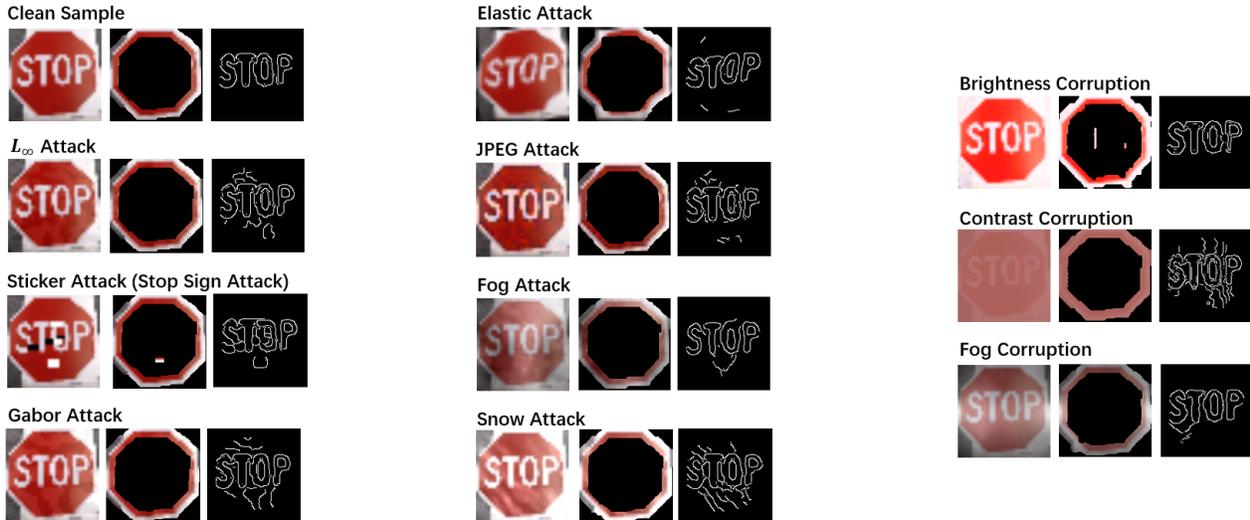

Figure 8. Visualization of adversarial examples and corrupted samples.

the KEMLP pipeline. Empirically, in our traffic sign identification task, since the end-to-end main task model has almost perfect accuracy on clean data, directly training on clean data will always give the main task model a dominant weight, leading to a trivial pipeline model. Thus, during training, we augment the training set with artificial adversarial samples, where the sensing signal from the main task model is randomly flipped. As a result, during training, to make correct predictions on these artificial adversarial samples, the optimizer must also assign nontrivial weights to other auxiliary models. We call the ratio of such artificial adversarial samples in the training set the “adversarial ratio” in our context, indicating prior belief on the balance between benign and adversarial distributions, and use  $\alpha$  to denote it. In our evaluation, we test different settings of  $\alpha \in \{0, 0.1, 0.2, 0.3, 0.4, 0.5, 0.6, 0.7, 0.8, 0.9, 1.0\}$  and report the best results in Table 2,6,7,1,3,8,9,4. In particular, we use  $\alpha = 0.8$  in Table 2,3,  $\alpha = 0.2$  in Table 6,7,8,9,4 and  $\alpha = 0.4$  in Table 1. Moreover, we also present the performance of KEMLP against different attacks with a fixed  $\alpha = 0.5$  in Figure 3.

For all the neural models, we use the standard Stochastic Gradient Descent Optimizer for training. The optimizer adopts a learning rate of  $10^{-2}$ , momentum of 0.9 and weight decay of  $10^{-4}$ . In all the training cases, we use 50000 training iterations with a batch size of 200 for each random training iteration. To train the weights of the graphical model in the pipeline, we perform Maximum Likelihood Estimate (MLE) with the standard gradient descent algorithm, and we use a learning rate of  $10^{-1}$  and run 4000 training iterations with a batch size of 50 for each random iterations.

#### B.4. Visualization of Adversarial Examples and Corrupted Samples

In Figure 8, we provide a visualization of the generated adversarial examples (corrupted samples) that are used for robustness evaluation in our work. For each type of attack (corruption), we present the generated example (the first image in each block), the extracted border (the second image in each block), and the sign content (the third image in each block) from the sample.

As we can see, although the adversarial examples can easily fool an end-to-end neural network based main task model, the non-neural GrabCut algorithm and edge operator can still correctly extract the border and sign content from them. This allows other auxiliary models help to rectify the mistakes made by the main task model.

#### B.5. Additional Experiment Results

In the main text, we have presented our evaluation results under the setting of whitebox sensor attack. In this subsection, we present the evaluation results of  $\mathcal{L}_\infty$  attack and unforeseen attacks under blackbox sensor and blackbox pipeline attack settings. Specifically, we present the two blackbox results for  $\mathcal{L}_\infty$  attack in table 6 and table 7, and accordingly the two blackbox results for unforeseen attacks in table 8 and table 9.

Table 6. Adversarial accuracy under black-box sensor  $\mathcal{L}_\infty$  attack,  $\alpha = 0.2$  (Accuracy %)

|                              |       | $\epsilon = 0$ | $\epsilon = 4$      | $\epsilon = 8$      | $\epsilon = 16$     | $\epsilon = 32$ |
|------------------------------|-------|----------------|---------------------|---------------------|---------------------|-----------------|
| GTSRB-CNN                    | Main  | <b>99.38</b>   | 85.16               | 67.98               | 47.56               | 25.69           |
|                              | KEMLP | 98.28(-1.10)   | 91.36(+6.20)        | 79.53(+11.55)       | 61.21(+13.65)       | 41.85(+16.16)   |
| AdvTrain ( $\epsilon = 4$ )  | Main  | 97.94          | 94.88               | 90.23               | 72.99               | 50.75           |
|                              | KEMLP | 97.89(-0.05)   | <b>95.88(+1.00)</b> | <b>90.66(+0.43)</b> | 77.01(+4.02)        | 55.56(+4.81)    |
| AdvTrain ( $\epsilon = 8$ )  | Main  | 93.72          | 91.49               | 89.02               | 80.56               | 64.76           |
|                              | KEMLP | 96.79(+3.07)   | 94.29(+2.80)        | 90.23(+1.21)        | <b>81.40(+0.84)</b> | 65.92(+1.16)    |
| AdvTrain ( $\epsilon = 16$ ) | Main  | 84.54          | 83.05               | 82.00               | 79.76               | <b>73.20</b>    |
|                              | KEMLP | 94.68(+10.14)  | 90.72(+7.67)        | 86.52(+4.52)        | 80.02(+0.26)        | 70.47(-2.73)    |
| AdvTrain ( $\epsilon = 32$ ) | Main  | 74.74          | 73.64               | 72.79               | 71.91               | 67.77           |
|                              | KEMLP | 91.46(+16.72)  | 86.60(+12.96)       | 81.66(+8.87)        | 75.69(+3.78)        | 66.77(-1.00)    |
| DOA (5x5)                    | Main  | 97.43          | 84.93               | 70.70               | 52.44               | 33.15           |
|                              | KEMLP | 97.45(+0.02)   | 92.21(+7.28)        | 81.56(+10.86)       | 64.07(+11.63)       | 45.70(+12.55)   |
| DOA (7x7)                    | Main  | 97.27          | 79.48               | 65.77               | 48.71               | 30.99           |
|                              | KEMLP | 97.22(-0.05)   | 90.56(+11.08)       | 80.20(+14.43)       | 62.55(+13.84)       | 44.24(+13.25)   |

 Table 7. Adversarial accuracy under black-box pipeline  $\mathcal{L}_\infty$  attack,  $\alpha = 0.2$  (Accuracy %)

|                              |       | $\epsilon = 0$ | $\epsilon = 4$      | $\epsilon = 8$      | $\epsilon = 16$     | $\epsilon = 32$ |
|------------------------------|-------|----------------|---------------------|---------------------|---------------------|-----------------|
| GTSRB-CNN                    | Main  | <b>99.38</b>   | 81.17               | 60.52               | 37.60               | 24.28           |
|                              | KEMLP | 98.28(-1.10)   | 89.76(+8.59)        | 76.18(+15.66)       | 56.07(+18.47)       | 37.50(+13.22)   |
| AdvTrain ( $\epsilon = 4$ )  | Main  | 97.94          | 94.42               | 88.32               | 66.08               | 46.60           |
|                              | KEMLP | 97.89(-0.05)   | <b>95.88(+1.46)</b> | <b>89.61(+1.29)</b> | 71.91(+5.83)        | 51.57(+4.97)    |
| AdvTrain ( $\epsilon = 8$ )  | Main  | 93.72          | 90.72               | 87.11               | 75.49               | 58.64           |
|                              | KEMLP | 96.79(+3.07)   | 94.16(+3.44)        | 89.40(+2.29)        | 77.31(+1.82)        | 60.26(+1.62)    |
| AdvTrain ( $\epsilon = 16$ ) | Main  | 84.54          | 82.87               | 81.46               | 77.13               | <b>70.09</b>    |
|                              | KEMLP | 94.68(+10.14)  | 90.87(+8.00)        | 86.37(+4.91)        | <b>78.06(+0.93)</b> | 68.44(-1.65)    |
| AdvTrain ( $\epsilon = 32$ ) | Main  | 74.74          | 73.66               | 72.35               | 70.16               | 66.08           |
|                              | KEMLP | 91.46(+16.72)  | 86.70(+13.04)       | 81.74(+9.39)        | 73.46(+3.30)        | 65.23(-0.85)    |
| DOA (5x5)                    | Main  | 97.43          | 81.94               | 66.13               | 48.28               | 33.26           |
|                              | KEMLP | 97.45(+0.02)   | 91.13(+9.19)        | 78.88(+12.75)       | 61.42(+13.14)       | 42.36(+9.10)    |
| DOA (7x7)                    | Main  | 97.27          | 77.85               | 63.68               | 46.55               | 31.79           |
|                              | KEMLP | 97.22(-0.05)   | 89.84(+11.99)       | 77.78(+14.10)       | 60.39(+13.84)       | 40.90(+9.11)    |

As shown, similar trends in whitebox sensor attack setting can also be observed in these two blackbox attack settings, which indicates that the robustness is not just coming from gradient masking (Carlini and Wagner, 2017b; Athalye et al., 2018).

## B.6. Conceptual Discussion on KEMLP

In the main body of this work, we have both empirically and theoretically justified our intuition — *With the incorporation of human knowledge, in KEMLP, weak (in terms of accuracy) but robust sensors (or auxiliary models named in the main text) can assist a SOTA NN to enhance its robustness.*

In general, we expect that KEMLP can be more generic — it is not necessarily constructed by exactly one main task model and several auxiliary models that assist the main task model, instead, it can incorporate any kind of **sensors** (sub-models) and **knowledge rules** to form a sensing-reasoning style pipeline, which first captures observational information from the input via its sensors and then makes decision via reasoning based on knowledge rules and observational information extracted by the sensors. As a supplement, in this section, we give out a conceptual discussion on this generic version, presenting some additional promising opportunities it can provide for robust machine learning:

1. *The decision process of KEMLP framework allows the incorporation of human knowledge, which helps to improve the robustness of machine learning systems in a fundamental way.*

Recently, Ilyas et al. (2019) point out that the adversarial vulnerability can be directly attributed to the presence of non-robust features. This feature perspective indicates that adversarial vulnerability may be a human-centric phenomenon — in some sense, as long as a classifier relies on some human imperceptible/incomprehensible features, an adversarial example may be constructed via controlling these features without affecting human’s recognition. However, since we usually train a classifier to solely maximize distributional accuracy, the learnt model tend to use any available signal to do so, even those that look incomprehensible to humans — after all, the presence of “a tail” or “ears” is no more natural to a model than any other equally predictive feature.

Thus, from a pessimistic view, the problem of adversarial vulnerability of machine learning systems may never

**Table 8. Adversarial accuracy under black-box sensor unforeseen attack,  $\alpha = 0.2$  (Accuracy %)**

|                              |       | clean         | fog-256              | fog-512              | snow-0.25            | snow-0.75            | jpeg-0.125           | jpeg-0.25            | gabor-20             | gabor-40             | elastic-1.5          | elastic-2.0          |
|------------------------------|-------|---------------|----------------------|----------------------|----------------------|----------------------|----------------------|----------------------|----------------------|----------------------|----------------------|----------------------|
| GTSRB-CNN                    | Main  | <b>99.38</b>  | 77.55                | 59.93                | 78.50                | 45.34                | 83.10                | 65.90                | 75.36                | 59.26                | 77.16                | 57.64                |
|                              | KEMLP | 98.28(-1.10)  | 84.03(+6.48)         | 68.54(+8.61)         | 83.08(+4.58)         | 57.77(+12.43)        | 88.97(+5.87)         | 74.90(+9.00)         | 84.88(+9.52)         | 70.04(+10.78)        | 82.10(+4.94)         | 66.69(+9.05)         |
| AdvTrain ( $\epsilon = 4$ )  | Main  | 97.94         | 70.68                | 54.06                | 77.70                | 49.67                | 87.45                | 72.84                | 88.14                | 68.21                | 83.38                | 70.09                |
|                              | KEMLP | 97.89(-0.05)  | 79.37(+8.69)         | 64.38(+10.32)        | 82.38(+4.68)         | 59.21(+9.54)         | <b>91.80</b> (+4.35) | 80.09(+7.25)         | 91.51(+3.37)         | 75.05(+6.84)         | 84.80(+1.42)         | 73.12(+3.03)         |
| AdvTrain ( $\epsilon = 8$ )  | Main  | 93.72         | 67.70                | 53.73                | 76.13                | 51.75                | 86.27                | 76.75                | 89.25                | 76.47                | 80.71                | 67.85                |
|                              | KEMLP | 96.79(+3.07)  | 76.70(+9.00)         | 64.97(+11.24)        | 80.99(+4.86)         | 60.39(+8.64)         | 91.02(+4.75)         | 82.54(+5.79)         | <b>91.56</b> (+2.31) | 79.45(+2.98)         | 83.26(+2.55)         | 71.37(+3.52)         |
| AdvTrain ( $\epsilon = 16$ ) | Main  | 84.54         | 66.44                | 49.64                | 75.15                | 52.73                | 81.58                | 77.78                | 83.90                | 82.48                | 76.23                | 68.26                |
|                              | KEMLP | 94.68(+10.14) | 77.11(+10.67)        | 63.84(+14.20)        | 81.58(+6.43)         | 60.73(+8.00)         | 87.68(+6.10)         | <b>82.77</b> (+4.99) | 89.27(+5.37)         | <b>83.44</b> (+0.96) | 81.07(+4.84)         | 71.55(+3.29)         |
| AdvTrain ( $\epsilon = 32$ ) | Main  | 74.74         | 65.82                | 50.18                | 71.97                | 52.37                | 72.61                | 71.09                | 76.26                | 77.16                | 68.03                | 64.38                |
|                              | KEMLP | 91.46(+16.72) | 77.62(+11.80)        | 64.56(+14.38)        | 79.60(+7.63)         | 61.09(+8.72)         | 83.85(+11.24)        | 79.30(+8.21)         | 85.60(+9.34)         | 80.09(+2.93)         | 77.67(+9.64)         | 70.81(+6.43)         |
| DOA (5x5)                    | Main  | 97.43         | 78.24                | 62.32                | 79.55                | 56.69                | 86.55                | 71.32                | 82.23                | 67.28                | 87.96                | 75.75                |
|                              | KEMLP | 97.41(-0.02)  | <b>84.26</b> (+6.02) | <b>69.08</b> (+6.76) | 83.36(+3.81)         | <b>62.58</b> (+5.89) | 90.41(+3.86)         | 77.98(+6.66)         | 87.06(+4.83)         | 73.69(+6.41)         | <b>86.09</b> (-1.87) | <b>75.90</b> (+0.15) |
| DOA (7x7)                    | Main  | 97.27         | 76.34                | 61.32                | 79.30                | 55.94                | 83.20                | 66.10                | 82.25                | 67.54                | 86.73                | 73.77                |
|                              | KEMLP | 97.22(-0.05)  | 82.74(+6.40)         | 68.52(+7.20)         | <b>83.74</b> (+4.44) | 62.47(+6.53)         | 89.04(+5.84)         | 76.44(+10.34)        | 87.60(+5.35)         | 74.51(+6.97)         | 85.91(-0.82)         | 75.49(+1.72)         |

**Table 9. Adversarial accuracy under black-box pipeline unforeseen attack,  $\alpha = 0.2$  (Accuracy %)**

|                              |       | clean         | fog-256              | fog-512              | snow-0.25            | snow-0.75            | jpeg-0.125           | jpeg-0.25            | gabor-20             | gabor-40             | elastic-1.5  | elastic-2.0   |
|------------------------------|-------|---------------|----------------------|----------------------|----------------------|----------------------|----------------------|----------------------|----------------------|----------------------|--------------|---------------|
| GTSRB-CNN                    | Main  | <b>99.38</b>  | 71.17                | 49.13                | 70.73                | 36.45                | 75.44                | 51.98                | 72.61                | 53.47                | 70.88        | 54.53         |
|                              | KEMLP | 98.28(-1.10)  | 78.96(+7.79)         | 60.65(+11.52)        | 80.02(+9.29)         | 52.16(+15.71)        | 85.31(+9.87)         | 67.64(+15.66)        | 84.13(+11.52)        | 69.24(+15.77)        | 80.66(+9.78) | 67.80(+13.27) |
| AdvTrain ( $\epsilon = 4$ )  | Main  | 97.94         | 66.23                | 47.33                | 73.46                | 42.10                | 84.23                | 65.07                | 87.29                | 66.95                | 82.10        | 68.80         |
|                              | KEMLP | 97.89(-0.05)  | 74.97(+8.74)         | 58.62(+11.29)        | 80.63(+7.17)         | 54.09(+11.99)        | <b>90.84</b> (+6.61) | 76.00(+10.93)        | 90.61(+3.32)         | 74.77(+7.82)         | 84.85(+2.75) | 74.95(+6.15)  |
| AdvTrain ( $\epsilon = 8$ )  | Main  | 93.72         | 63.14                | 45.14                | 72.87                | 46.66                | 84.59                | 71.35                | 88.86                | 73.74                | 80.30        | 67.88         |
|                              | KEMLP | 96.79(+3.07)  | 72.89(+9.75)         | 58.02(+12.88)        | 79.73(+6.86)         | 55.86(+9.20)         | 90.59(+6.00)         | 80.02(+8.67)         | <b>90.92</b> (+2.06) | 77.93(+4.19)         | 83.80(+3.50) | 73.77(+5.89)  |
| AdvTrain ( $\epsilon = 16$ ) | Main  | 84.54         | 62.32                | 42.98                | 73.23                | 50.08                | 80.97                | 76.26                | 83.51                | 81.22                | 75.80        | 68.75         |
|                              | KEMLP | 94.68(+10.14) | 73.48(+11.16)        | 58.18(+15.20)        | 80.45(+7.22)         | 57.54(+7.46)         | 86.99(+6.02)         | <b>80.92</b> (+4.66) | 88.30(+4.79)         | <b>82.23</b> (+1.01) | 81.71(+5.91) | 72.69(+3.94)  |
| AdvTrain ( $\epsilon = 32$ ) | Main  | 74.74         | 61.86                | 45.01                | 70.47                | 50.57                | 72.38                | 69.70                | 76.16                | 76.39                | 68.65        | 64.99         |
|                              | KEMLP | 91.46(+16.72) | 73.33(+11.47)        | 58.49(+13.48)        | 78.94(+8.47)         | 58.67(+8.10)         | 83.33(+10.95)        | 77.42(+7.72)         | 84.95(+8.79)         | 79.09(+2.70)         | 78.37(+9.72) | 71.45(+6.46)  |
| DOA (5x5)                    | Main  | 97.43         | 75.01                | 56.97                | 77.67                | 53.14                | 83.15                | 63.79                | 82.07                | 65.77                | <b>88.17</b> | <b>78.88</b>  |
|                              | KEMLP | 97.41(-0.02)  | <b>80.40</b> (+5.39) | <b>64.40</b> (+7.43) | 82.28(+4.61)         | 59.52(+6.38)         | 88.89(+5.74)         | 73.69(+9.90)         | 87.04(+4.97)         | 73.43(+7.66)         | 86.99(-1.18) | 77.88(-1.00)  |
| DOA (7x7)                    | Main  | 97.27         | 73.97                | 57.05                | 77.21                | 53.55                | 81.40                | 62.68                | 82.15                | 67.28                | 87.42        | 78.27         |
|                              | KEMLP | 97.22(-0.05)  | 80.04(+6.07)         | 64.17(+7.12)         | <b>82.46</b> (+5.25) | <b>59.75</b> (+6.20) | 88.30(+6.90)         | 73.48(+10.80)        | 87.09(+4.94)         | 73.95(+6.67)         | 86.42(-1.00) | 78.58(+0.31)  |

be fundamentally solved via just training-level techniques like adversarial training (Madry et al., 2017) or purely mathematical techniques like randomized smoothing (Cohen et al., 2019). After all, if the robustness problem is human-centric, the predictive features and decision mechanisms learnt by purely supervised learning algorithms may never be well aligned with human’s sense. Even a model is robust to certain  $\mathcal{L}_p$  attack via these robust machine learning techniques, there is deformation, snow, fog and any other kind of unforeseen adversarial attack (Kang et al., 2019), as long as these perturbations can not affect human’s recognition in some sense.

From this perspective, to fundamentally solve the problem of adversarial vulnerability, which seems to be a human-centric phenomenon, human knowledge should play a critical role as a guidance for learning features and decision mechanisms.

Our KEMLP framework is one such attempt to adopt knowledge for robust machine learning. Different from end-to-end neural network models, which complete the full procedure of sensory information process and decision making all in a single uninterpretable black box, the KEMLP framework resolves a decision problem into two separate processes — 1) sensory information capturing (sensing domain) during which a set of observations with clear semantic meanings are obtained; 2) decision making (logic domain) during which the final decision is made via logical reasoning, based on the observations from the first process and the decision rules determined by human knowledge.

Such design brings about two fundamental benefits:

- The sensory features extracted in the sensing domain of KEMLP are totally in a human understandable format with clear semantic meaning, and the relations between features and candidate decisions in the logical domain also have clear human knowledge as the basis. For instance, in our KEMLP implementation for traffic sign identification, the extracted sensory features output by the sensors are all boolean variables, representing meaningful concepts, e.g. *whether the given sign is of the shape of octagon*, *whether the content on the sign are the characters “S”, “T”, “O”, “P”*, and the decision rules like *“Stop sign must be of the shape of octagon”* have clear logical basis. As a result, the problem of non-robust features (Ilyas et al., 2019; Tsipras et al., 2019) no longer exists in the logic domain of KEMLP framework, as long as the knowledge rules themselves are reasonable.
- In KEMLP framework, the adversarial vulnerability is strictly restricted to the sensing domain — to build up a robust pipeline model, we only need to deal with the sensory errors (the mistakes made by sensors, given that the sensors may still be attacked). Specifically, if an adversarial example fools our KEMLP framework, we don’t need to consider the non-robust features or unreliable decision mechanism, instead, the only error we need to deal with is — one or several sensors have made wrong observations. Such errors are not as fundamental as what we have mentioned for end-to-end

neural network models, because they are technically tractable and can be well controlled. One concrete example is the case we present in the main body, where we have used a set of weak (in terms of accuracy) but robust sensors to build a good KEMLP instance.

**2. KEMLP framework provides a principled way to incorporate “weak” models.**

As we have mentioned, in KEMLP, the false negative errors of permissive sensors and false positive errors of preventative sensors will not mislead the decision process. Thus, to construct a KEMLP pipeline model, a binary sensor with high precision but relatively low recall can be used as permissive sensor, and a binary sensor with high recall but relatively low precision can be used as preventative sensor. Despite these sensors may be deemed as “weak” in terms of their accuracy, incorporating them will be very helpful to improve the performance of decision making. In particular, for robust machine learning, we are quite interested in taking use of some “weak” models with relatively lower accuracy but better adversarial robustness, to boost the the whole pipeline system. In the main text, we have already theoretically analyzed such robustness improvement.

In practice, such “weak” sensors are common. Take the traffic sign identification for example, earlier before the wide application of DNNs, elaborate algorithms (Kehtarnavaz et al., 1993; Miura et al., 2000) were already designed to handle this task. Although these sensors based on non-neural algorithms are weaker than the the state-of-the-art CNN models in terms of identification accuracy on clean data, they are more interpretable and less likely to be attacked by small adversarial noise. Moreover, in spite of relatively low accuracy, these “weak” sensors can usually be easily adapted to have high precision (at the cost of recall) or high recall (at the cost of precision), thus they can be incorporated into the KEMLP framework as permissive or preventative sensors. For instance, Kehtarnavaz et al. (1993) propose to identify a stop sign by detecting the eight lines of its octagon shape with Hough transform. For sure, because of the complex natural environment, this method (with a relatively high threshold to claim a straight line) often fails to correctly detect all of the 8 lines, which leads to a low recall (about 30% on GTSRB dataset according to our evaluation). However, it can achieve very high precision (about 95% on GTSRB dataset) because it’s hard to mistakenly detect an octagon when the threshold of claiming each straight line of the eight edges is high. Similarly, one can hardly use small adversarial noise to cheat Hough transform on the detection of all 8 edges, so its false positive error rate will still be low even against adversarial attacks. So, although this Hough transform based sensor is “weak”, it can be helpful as an permissive sensor in a KEMLP pipeline model.

Moreover, although recent study on robust machine learning have made some progress in improving adversarial robustness (Cohen et al., 2019; Madry et al., 2017), it is often at the cost of clean accuracy (Tsipras et al., 2019; Mohapatra et al., 2020). So, in some sense, all of the neural networks based sensors enhanced by adversarial defense techniques may also be deemed as one class of “weak” sensors, which share better robustness with weaker clean accuracy. Hence, we believe our KEMLP framework also provides an opportunity to incorporate those sensors enhanced by state-of-the-art defense techniques and helps to relieve the trade-off between robustness and accuracy. Actually, as we can see in Section 5, when we combine the adversarially trained main sensor and other auxiliary models, both the robust accuracy and clean accuracy are significantly improved compared with a single adversarially trained model.

**3. KEMLP framework subsumes ensemble defense and naturally leads to task-level diversity among the sub-models.**

In some sense, our KEMLP framework can be deemed as a more general framework that subsumes ensemble defense (Strauss et al., 2017; Liu et al., 2018; Kariyappa and Qureshi, 2019; Pang et al., 2019; Yang et al., 2020b), in that each sub-model in the ensemble can be directly modeled as a Type-I sensor (main task model) in KEMLP.

Much the same to ensemble defense, if all (or at least a majority of) sub-models (sensors) in a KEMLP pipeline can be simultaneously cheated, the final decision still can not be reliable. In the study of ensemble defense, to avoid such problems, different training strategies (Pang et al., 2019; Kariyappa and Qureshi, 2019; Yang et al., 2020b) are proposed, trying to diversify the sub-models during training stage, so that an adversarial example can only attack a minority of the sub-models.

Besides these training-level diversities studied in ensemble defense, the KEMLP framework, as a more general form, naturally provides us the opportunity to design diverse sub-models (sensors) in task level, because KEMLP framework allows the incorporation of sensors that are designed for very different tasks, e.g. *digit recognition*, *shape recognition*, etc. Intuitively, such task-level diversity naturally makes it harder to transfer an adversarial example to a majority of sensors, for example, even if the attackers have managed to fool the digit recognition sensors by perturbing the content of digits, the shape recognition of traffic sign border can’t be affected. We believe this new perspective of model diversity can also provide a possible solution for adversarial vulnerability in machine learning systems.

### B.7. Is KEMLP Robust against Adaptive Attacks?

Since the auxiliary models are implemented by non-neural pre-processing (edge operators and Grab-Cut) followed by neural network based classification, they are *not* end-to-end differentiable and thus the gradient-based adaptive attacks cannot be directly applied. We evaluated KEMLP with whitebox *adaptive* attack against 1) the main sensor (Tables 2,3) and 2) the distilled model of the whole pipeline (Tables 7,9) in paper. Note that we also evaluate KEMLP against the *model agnostic* common corruptions (Table 4), which demonstrates its effectiveness from another perspective.

We also evaluated our KEMLP model on SPSA attack (Uesato et al., 2018), which is a gradient-free black box attack. We conduct evaluation on a small test set with 50 stop-sign and 50 non-stop-sign samples. Our observations are as follows: 1) When we conduct SPSA attack directly on the main sensor, the accuracy of the main sensor can be reduced to near zero ( $\epsilon = 32$  for  $\mathcal{L}_\infty$  attack), while the same attack is not effective when it is conducted on the whole end-to-end pipeline. 2) Alternatively, we conduct the attack directly on the auxiliary sensors which are based on non-neural preprocessing and neural classification. Still, we find that even under strong perturbation ( $\epsilon = 32$ ), permissive sensors maintain low false rate (below 15%) and non-trivial truth rate (over 50%), while preventative sensors maintain high truth rate (over 80%) and relatively low false rate (below 30%).
